# Supplementary material for: Ab-initio tensile tests applied to BCC refractory alloys
Source: arXiv:2311.17713 ancillary file (2023-12-05)
Supplement: Supplementary file 1 [file supplementary-material.pdf]

# Supplementary Material
# *Ab-initio* tensile tests applied to BCC refractory alloys

Vishnu Raghuraman and Michael Widom
Department of Physics, Carnegie Mellon University, Pittsburgh, PA 15213

Saro San
NETL Support Contractor, Albany OR 97321

Michael C. Gao
National Energy Technology Laboratory, Albany OR 97321

# Computational Details

First-principles calculations are done using the program VASP[1]. We apply PAW potentials (Al, Cr_pv, Hf_pv, Mo_sv, Nb_sv, Re, Ru_pv, Si, Ta_pv, Ti_sv, V_sv, W_sv, Zr_sv) in the PBE generalized gradient approximation [2]

Energy cutoff of 350 eV is used with Methfessel-Paxton first order smearing [3] of width 0.2 eV.

128 atom unit cells (4x4x4 BCC supercells) are used with a k-point grid of 3x3x3.

Second and third order elastic constants are obtained by applying finite difference formulae to the energy and stress obtained from VASP calculation. This is implemented using simple python scripts and made available online [4]

[1] G. Kresse and D. Joubert, Phys. Rev. B 59, 1758 (1999).
[2] J. P. Perdew, K. Burke, and M. Ernzerhof, Phys. Rev. Lett. 77, 3865 (1996).
[3] M. Methfessel and A. T. Paxton, Phys. Rev. B 40, 3616 (1989).
[4] https://github.com/vishnu2709/ElasticToolkit.git

# Computational Details – INCAR file

```
  ISTART =      1    job   : 0-new  1-cont  2-samecut
NWRITE = 1
PREC = Acc
   NELM   =     40;
EDIFF = 1E-8
   NEDOS  = 1401
ALGO = Normal
LREAL = A
NSW = 40
   ISIF=3
   IBRION = 2
   POTIM = 0.25
   ISMEAR =     1;
   SIGMA  =    0.2;  broadening in eV -4-tet -1-fermi 0-gaus
LWAVE = F
LCHARG = F
#NPAR = 4
KPAR = 4
NSIM = 4
LPLANE = T
EDIFFG = -1E-04
ENCUT = 350
```

# Systems that show stacking faults

| | Stacking Fault Critical Strain | Stacking Fault Critical Stress (GPa) |
|---|---|---|
| $Mo_3Hf$ | 0.125 | 11.24 |
| $Mo_3Nb$ | 0.14 | 13.53 |
| $Mo_3Ta$ | 0.14 | 13.82 |
| $Mo_3Ti$ | 0.14 | 10.304 |
| $Mo_3V$ | 0.15 | 14.581 |
| $Mo_3W$ | 0.14 | 15.79 |
| $Mo_3Zr$ | 0.175 | 5.906 |
| $Nb_3Hf$ | 0.125 | 5.657 |
| $Nb_3Mo$ | 0.15 | 8.155 |
| $Nb_3Re$ | 0.15 | 10.196 |
| $Nb_3Ta$ | 0.15 | 6.3 |
| $Nb_3Ti$ | 0.15 | 4.914 |
| $Nb_3Zr$ | 0.15 | 5.233 |

# Systems that show slip

| | Slip Critical Strain | Slip Critical Stress (GPa) |
|---|---|---|
| $Mo_3Ti$ | 0.175 | 6.084 |
| $Mo_3Zr$ | 0.15 | 3.298 |
| $Nb_3Cr$ | 0.15 | 2.969 |
| $Nb_3Hf$ | 0.15 | 0.787 |
| $Nb_3V$ | 0.15 | 1.191 |
| $Nb_3W$ | 0.15 | 2.216 |

# Systems that show twinning

| | Twinning Critical Strain | Twinning Critical Stress (GPa) |
|---|---|---|
| $Mo_3Cr$ | 0.175 | 3.332 |
| $Mo_3Hf$ | 0.175 | 6.724 |
| $Mo_3Nb$ | 0.175 | 8.906 |
| $Mo_3Re$ | 0.2 | 2.123 |
| $Mo_3Ta$ | 0.175 | 10.171 |
| $Mo_3Ti$ | 0.2 | 2.99 |
| $Mo_3V$ | 0.175 | 2.096 |
| $Mo_3W$ | 0.2 | 4.404 |
| $Mo_3Zr$ | 0.175 | 5.906 |
| $Nb_3Cr$ | 0.2 | 2.422 |

| | Twinning Critical Strain | Twinning Critical Stress (GPa) |
|---|---|---|
| $Nb_3Hf$ | 0.2 | 0.844 |
| Nb3Mo | 0.15 | 8.155 |
| Nb3Re | 0.2 | 1.866 |
| Nb3Ru | 0.2 | 2.601 |
| Nb3Ta | 0.15 | 6.3 |
| Nb3Ti | 0.15 | 4.914 |
| Nb3V | 0.2 | 0.928 |
| Nb3W | 0.2 | 2.489 |
| Nb3Zr | 0.2 | 0.517 |

# Ductility parameters for Mo-based binaries

| | D | Pugh Ratio | Chi | DOS ($E_F$) |
|---|---|---|---|---|
| $Mo_3Al$ | 2.336 | 2.508385 | 0.5 | 0.66132177 |
| $Mo_3Cr$ | 2.018 | 2.166633 | 0.77272727 | 0.57482346 |
| $Mo_3Hf$ | 1.955 | 2.493321 | 0.6 | 0.67613256 |
| $Mo_3Nb$ | 1.875 | 2.393345 | 0.9047619 | 0.63882975 |
| $Mo_3Re$ | 2.265 | 2.487377 | 0.85714286 | 0.98181142 |
| $Mo_3Ru$ | 2.623 | 2.800377 | 0.51851852 | 0.84674198 |
| $Mo_3Si$ | 2.346 | 3.341964 | 0.42307692 | 0.64729672 |
| $Mo_3Ta$ | 1.893 | 2.236932 | 0.69230769 | 0.44067222 |
| $Mo_3Ti$ | 2.080 | 2.554702 | 0.8 | 0.75133368 |
| $Mo_3V$ | 1.966 | 2.349747 | 0.73076923 | 0.61325165 |
| $Mo_3W$ | 1.965 | 2.110352 | 0.625 | 0.49242169 |
| $Mo_3Zr$ | 1.946 | 2.511616 | 0.68181818 | 0.6420529 |

# Ductility parameters for Nb-based binaries

| | D | Pugh Ratio | Chi | DOS ($E_F$) |
|---|---|---|---|---|
| $Nb_3Al$ | 2.813 | 3.447546 | 0.52173913 | 0.87944659 |
| $Nb_3Cr$ | 2.666 | 5.862107 | 2.11111111 | 1.231375 |
| $Nb_3Hf$ | 3.091 | 4.35744 | 1.91666667 | 1.49523222 |
| $Nb_3Nb$ | 2.428 | 4.877899 | 1.53846154 | 1.1514691 |
| $Nb_3Re$ | 1.992 | 2.770588 | 0.48275862 | 0.63858369 |
| $Nb_3Ru$ | 2.470 | 2.757862 | 0.625 | 0.75115421 |
| $Nb_3Si$ | 2.194 | 5.863982 | 0.30769231 | 0.76817078 |
| $Nb_3Ta$ | 2.999 | 4.185845 | 3.71428571 | 1.41352844 |
| $Nb_3Ti$ | 3.250 | 4.865881 | 2.36363636 | 1.67424187 |
| $Nb_3V$ | 2.882 | 5.546459 | 3.42857143 | 1.58476116 |
| $Nb_3W$ | 2.431 | 4.605788 | 2.3 | 1.14789133 |
| $Nb_3Zr$ | 2.955 | 5.570297 | 3.66666667 | 1.59325964 |

# Ductility parameters for quaternaries

| | D | Pugh Ratio | Chi | DOS ($E_F$) |
|---|---|---|---|---|
| CrMoNbV | 2.265 | 3.151272 | 0.88235294 | 0.77461246 |
| CrMoNbW | 1.878 | 2.418349 | 0.69565217 | 0.58108082 |
| NbMoTiAl | 2.696 | 3.107548 | 0.52 | 0.92552305 |
| NbMoTiCr | 2.408 | 3.621738 | 1.2 | 1.1441718 |
| NbMoTiSi | 2.309 | 3.978651 | 0.7 | 0.8422502 |
| HfNbTiZr | 3.821 | 3.955516 | 0.46153846 | 1.41028167 |
| MoNbTaTi | 2.770 | 3.584298 | 1.23529412 | 1.31529847 |
| HfMoNbTi | 2.989 | 3.605767 | 1.05 | 1.31508118 |

# Ductility parameters for quaternaries

| | D | Pugh Ratio | Chi | DOS ($E_F$) |
|---|---|---|---|---|
| MoNbReTi | 2.180 | 2.582367 | 0.7826087 | 0.82135625 |
| MoNbRuTi | 2.266 | 2.644207 | 0.58333333 | 0.83784618 |
| MoNbTiV | 2.728 | 4.280731 | 1.76923077 | 1.44028613 |
| MoNbTiW | 2.367 | 3.050317 | 0.94736842 | 1.06665231 |
| MoNbTiZr | 2.883 | 3.955516 | 1.27777778 | 1.34858008 |
| MoNbTaW | 2.113 | 2.866163 | 0.875 | 0.68528811 |
| NbTaVW | 2.527 | 3.736125 | 2.07692308 | 1.22931471 |
| NbTaTiV | 3.253 | 4.565096 | 1 | 1.66783607 |

# Wallace tensor eigenvalues, Stress and Lattice distortion plots

NOTE

For eigenvalue plots, the curves obtained from tensile test are labelled “Nonlinear” and those obtained from third order elastic constants are labelled “Third Order”

# Mo-based binaries

Wallace tensor eigenvalues, stress, lattice distortion

# $Mo_3Al_1$

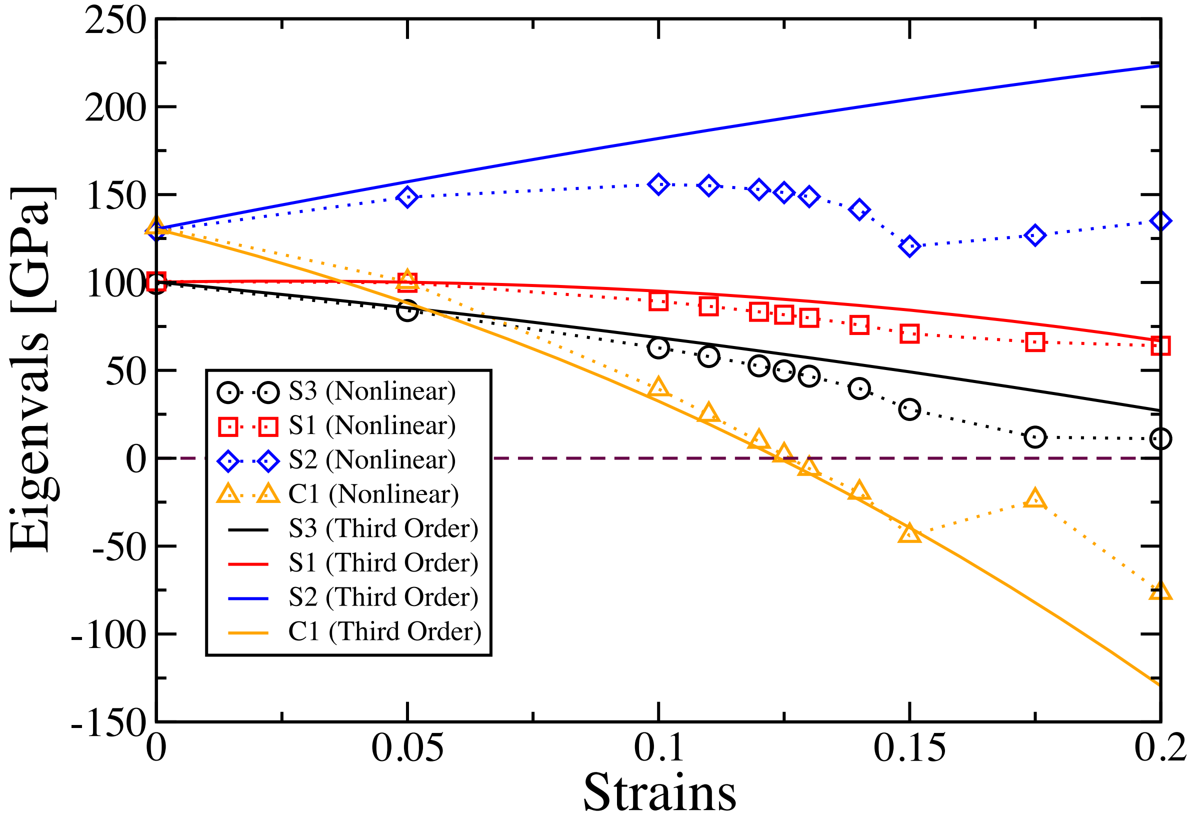

Eigenvals [GPa]
Strains
S3 (Nonlinear)
S1 (Nonlinear)
S2 (Nonlinear)
C1 (Nonlinear)
S3 (Third Order)
S1 (Third Order)
S2 (Third Order)
C1 (Third Order)
250
200
150
100
50
0
-50
-100
-150
0
0.05
0.1
0.15
0.2


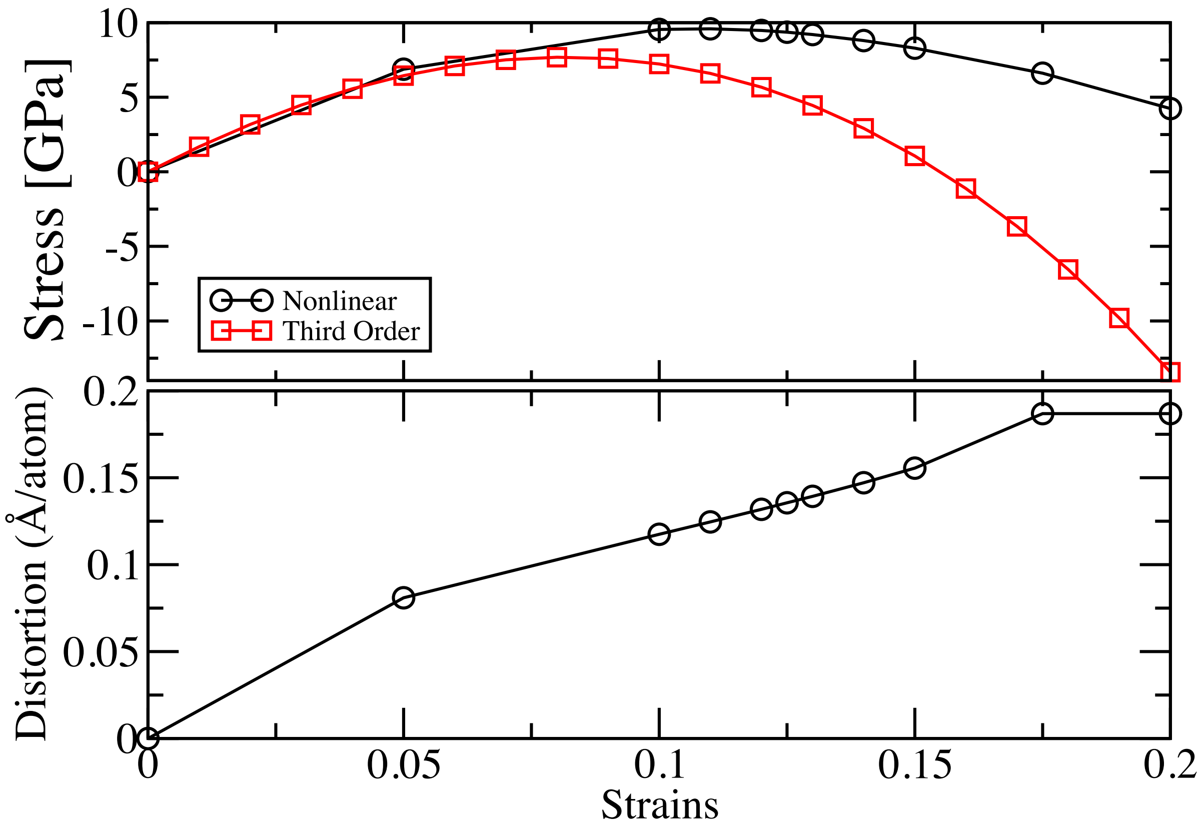

Stress [GPa]
Distortion (Å/atom)
Strains
Nonlinear
Third Order
10
5
0
-5
-10
0.2
0.15
0.1
0.05
0
0
0.05
0.1
0.15
0.2

# $Mo_3Cr_1$

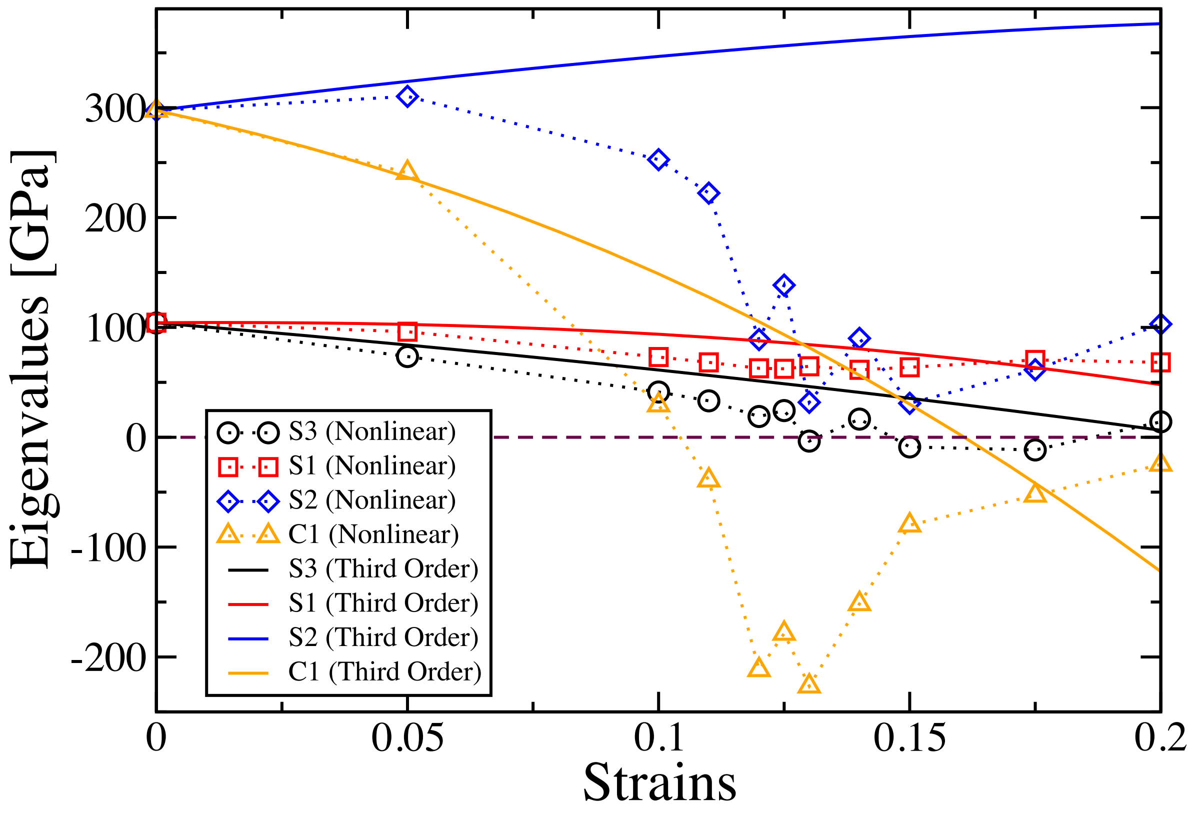
Eigenvalues [GPa]
Strains
S3 (Nonlinear)
S1 (Nonlinear)
S2 (Nonlinear)
C1 (Nonlinear)
S3 (Third Order)
S1 (Third Order)
S2 (Third Order)
C1 (Third Order)
300
200
100
0
-100
-200
0
0.05
0.1
0.15
0.2

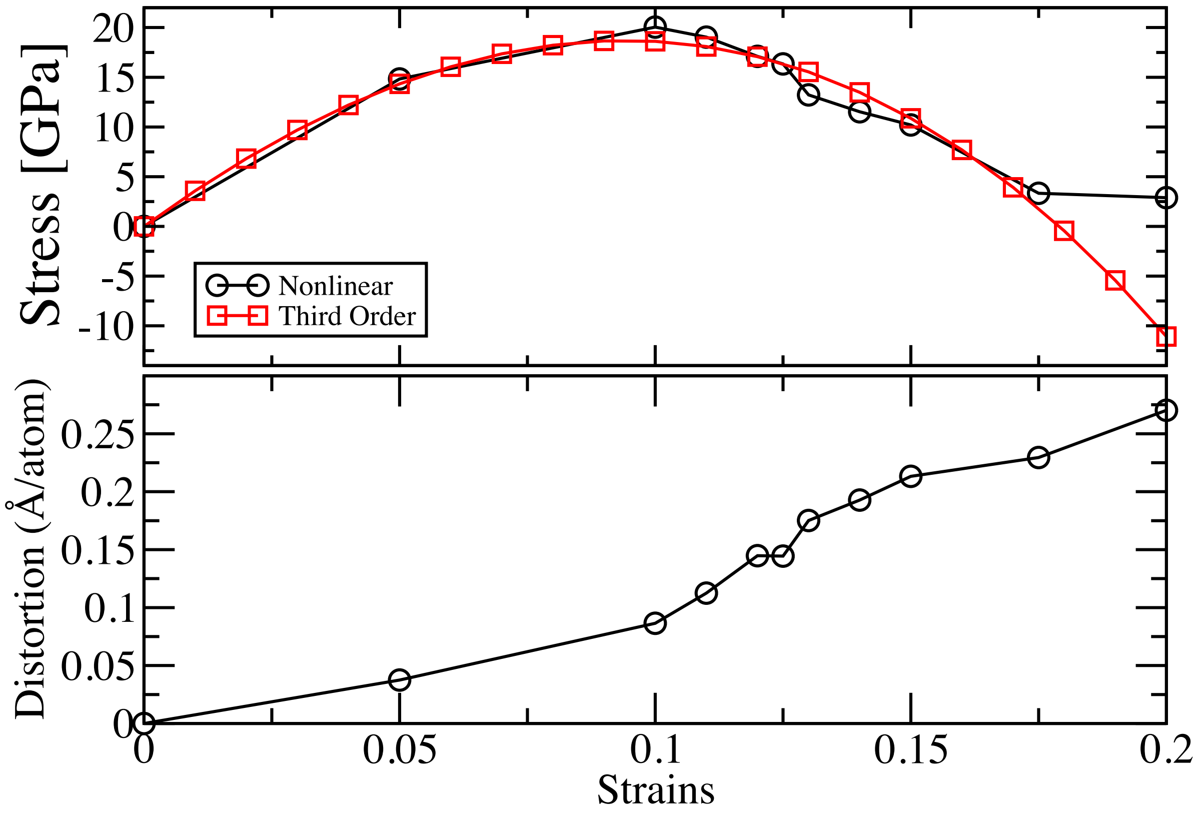
Stress [GPa]
Nonlinear
Third Order
Distortion (Å/atom)
Strains
20
15
10
5
0
-5
-10
0.25
0.2
0.15
0.1
0.05
0
0
0.05
0.1
0.15
0.2

# $Mo_3Hf_1$

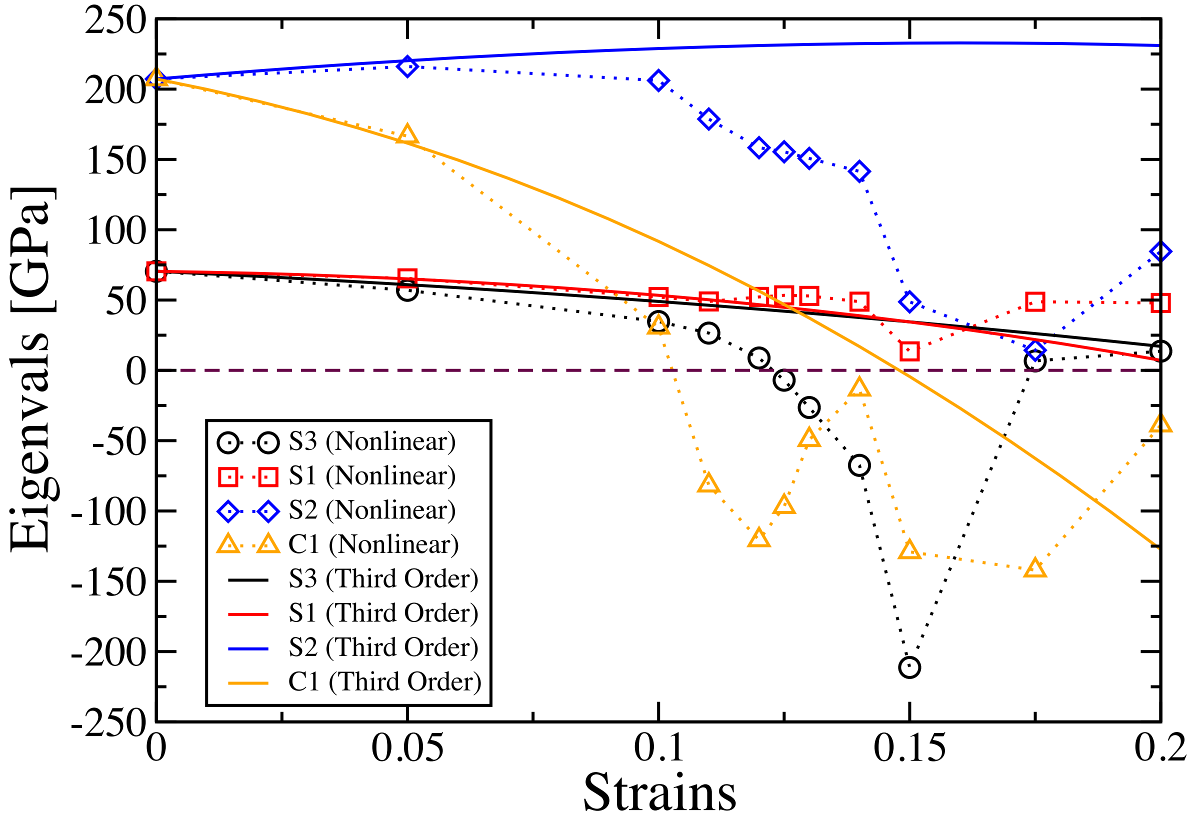
250
200
150
100
50
0
-50
-100
-150
-200
-250
Eigenvals [GPa]
0
0.05
0.1
0.15
0.2
Strains
S3 (Nonlinear)
S1 (Nonlinear)
S2 (Nonlinear)
C1 (Nonlinear)
S3 (Third Order)
S1 (Third Order)
S2 (Third Order)
C1 (Third Order)

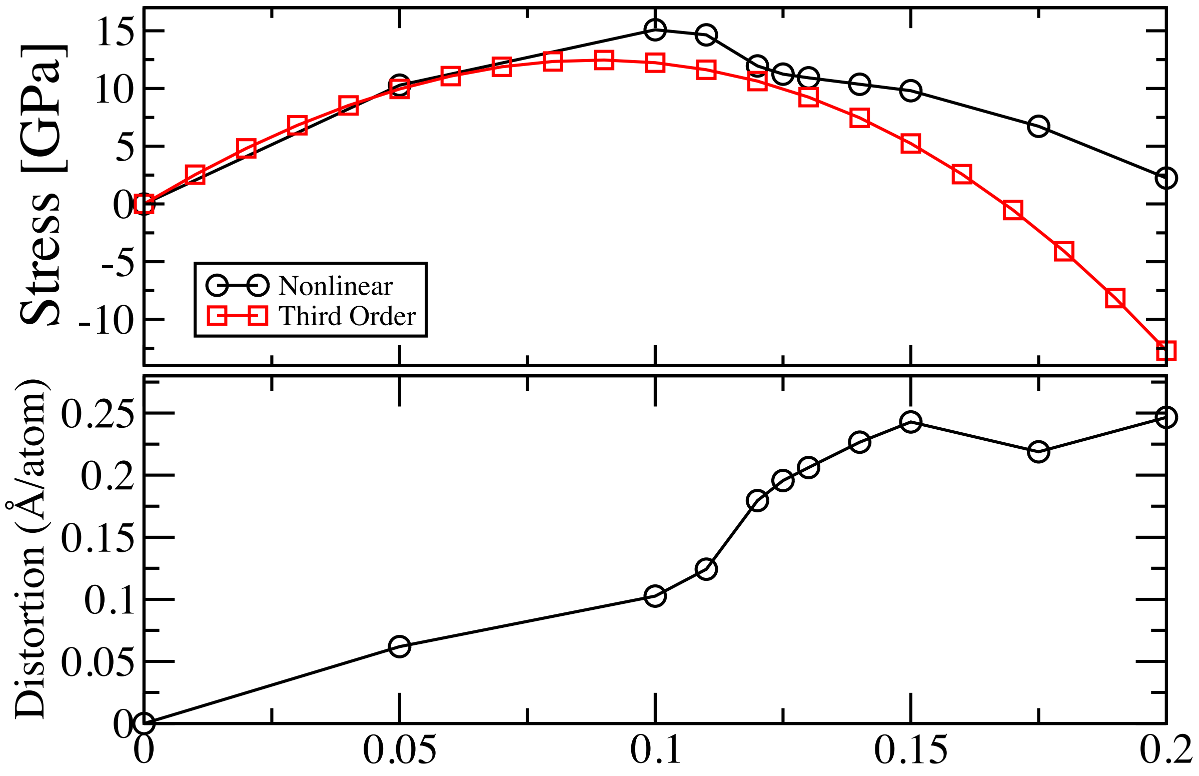
Stress [GPa]
15
10
5
0
-5
-10
Nonlinear
Third Order
Distortion (Å/atom)
0.25
0.2
0.15
0.1
0.05
0
0
0.05
0.1
0.15
0.2

# $Mo_3Nb_1$

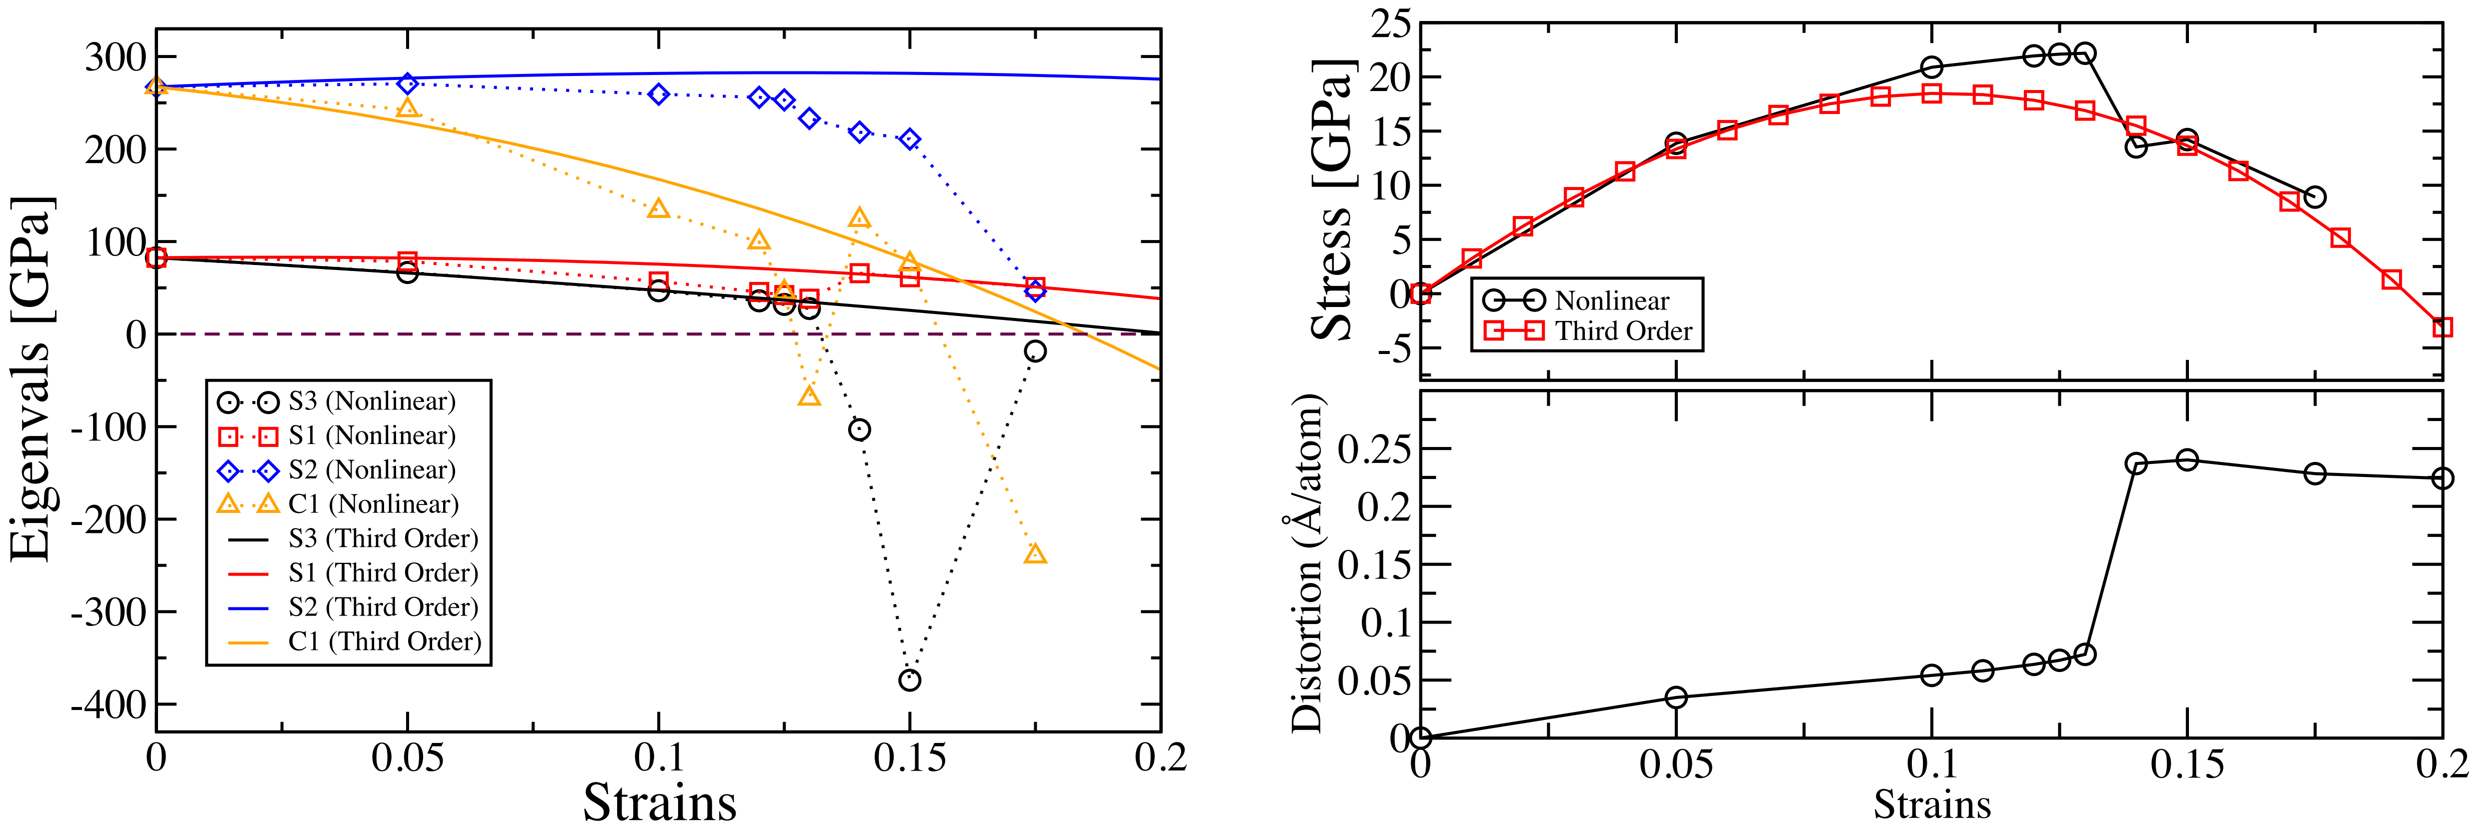

Eigenvals [GPa]
Strains
S3 (Nonlinear)
S1 (Nonlinear)
S2 (Nonlinear)
C1 (Nonlinear)
S3 (Third Order)
S1 (Third Order)
S2 (Third Order)
C1 (Third Order)
300
200
100
0
-100
-200
-300
-400
0
0.05
0.1
0.15
0.2
Stress [GPa]
Nonlinear
Third Order
25
20
15
10
5
0
-5
Distortion (Å/atom)
0.25
0.2
0.15
0.1
0.05
0
Strains

# $Mo_3Nb_1$ – Gauging Size Effect

Comparing eigenvalues, stress and distortion for 3x3x3 and 4x4x4 SQSs
The critical strains are similar but slightly higher for 3x3x3 system

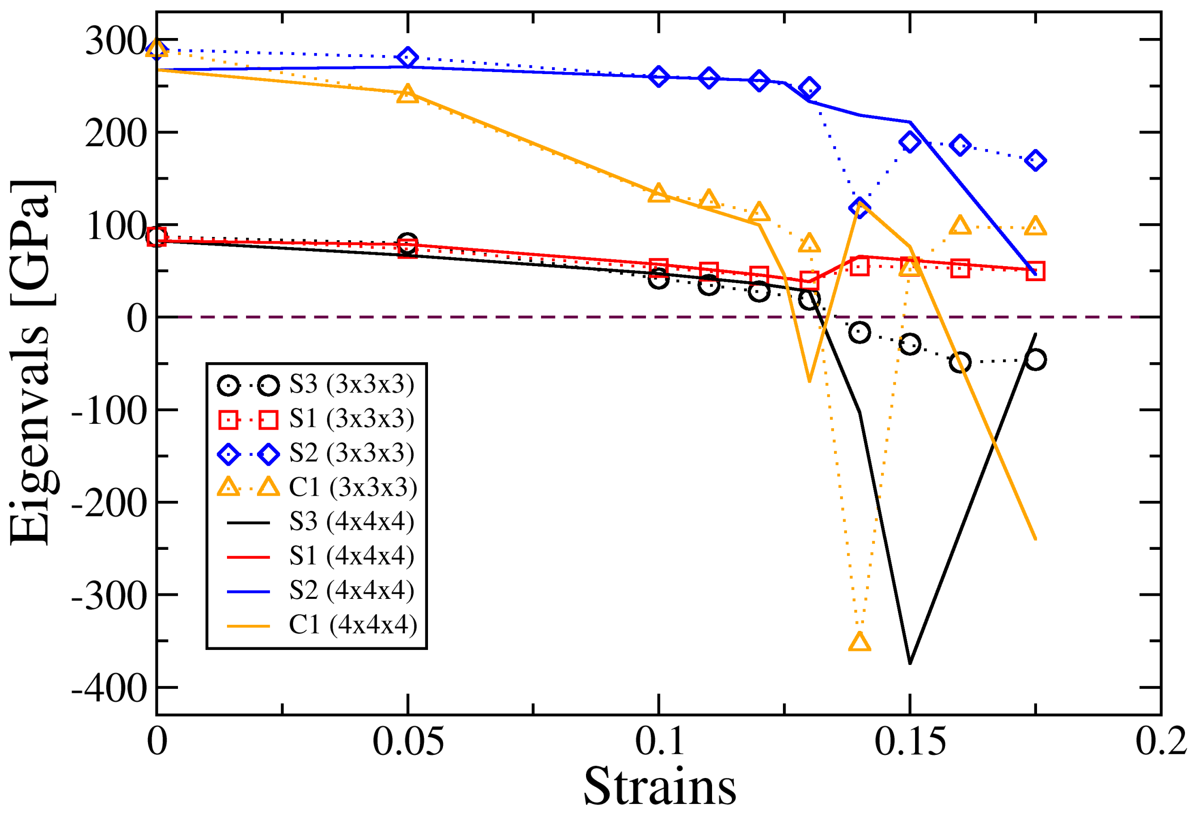


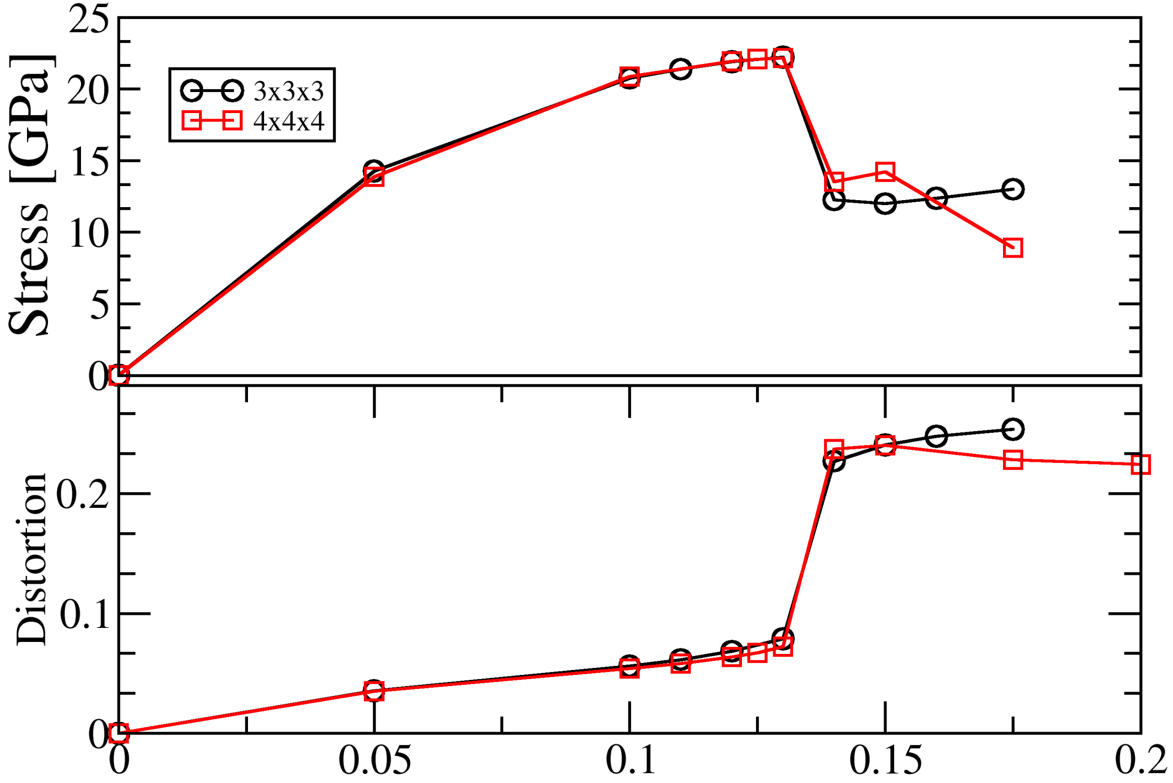

# $Mo_3Nb_1$ – Gauging Size Effect

We observe stacking fault and twinning in the 3x3x3 system.

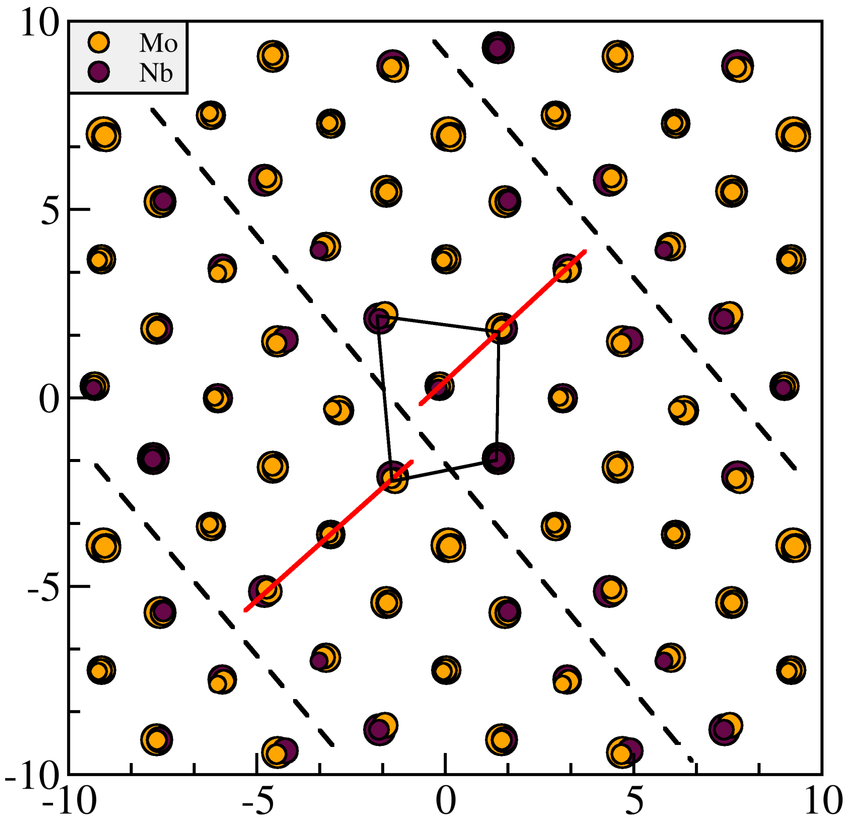


14% strain
[100] direction

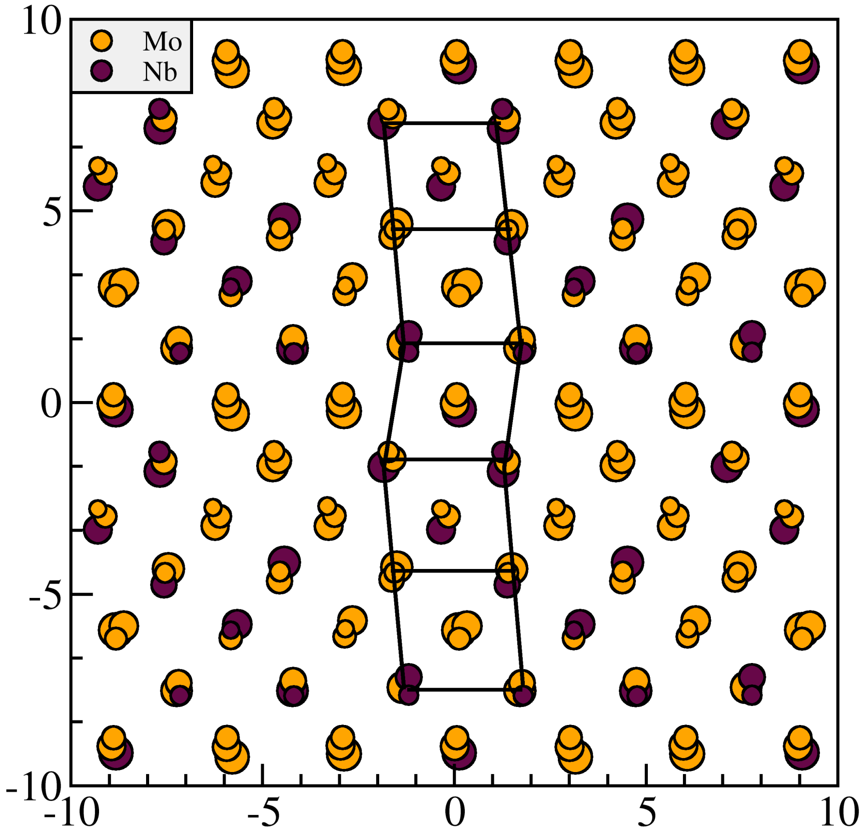


20% strain
[001] direction

# $Mo_3Re_1$

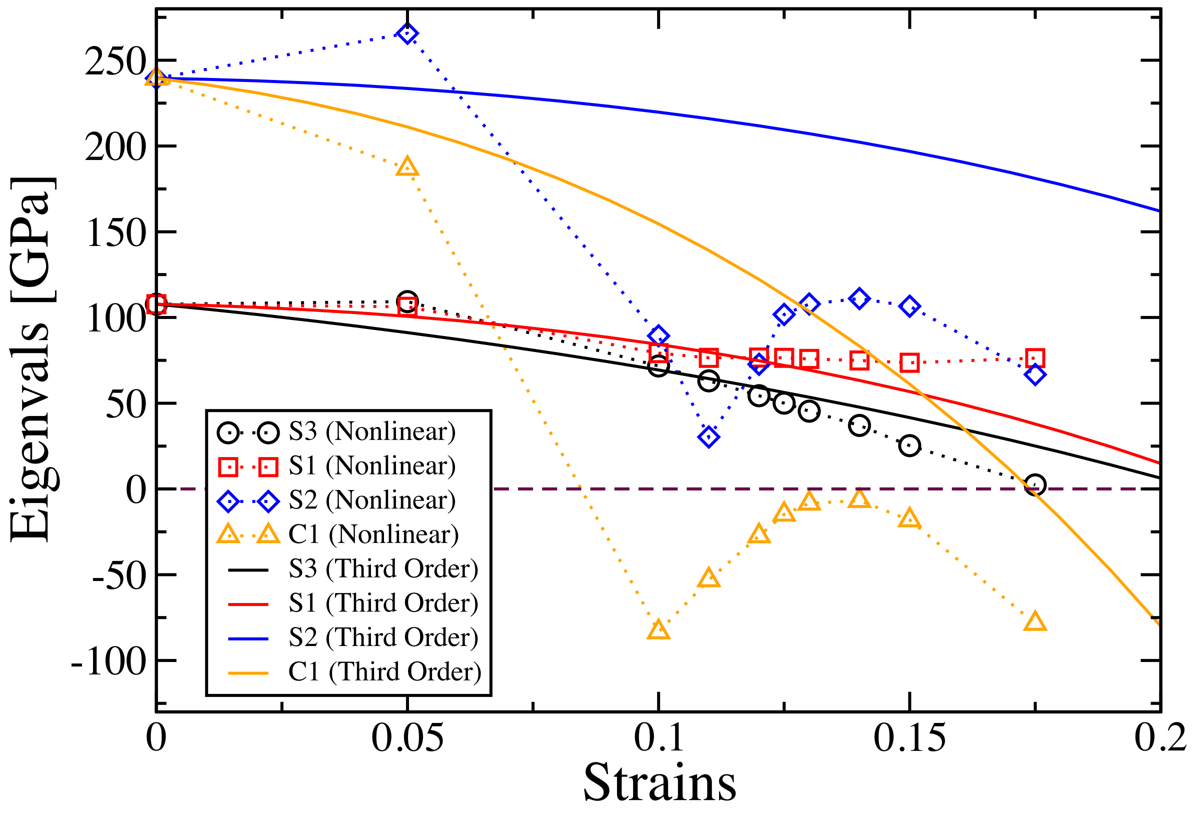

Eigenvals [GPa]
250
200
150
100
50
0
-50
-100
0
0.05
0.1
0.15
0.2
Strains
S3 (Nonlinear)
S1 (Nonlinear)
S2 (Nonlinear)
C1 (Nonlinear)
S3 (Third Order)
S1 (Third Order)
S2 (Third Order)
C1 (Third Order)


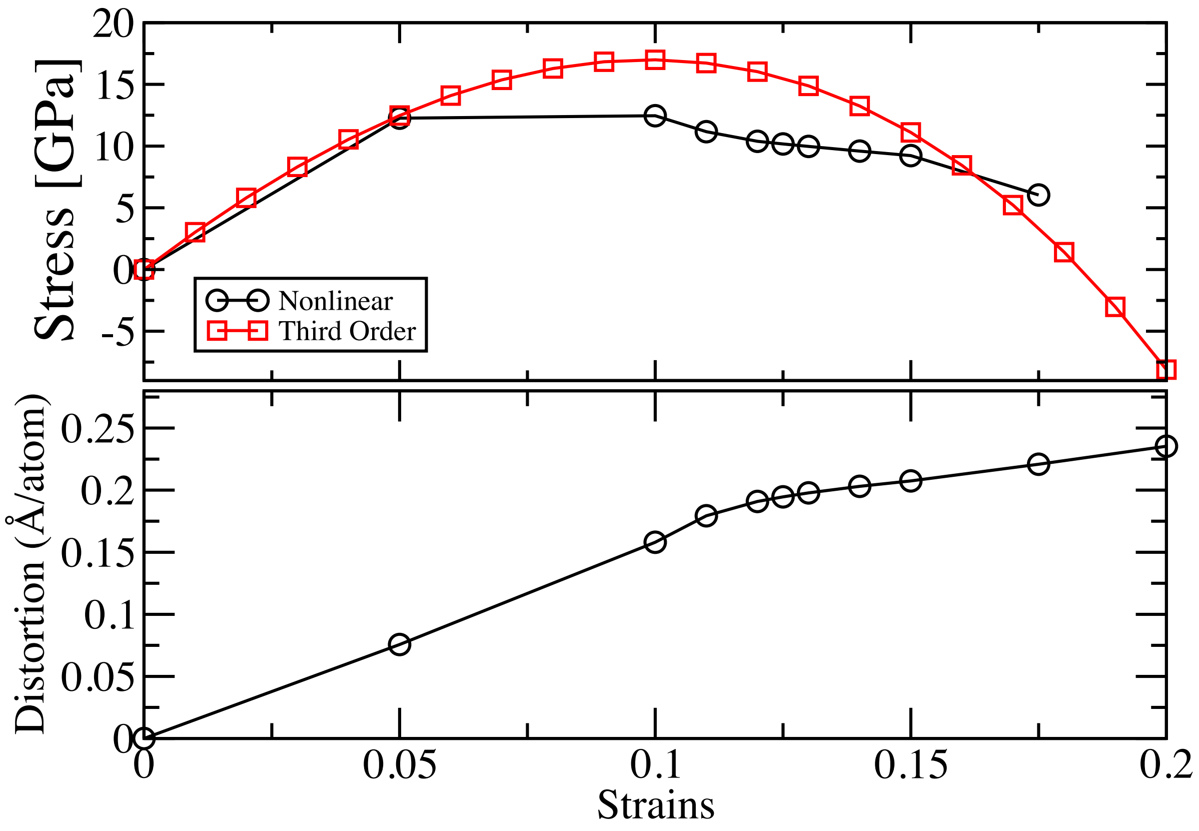

Stress [GPa]
20
15
10
5
0
-5
Nonlinear
Third Order
Distortion (Å/atom)
0.25
0.2
0.15
0.1
0.05
0
0
0.05
0.1
0.15
0.2
Strains

# $Mo_3Ru_1$

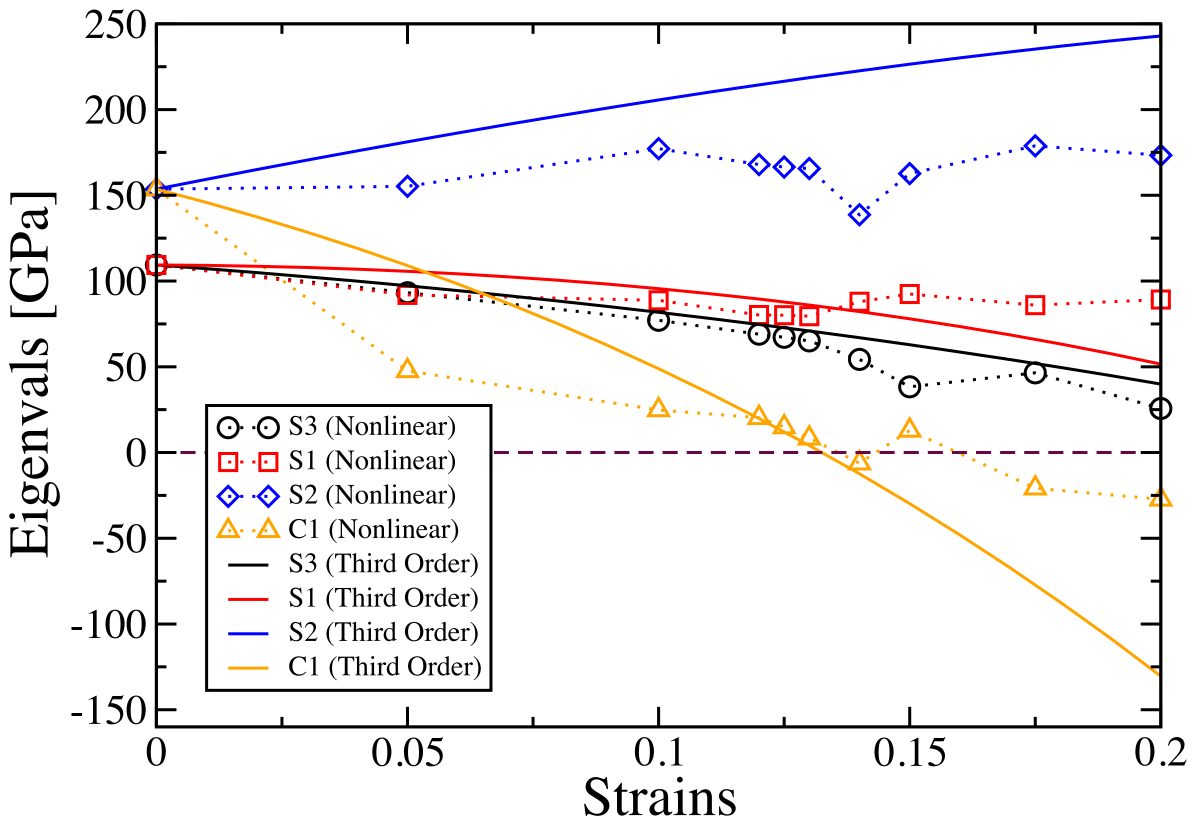

Eigenvals [GPa]
250
200
150
100
50
0
-50
-100
-150
0
0.05
0.1
0.15
0.2
Strains
S3 (Nonlinear)
S1 (Nonlinear)
S2 (Nonlinear)
C1 (Nonlinear)
S3 (Third Order)
S1 (Third Order)
S2 (Third Order)
C1 (Third Order)


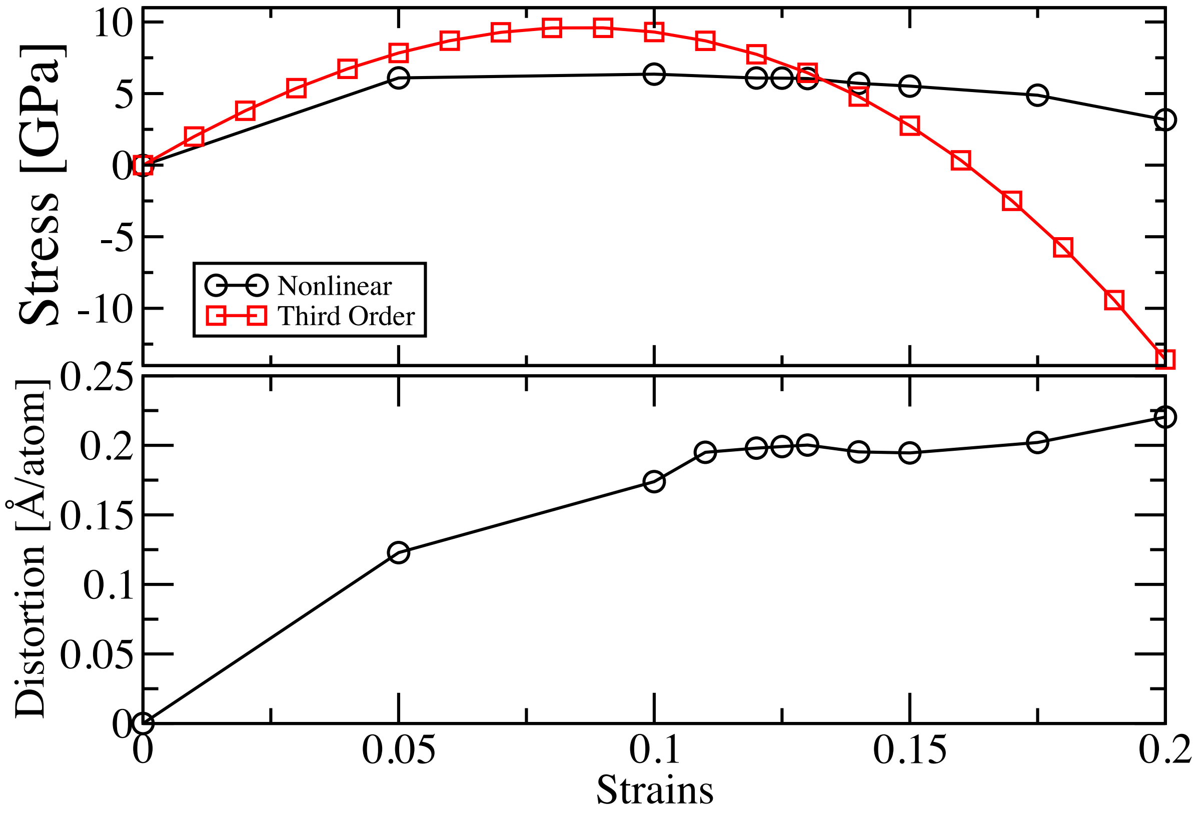

Stress [GPa]
10
5
0
-5
-10
Nonlinear
Third Order
Distortion [Å/atom]
0.25
0.2
0.15
0.1
0.05
0
0
0.05
0.1
0.15
0.2
Strains

# $Mo_3Si_1$

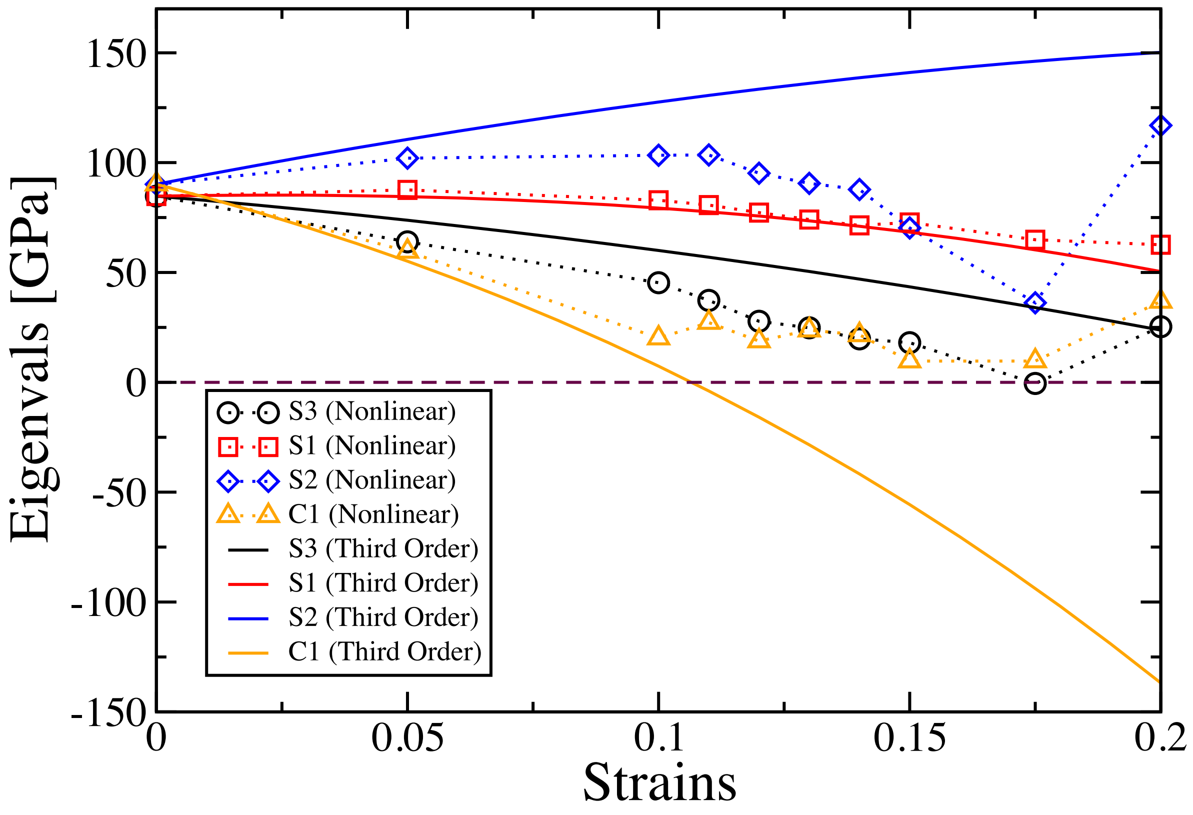
Eigenvals [GPa]
150
100
50
0
-50
-100
-150
0
0.05
0.1
0.15
0.2
Strains
S3 (Nonlinear)
S1 (Nonlinear)
S2 (Nonlinear)
C1 (Nonlinear)
S3 (Third Order)
S1 (Third Order)
S2 (Third Order)
C1 (Third Order)

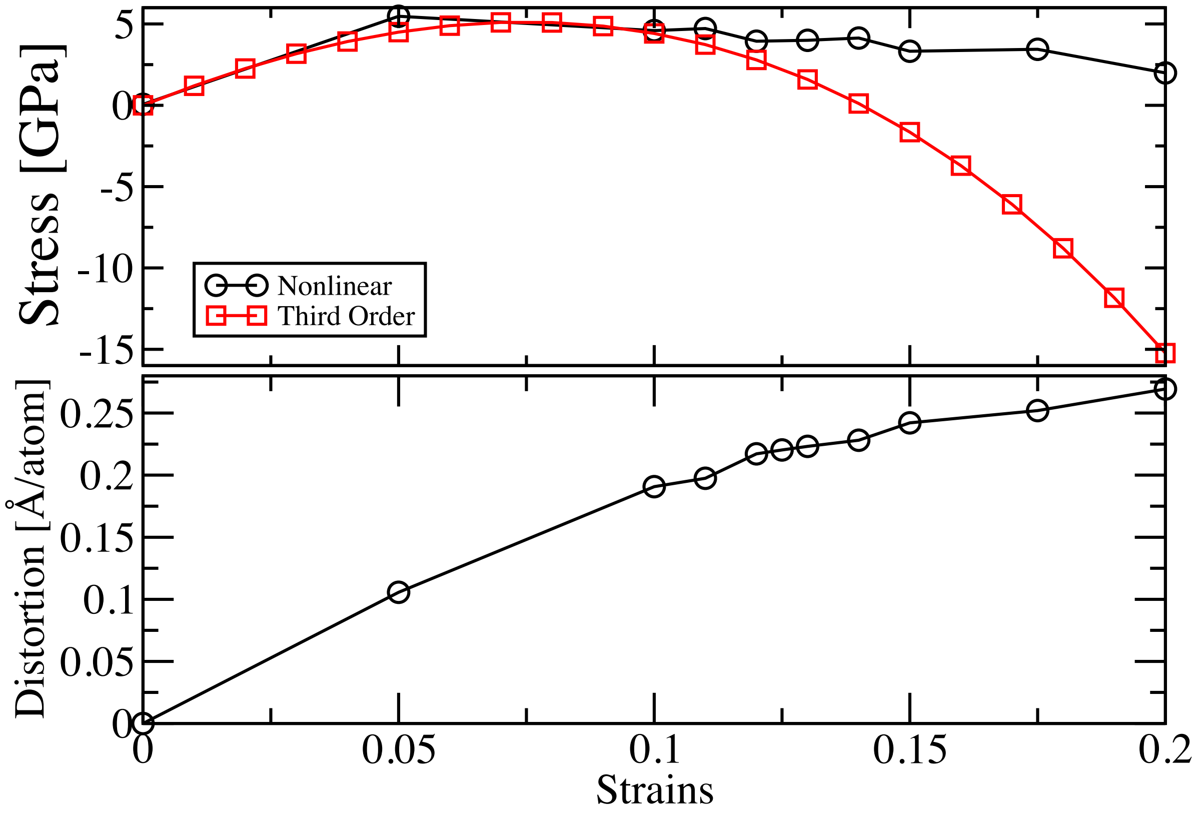
Stress [GPa]
5
0
-5
-10
-15
Nonlinear
Third Order
Distortion [Å/atom]
0.25
0.2
0.15
0.1
0.05
0
0
0.05
0.1
0.15
0.2
Strains

# $Mo_3Ta_1$

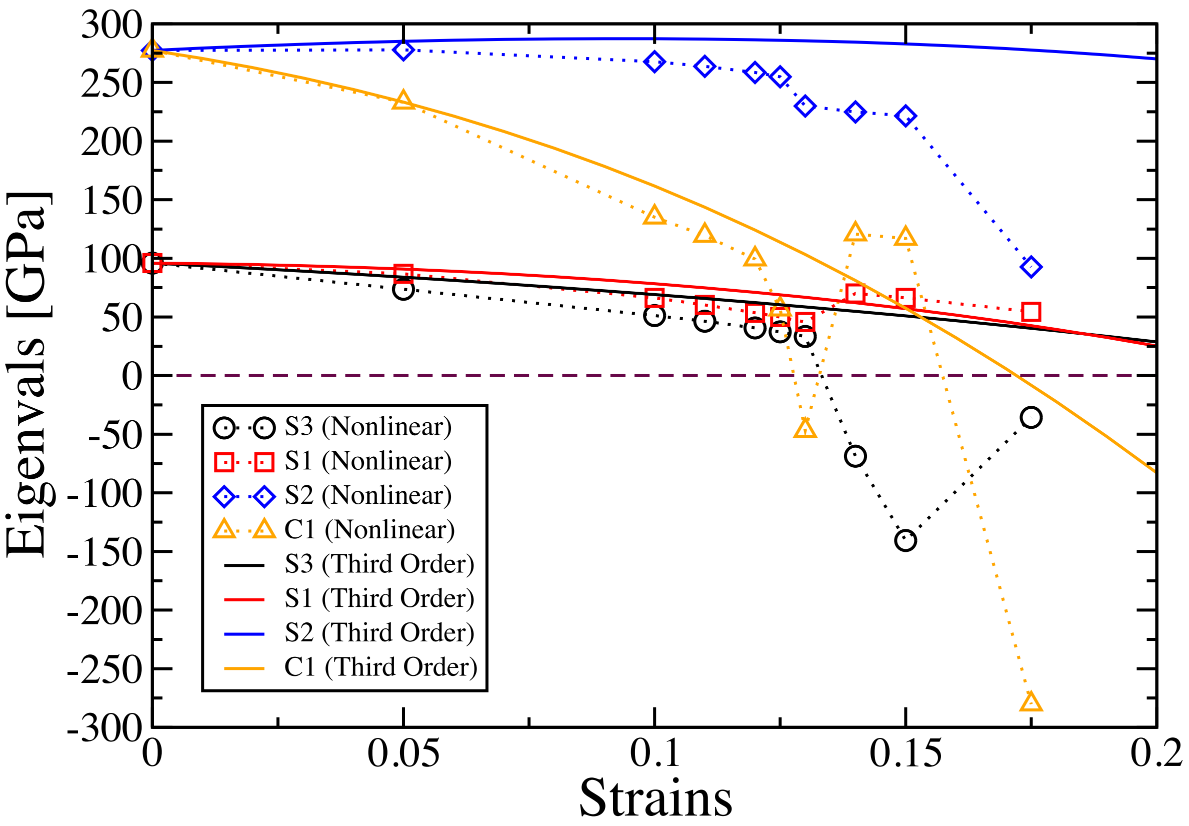
Eigenvals [GPa]
Strains
S3 (Nonlinear)
S1 (Nonlinear)
S2 (Nonlinear)
C1 (Nonlinear)
S3 (Third Order)
S1 (Third Order)
S2 (Third Order)
C1 (Third Order)
300
250
200
150
100
50
0
-50
-100
-150
-200
-250
-300
0
0.05
0.1
0.15
0.2

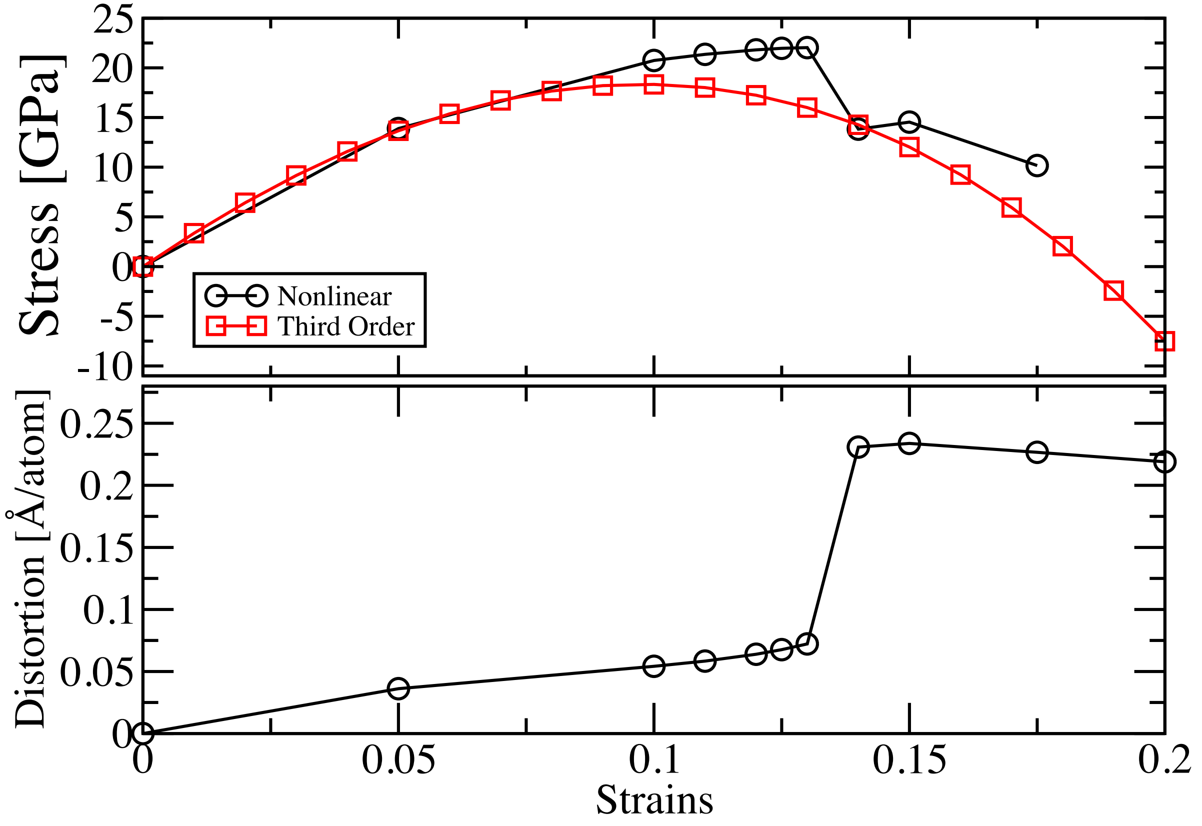
Stress [GPa]
Nonlinear
Third Order
25
20
15
10
5
0
-5
-10
Distortion [Å/atom]
0.25
0.2
0.15
0.1
0.05
0
Strains
0
0.05
0.1
0.15
0.2

# $Mo_3Ti_1$

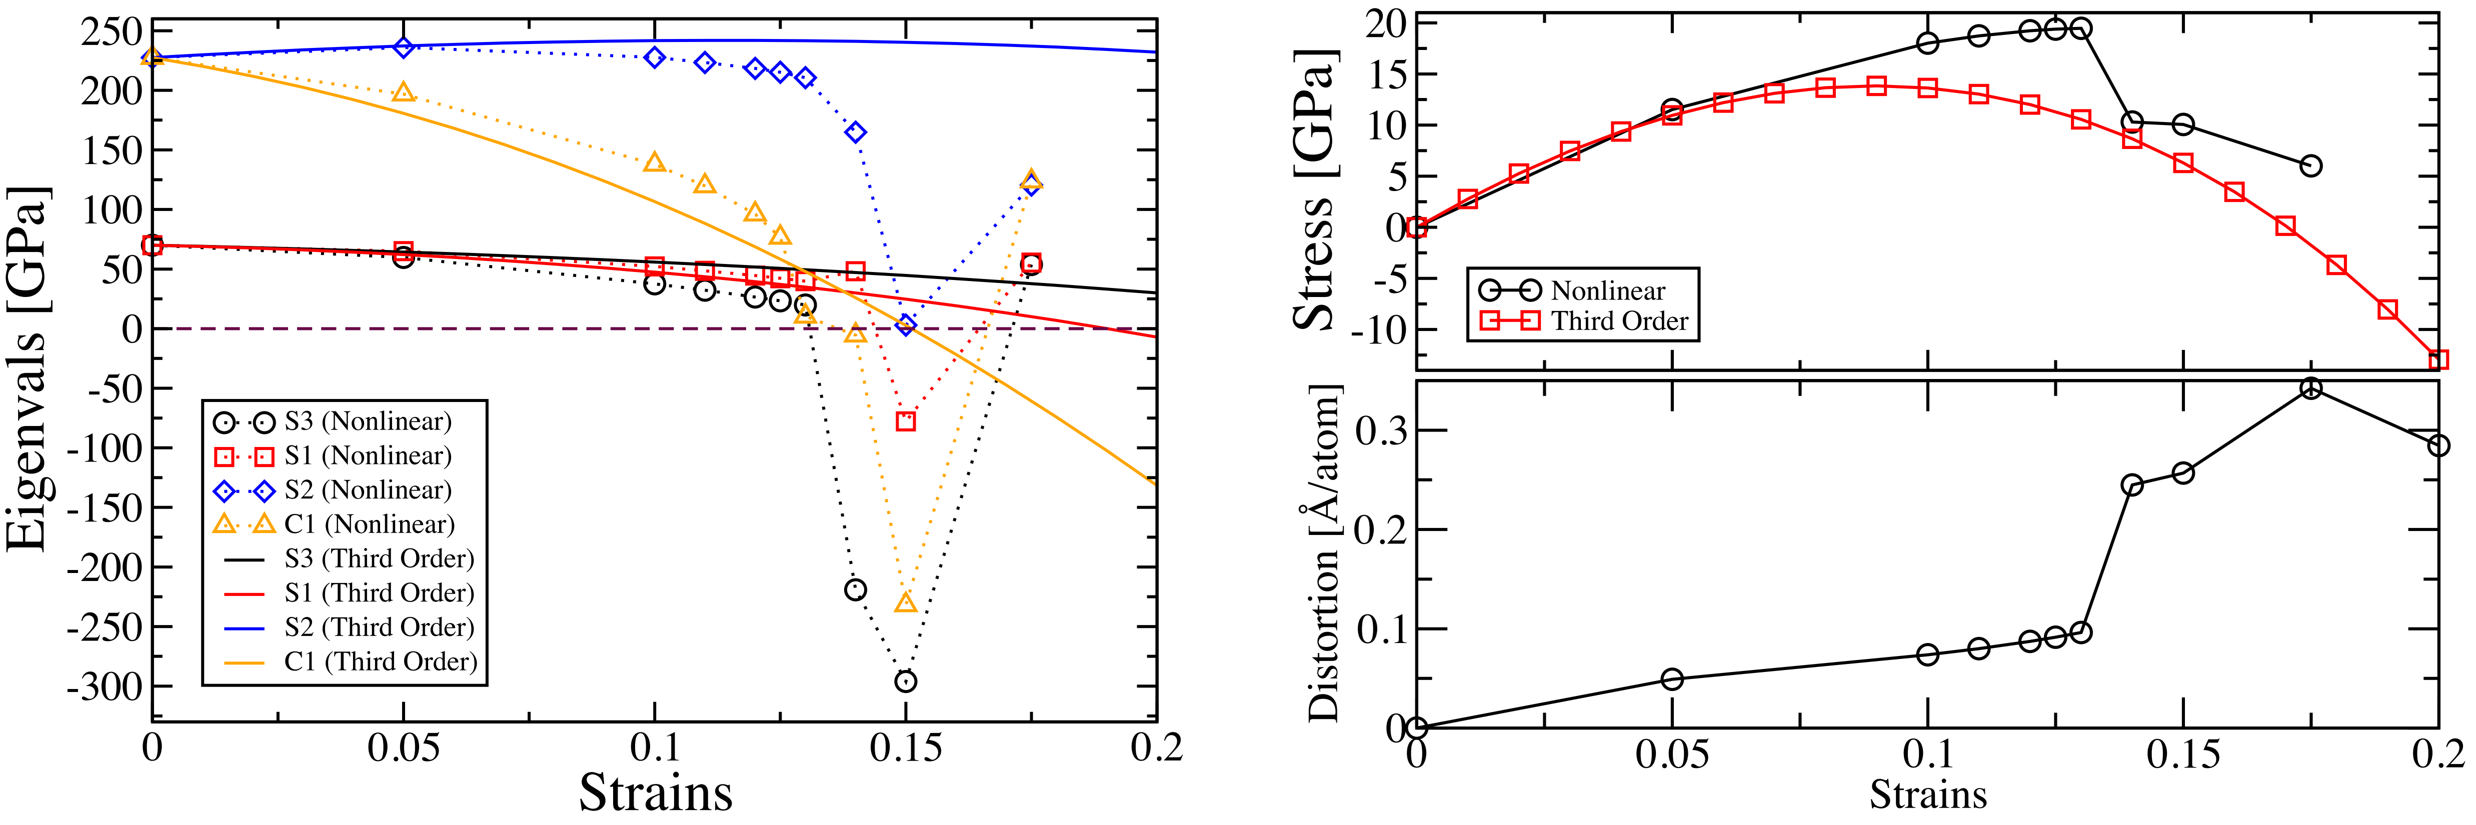

Eigenvals [GPa]
Strains
S3 (Nonlinear)
S1 (Nonlinear)
S2 (Nonlinear)
C1 (Nonlinear)
S3 (Third Order)
S1 (Third Order)
S2 (Third Order)
C1 (Third Order)
Stress [GPa]
Nonlinear
Third Order
Distortion [Å/atom]
Strains

# $Mo_3V_1$

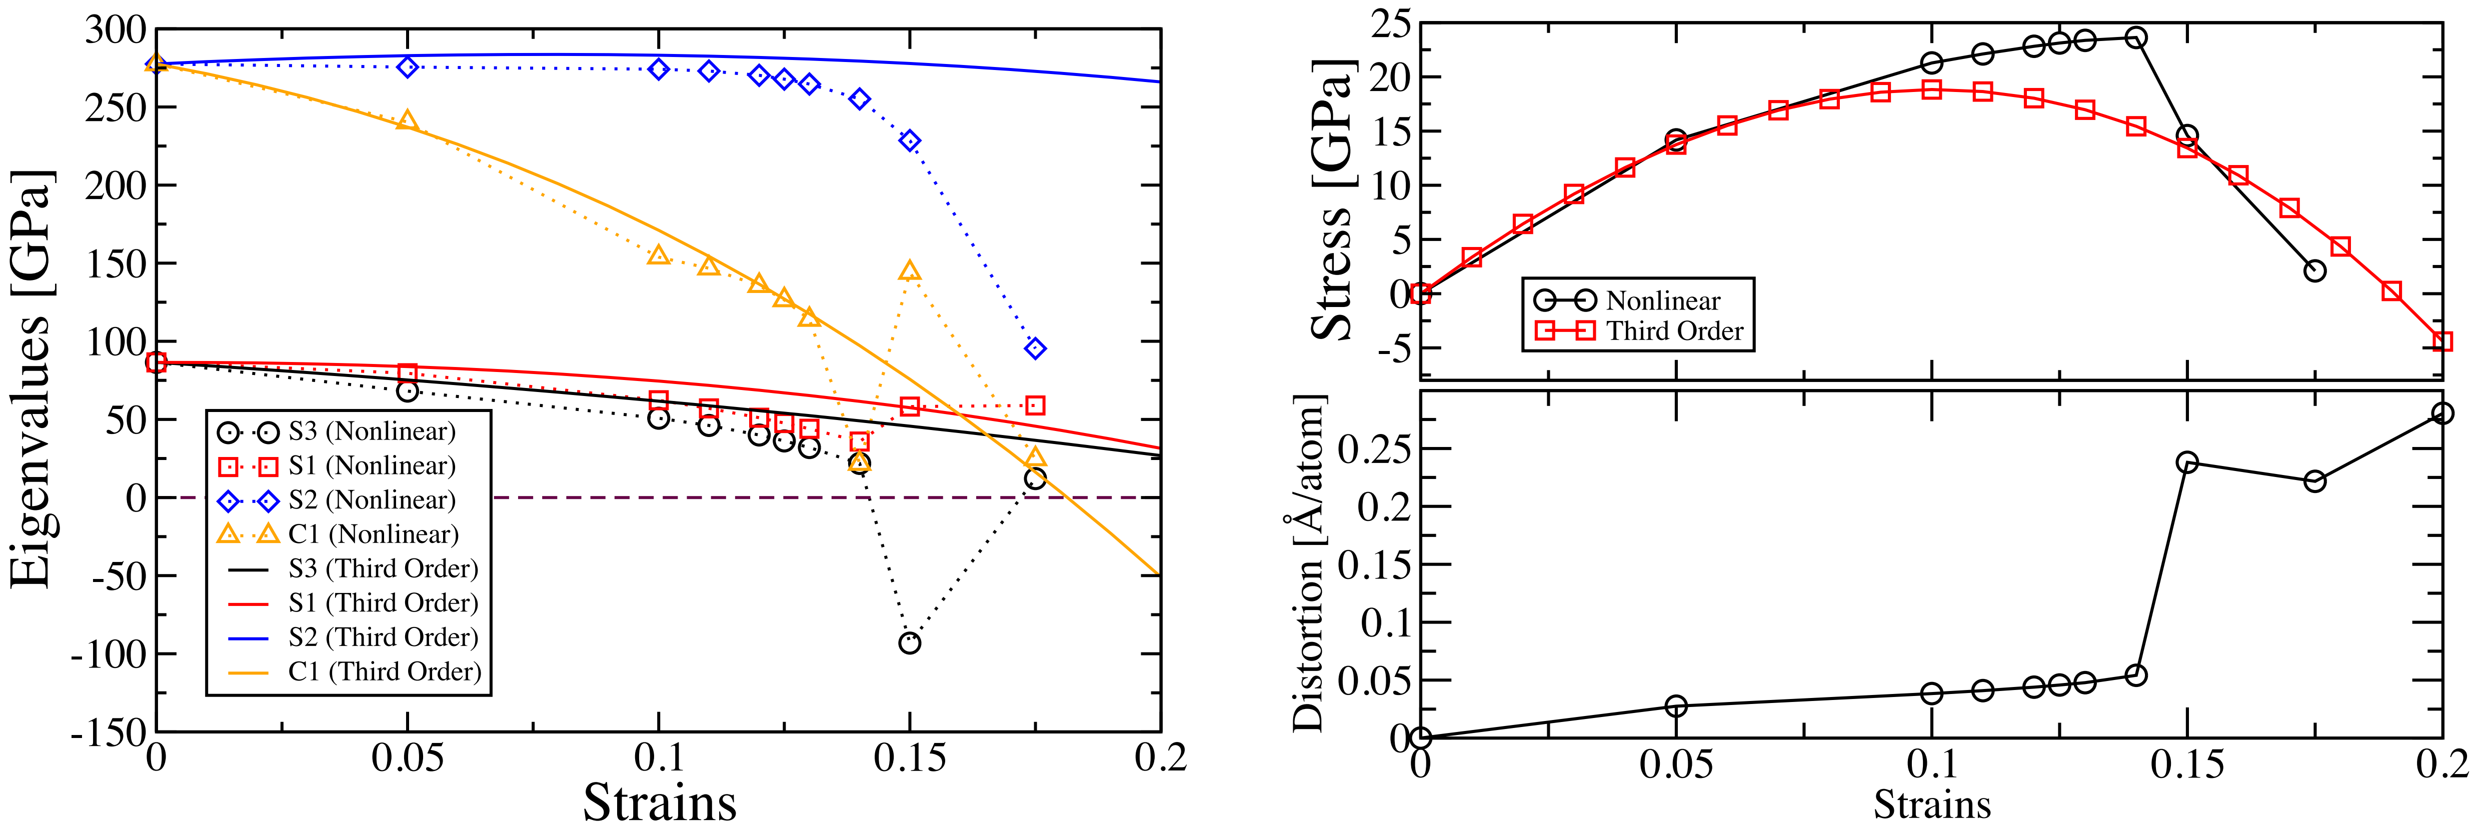

Eigenvalues [GPa]
300
250
200
150
100
50
0
-50
-100
-150
0
0.05
0.1
0.15
0.2
Strains
S3 (Nonlinear)
S1 (Nonlinear)
S2 (Nonlinear)
C1 (Nonlinear)
S3 (Third Order)
S1 (Third Order)
S2 (Third Order)
C1 (Third Order)
Stress [GPa]
25
20
15
10
5
0
-5
Nonlinear
Third Order
Distortion [Å/atom]
0.25
0.2
0.15
0.1
0.05
0
0
0.05
0.1
0.15
0.2
Strains

# $Mo_3W_1$

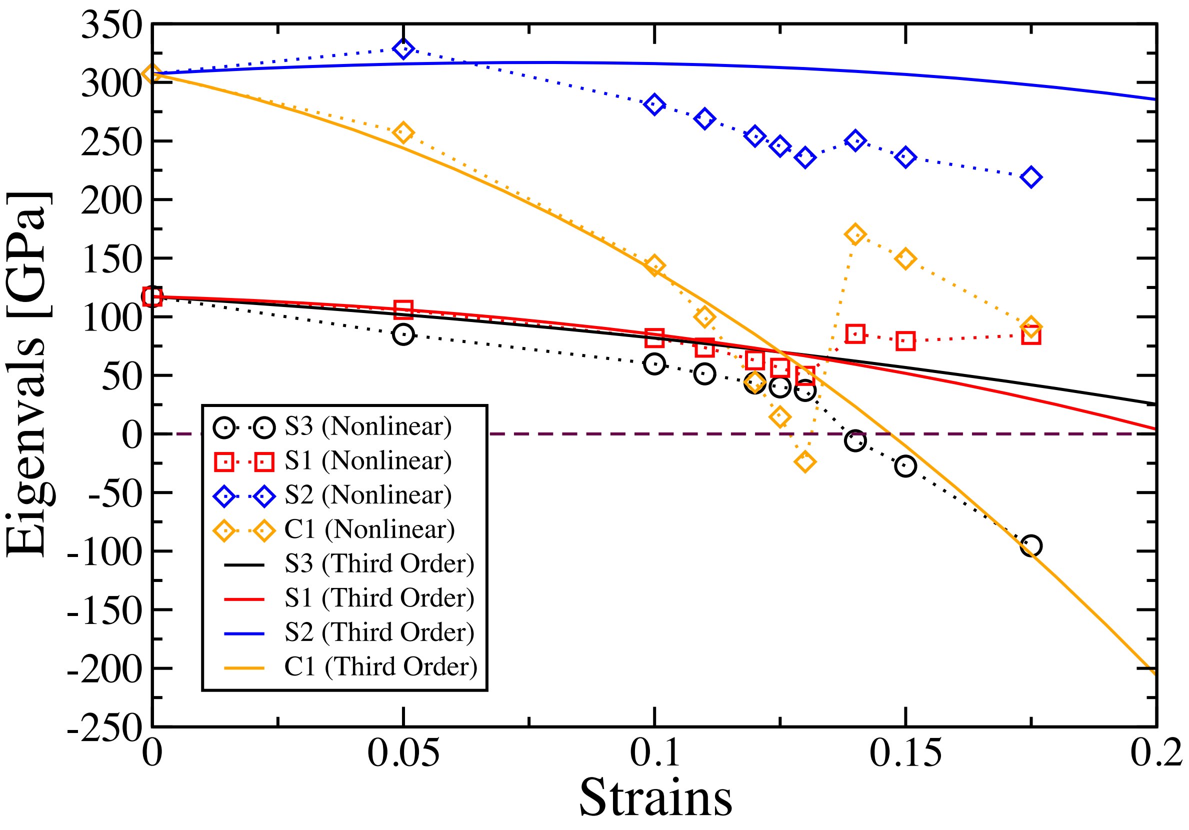
Eigenvals [GPa]
Strains
S3 (Nonlinear)
S1 (Nonlinear)
S2 (Nonlinear)
C1 (Nonlinear)
S3 (Third Order)
S1 (Third Order)
S2 (Third Order)
C1 (Third Order)

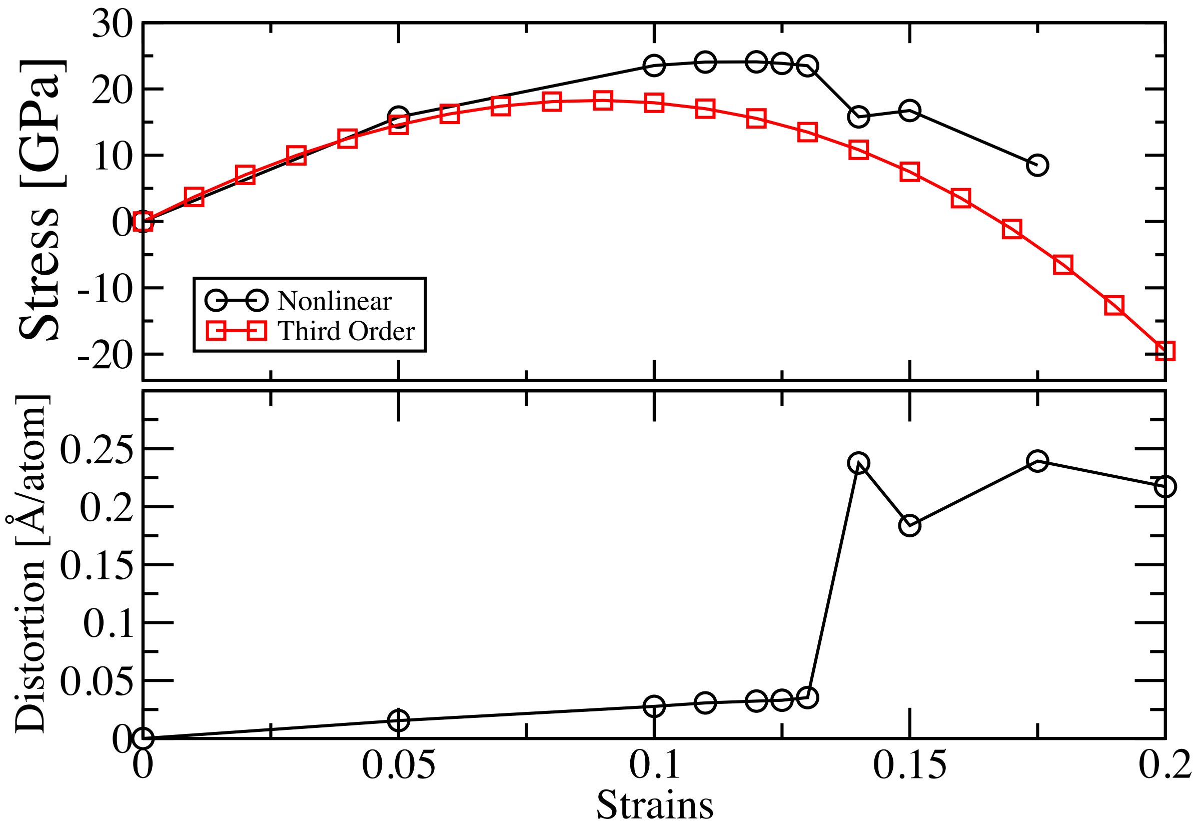
Stress [GPa]
Nonlinear
Third Order
Distortion [Å/atom]
Strains

# $Mo_3Zr_1$

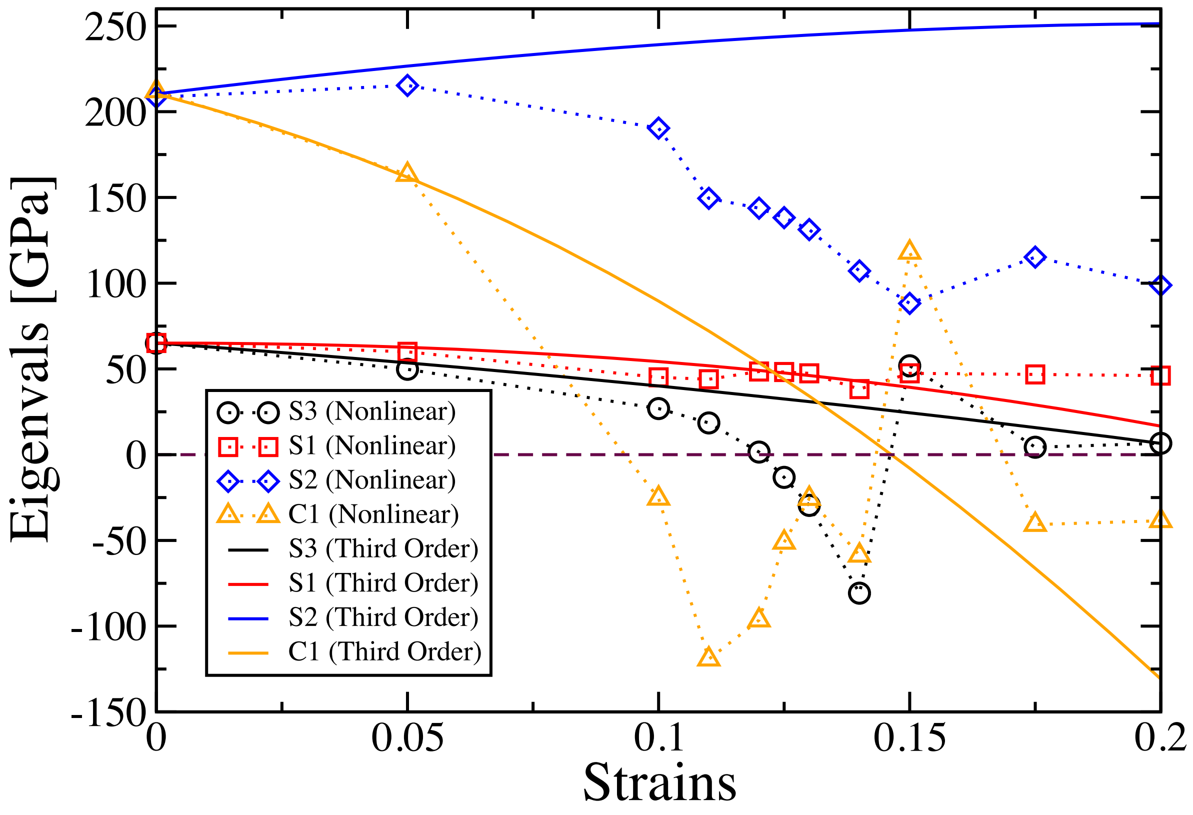

Eigenvals [GPa]
250
200
150
100
50
0
-50
-100
-150
0
0.05
0.1
0.15
0.2
Strains
S3 (Nonlinear)
S1 (Nonlinear)
S2 (Nonlinear)
C1 (Nonlinear)
S3 (Third Order)
S1 (Third Order)
S2 (Third Order)
C1 (Third Order)


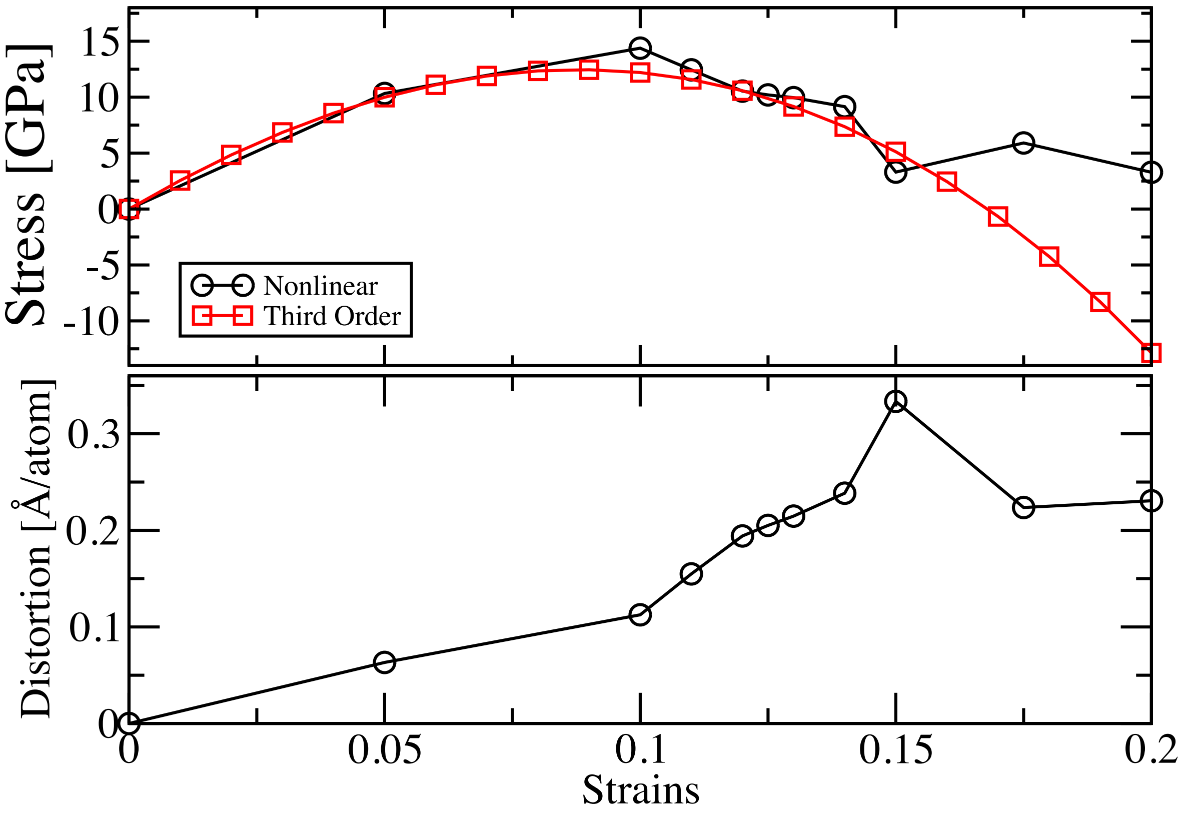

Stress [GPa]
15
10
5
0
-5
-10
Nonlinear
Third Order
Distortion [Å/atom]
0.3
0.2
0.1
0
0
0.05
0.1
0.15
0.2
Strains

# Nb-based binaries

Wallace tensor eigenvalues, stress, lattice distortion

# $Nb_3Al_1$

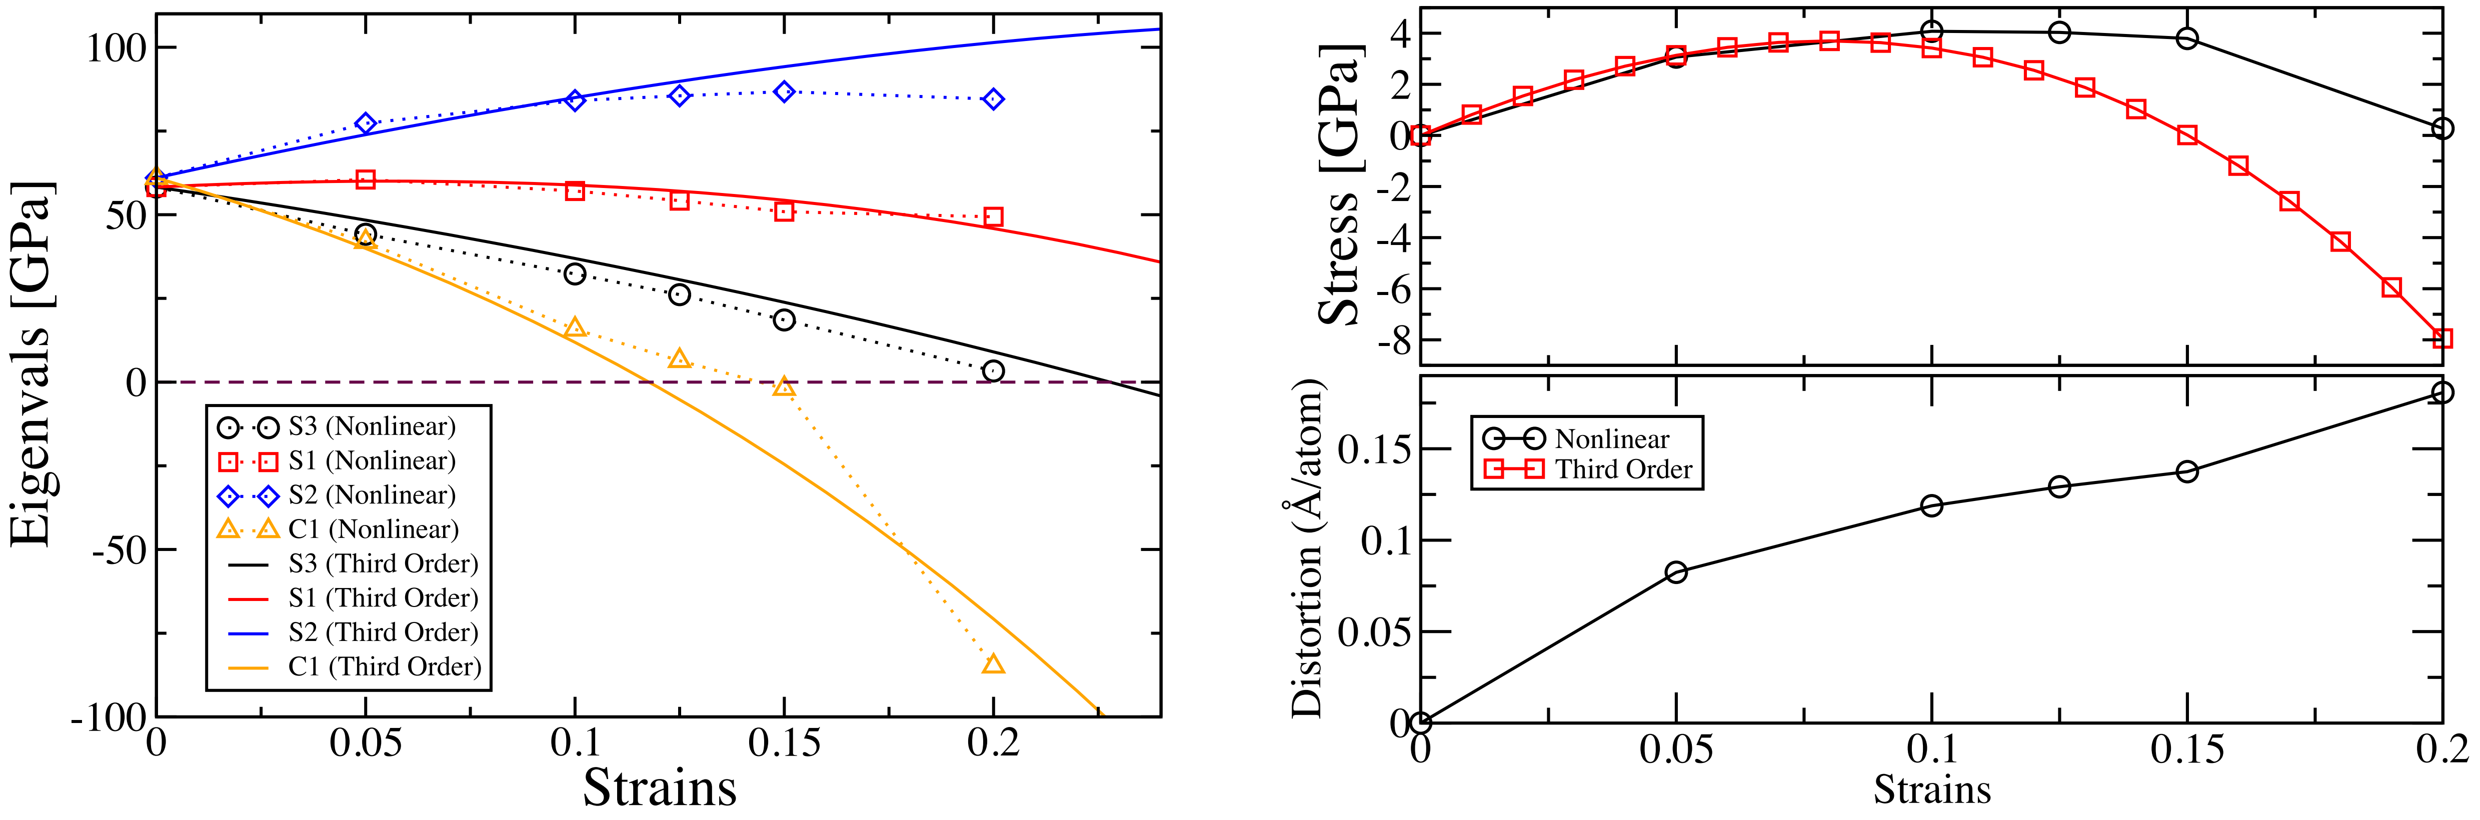

Eigenvals [GPa]
100
50
0
-50
-100
0
0.05
0.1
0.15
0.2
Strains
S3 (Nonlinear)
S1 (Nonlinear)
S2 (Nonlinear)
C1 (Nonlinear)
S3 (Third Order)
S1 (Third Order)
S2 (Third Order)
C1 (Third Order)
Stress [GPa]
4
2
0
-2
-4
-6
-8
Distortion (Å/atom)
0.15
0.1
0.05
0
Nonlinear
Third Order
0
0.05
0.1
0.15
0.2
Strains

# $Nb_3Cr_1$

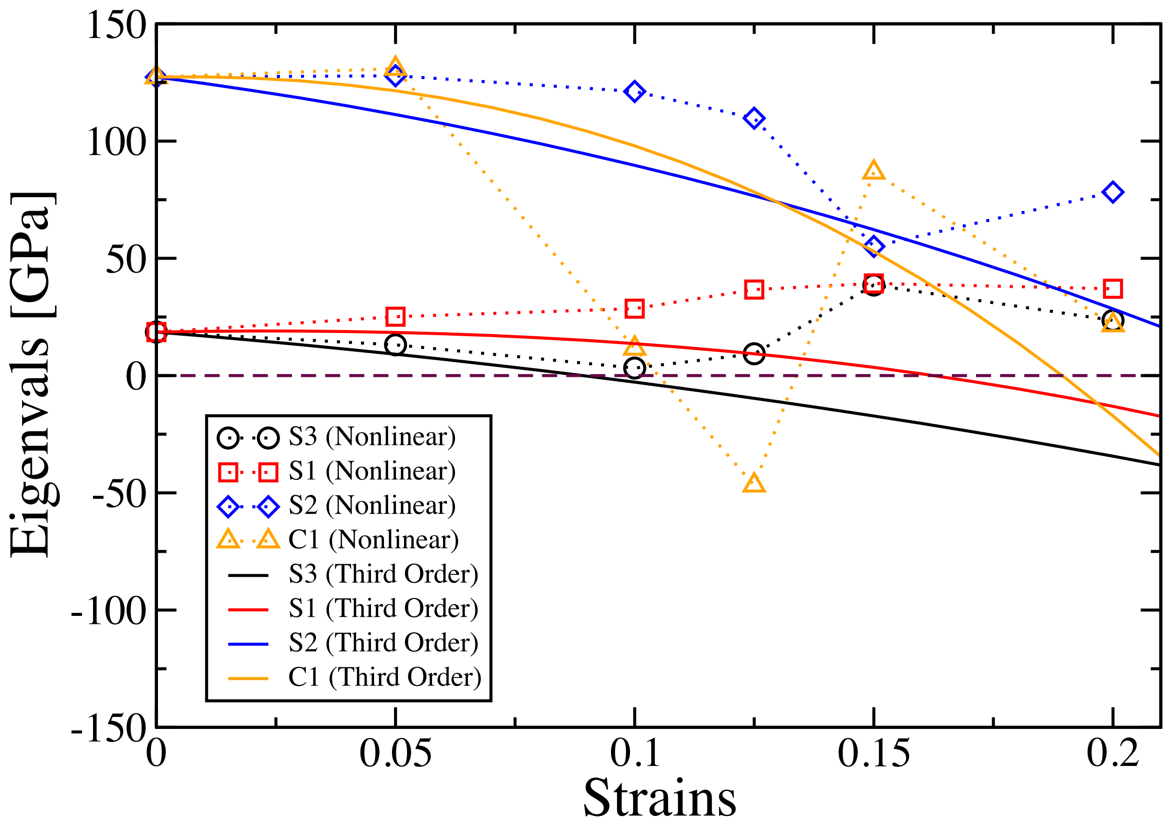

Eigenvals [GPa]
Strains
S3 (Nonlinear)
S1 (Nonlinear)
S2 (Nonlinear)
C1 (Nonlinear)
S3 (Third Order)
S1 (Third Order)
S2 (Third Order)
C1 (Third Order)


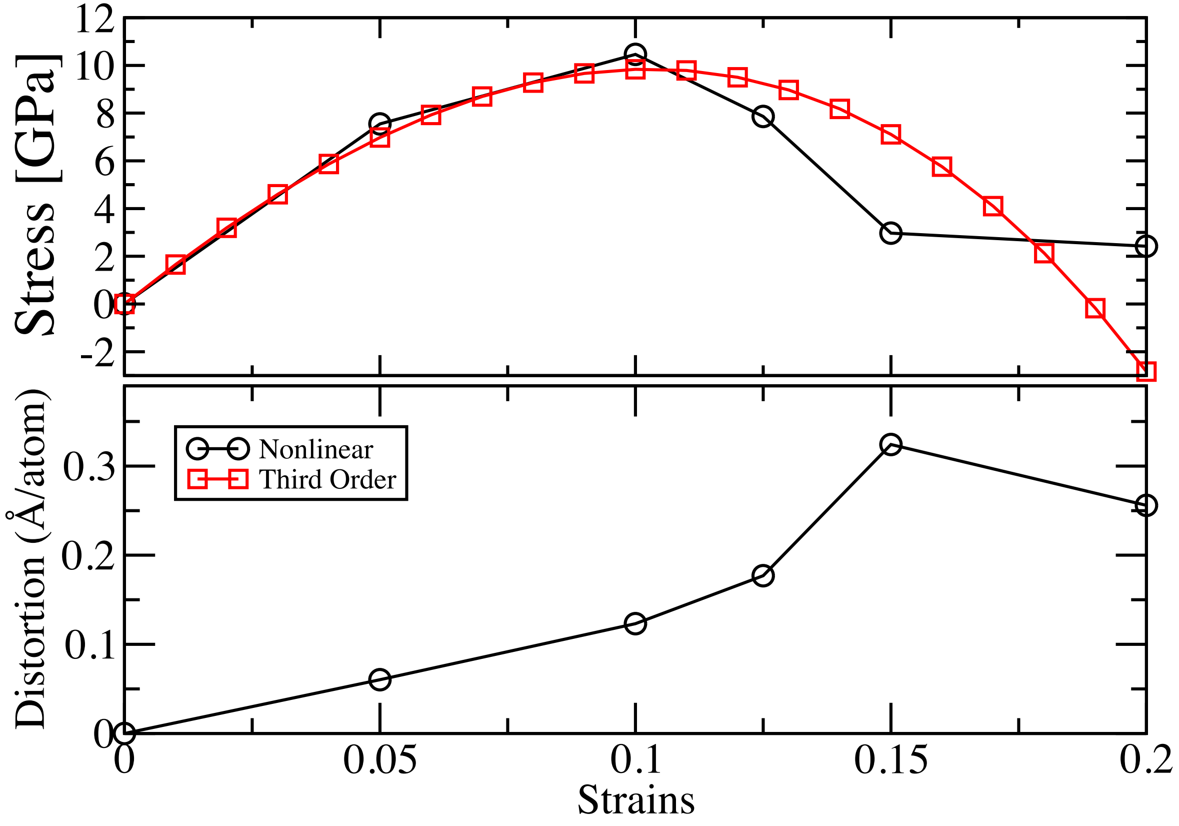

Stress [GPa]
Distortion (Å/atom)
Nonlinear
Third Order
Strains

# $Nb_3Hf_1$

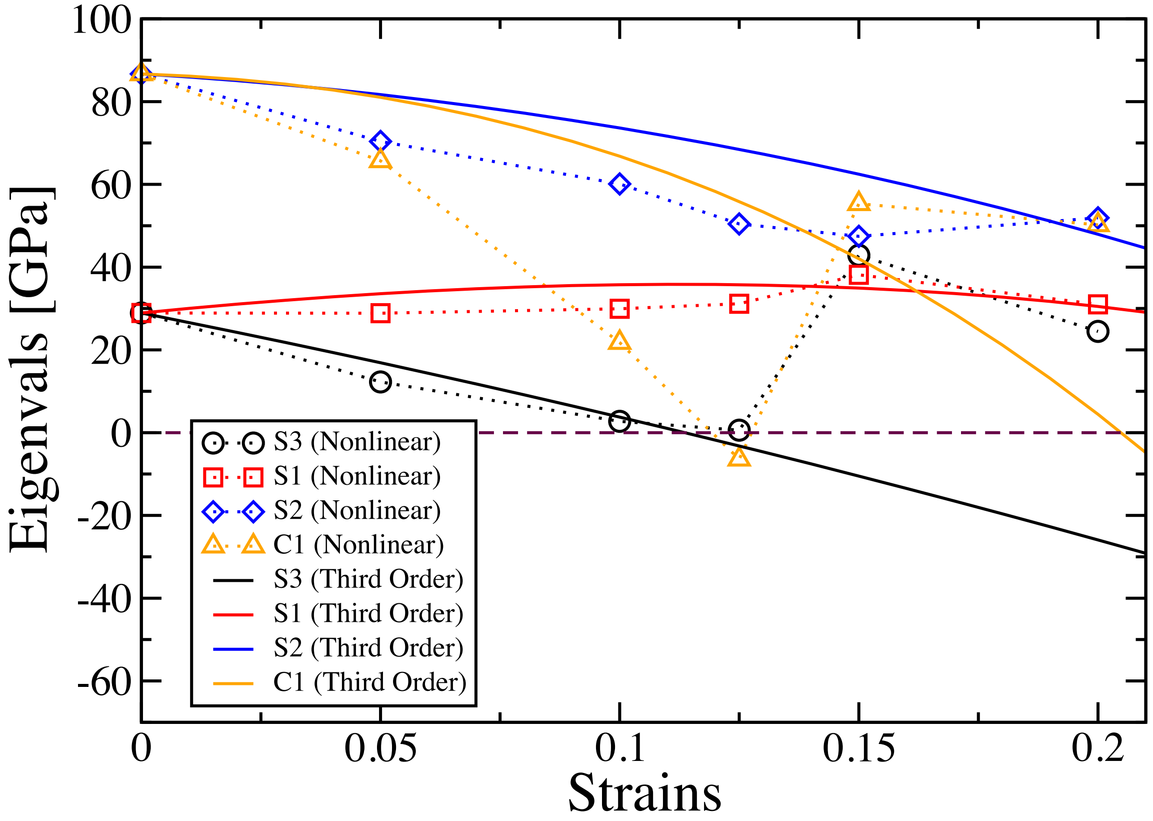

Eigenvals [GPa]
Strains
S3 (Nonlinear)
S1 (Nonlinear)
S2 (Nonlinear)
C1 (Nonlinear)
S3 (Third Order)
S1 (Third Order)
S2 (Third Order)
C1 (Third Order)
100
80
60
40
20
0
-20
-40
-60
0
0.05
0.1
0.15
0.2


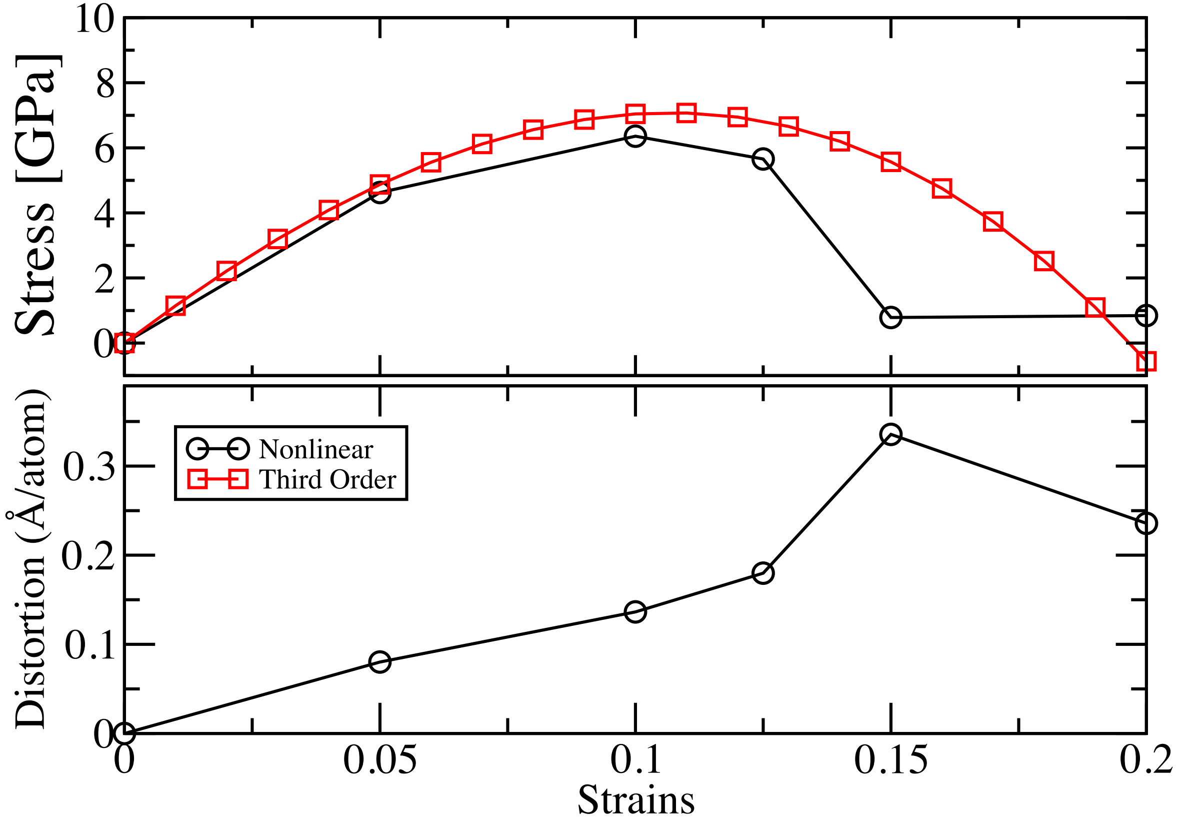

Stress [GPa]
Distortion (Å/atom)
Strains
Nonlinear
Third Order
10
8
6
4
2
0
0.3
0.2
0.1
0
0
0.05
0.1
0.15
0.2

# $Nb_3Mo_1$

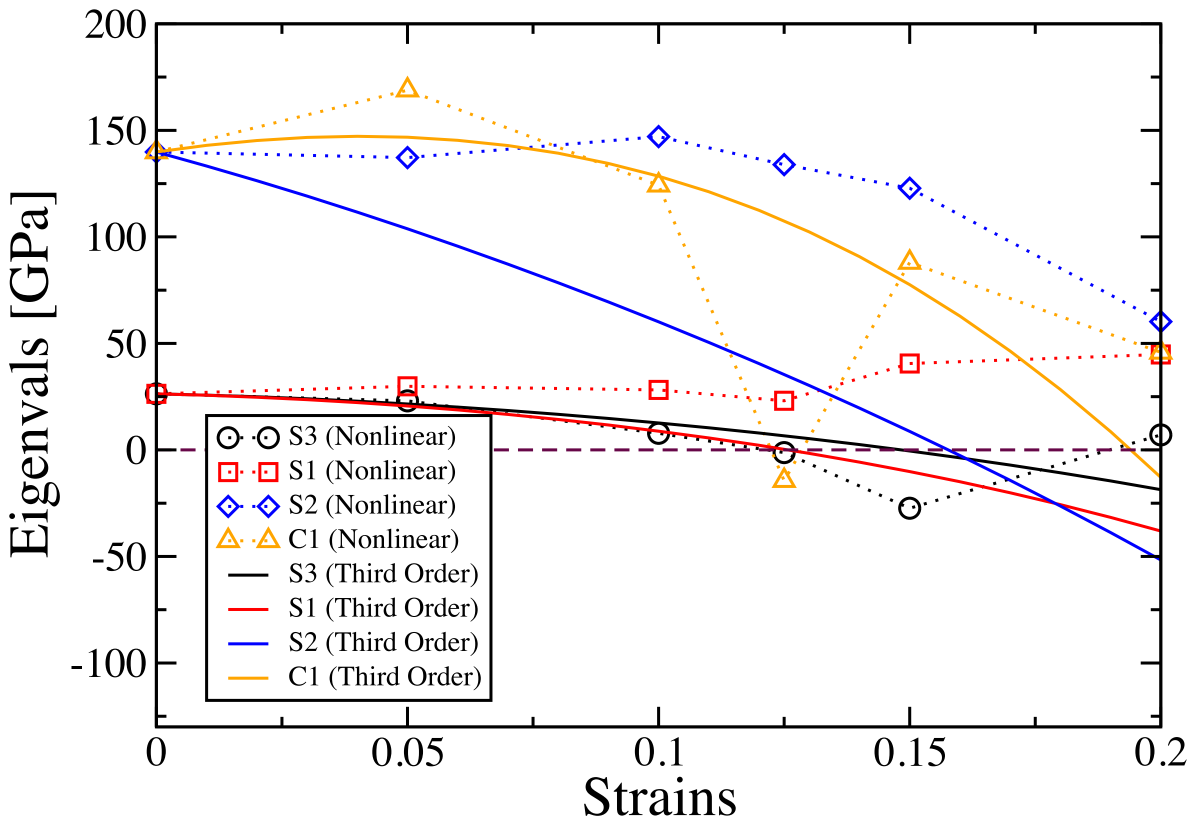

Eigenvals [GPa]
Strains
S3 (Nonlinear)
S1 (Nonlinear)
S2 (Nonlinear)
C1 (Nonlinear)
S3 (Third Order)
S1 (Third Order)
S2 (Third Order)
C1 (Third Order)


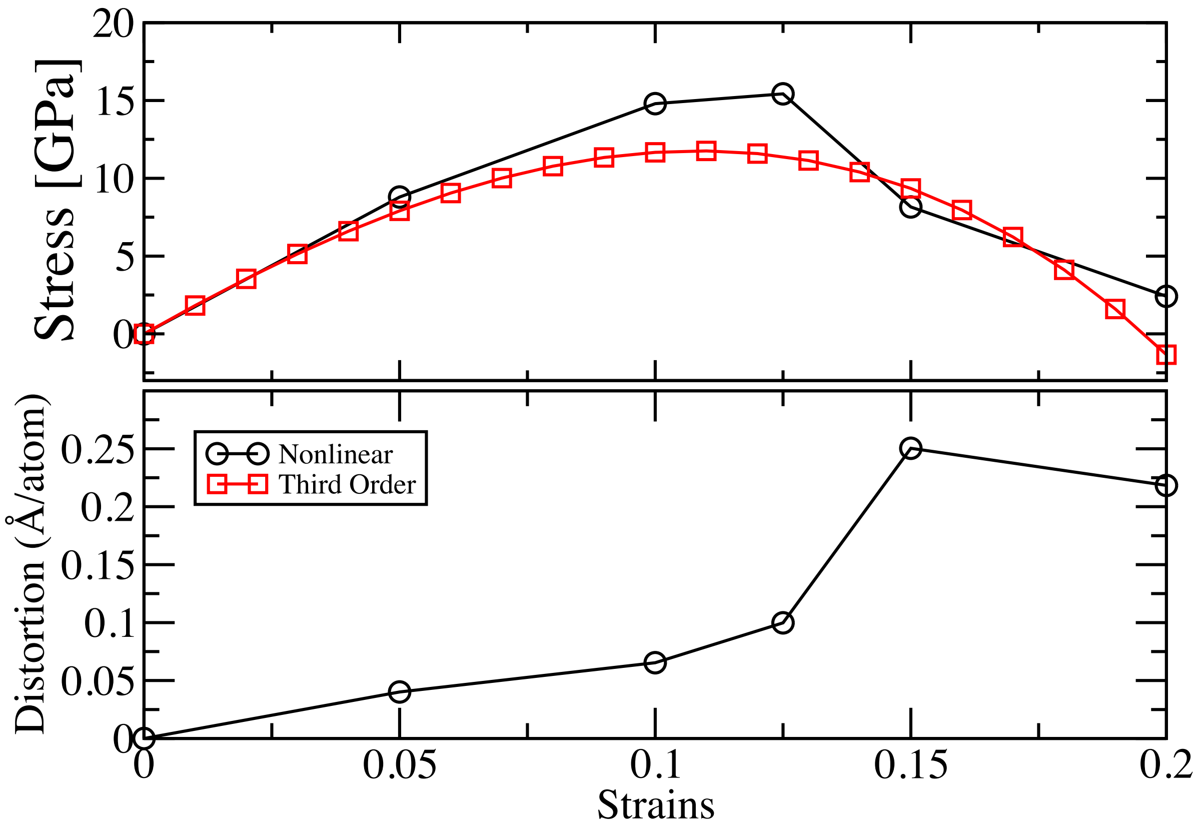

Stress [GPa]
Distortion (Å/atom)
Nonlinear
Third Order
Strains

# $Nb_3Re_1$

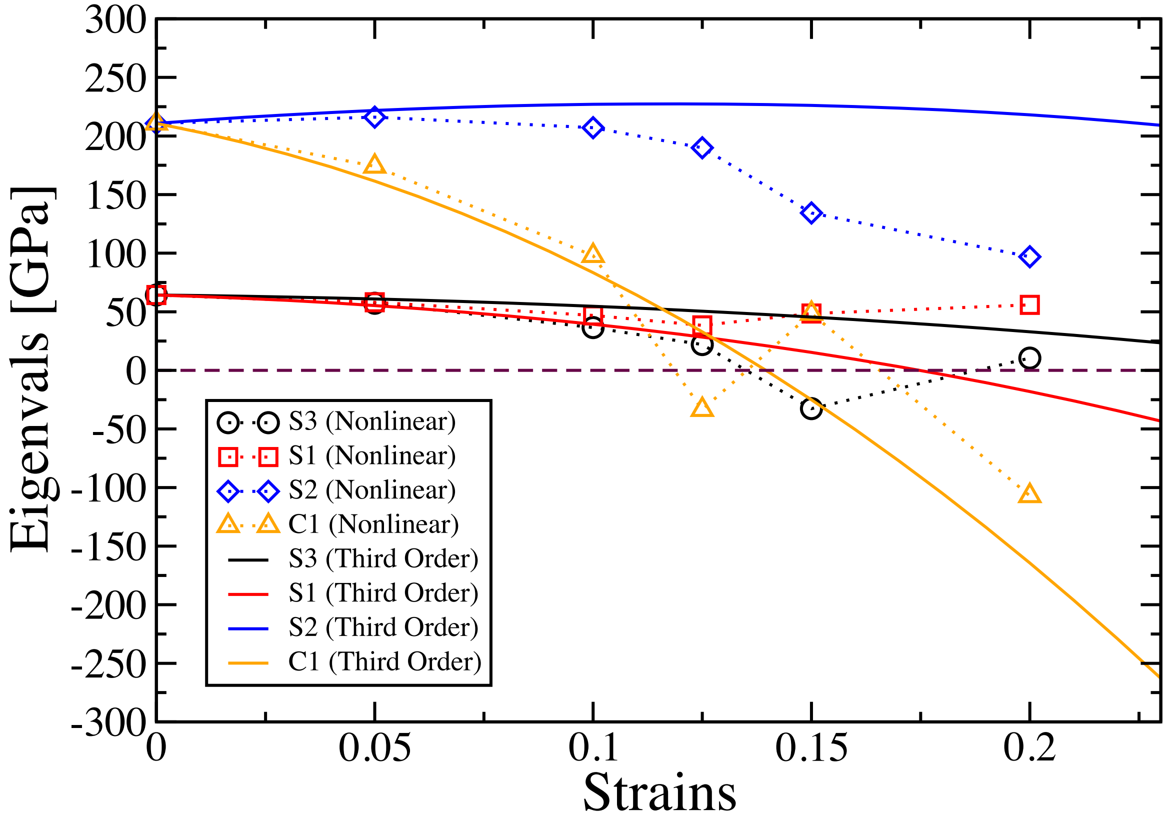
Eigenvals [GPa]
Strains
300
250
200
150
100
50
0
-50
-100
-150
-200
-250
-300
0
0.05
0.1
0.15
0.2
S3 (Nonlinear)
S1 (Nonlinear)
S2 (Nonlinear)
C1 (Nonlinear)
S3 (Third Order)
S1 (Third Order)
S2 (Third Order)
C1 (Third Order)

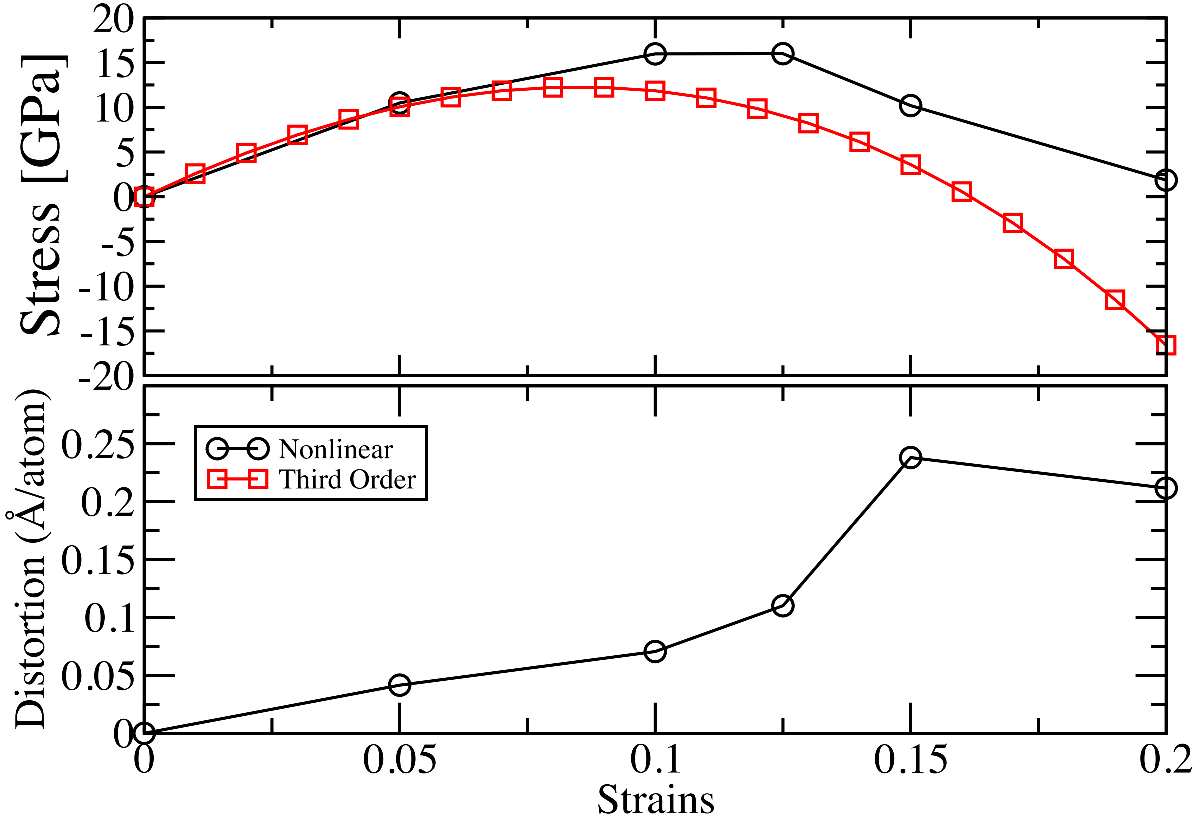
Stress [GPa]
20
15
10
5
0
-5
-10
-15
-20
Distortion (Å/atom)
0.25
0.2
0.15
0.1
0.05
0
Nonlinear
Third Order
0
0.05
0.1
0.15
0.2
Strains

# $Nb_3Ru_1$

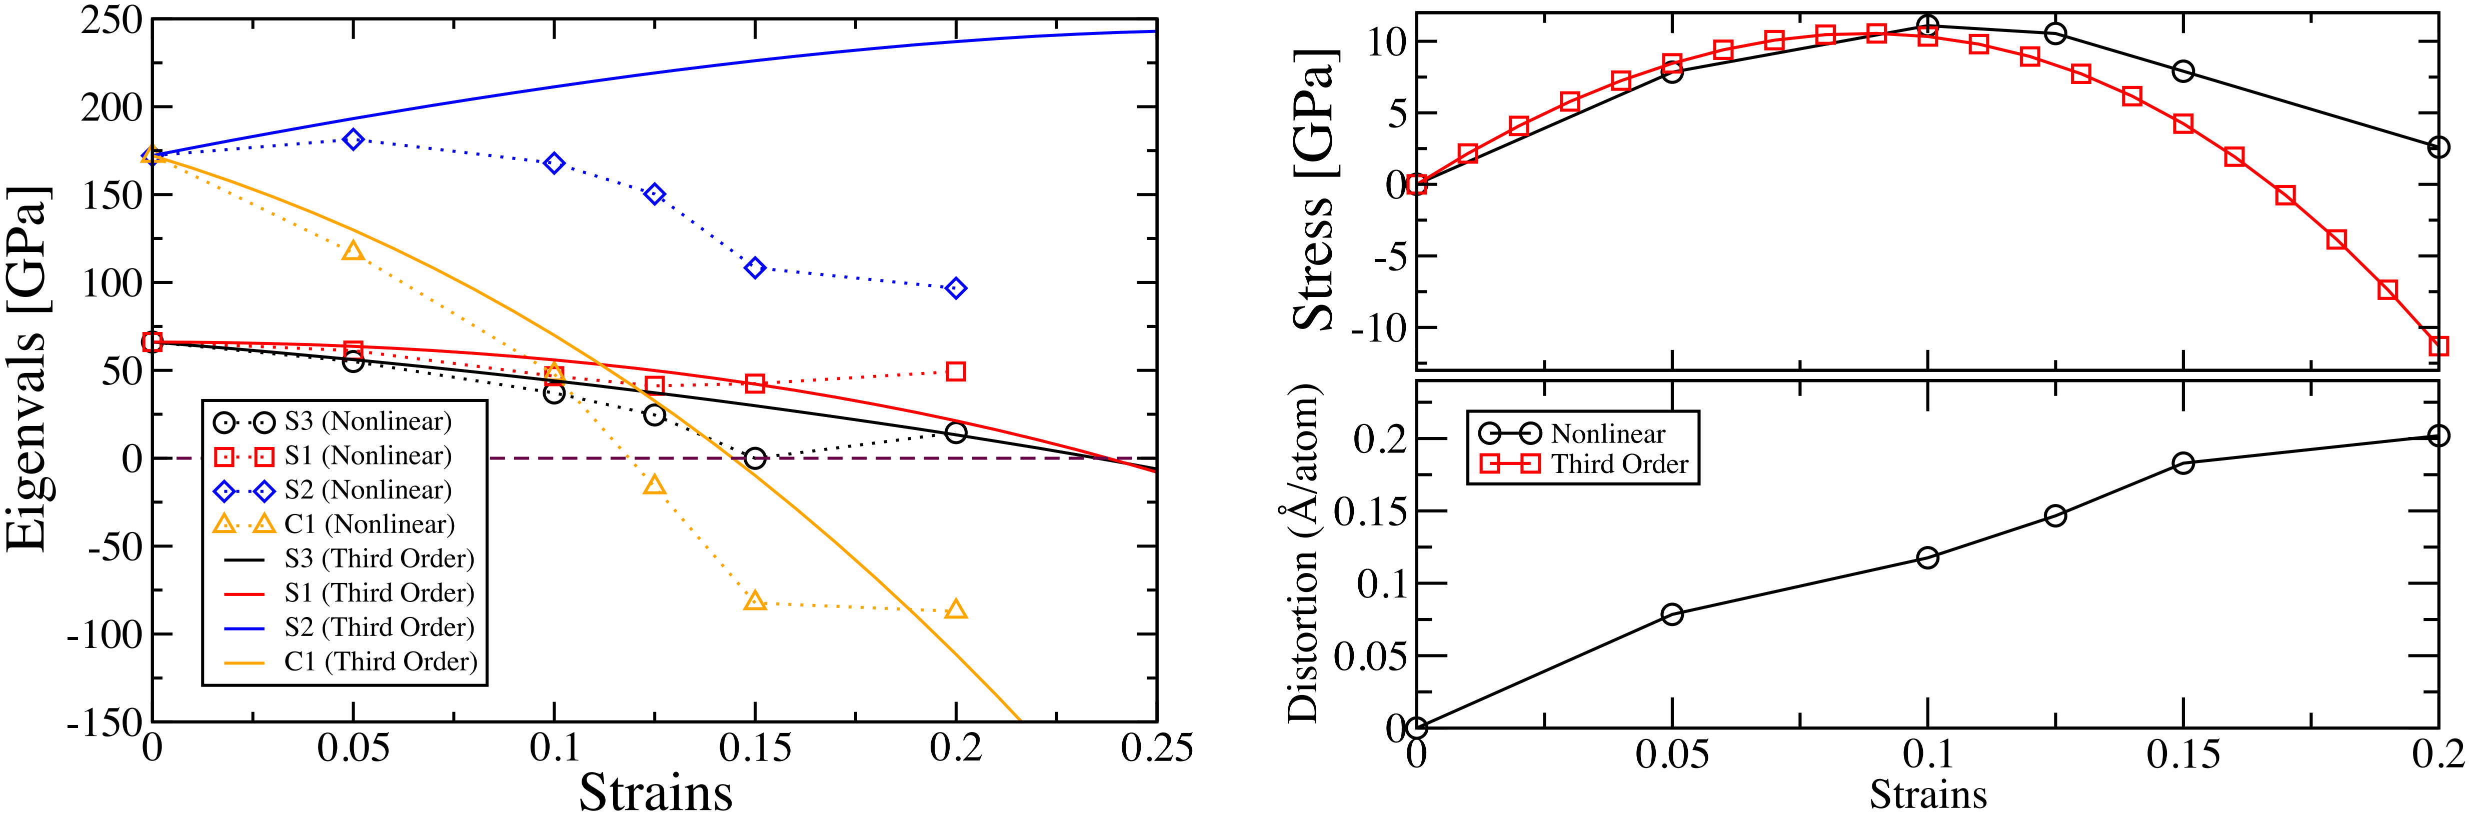

Eigenvals [GPa]
Strains
S3 (Nonlinear)
S1 (Nonlinear)
S2 (Nonlinear)
C1 (Nonlinear)
S3 (Third Order)
S1 (Third Order)
S2 (Third Order)
C1 (Third Order)
Stress [GPa]
Distortion (Å/atom)
Strains
Nonlinear
Third Order

# $Nb_3Si_1$

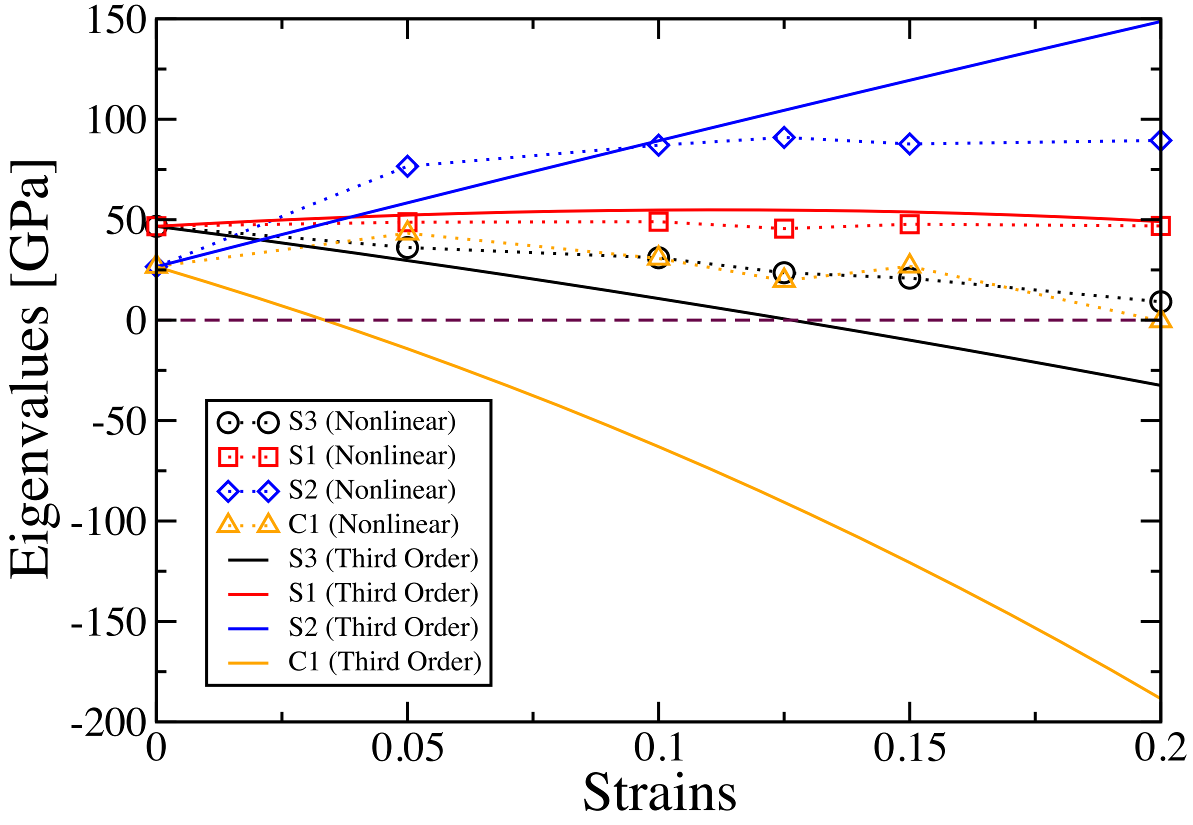
Eigenvalues [GPa]
Strains
S3 (Nonlinear)
S1 (Nonlinear)
S2 (Nonlinear)
C1 (Nonlinear)
S3 (Third Order)
S1 (Third Order)
S2 (Third Order)
C1 (Third Order)

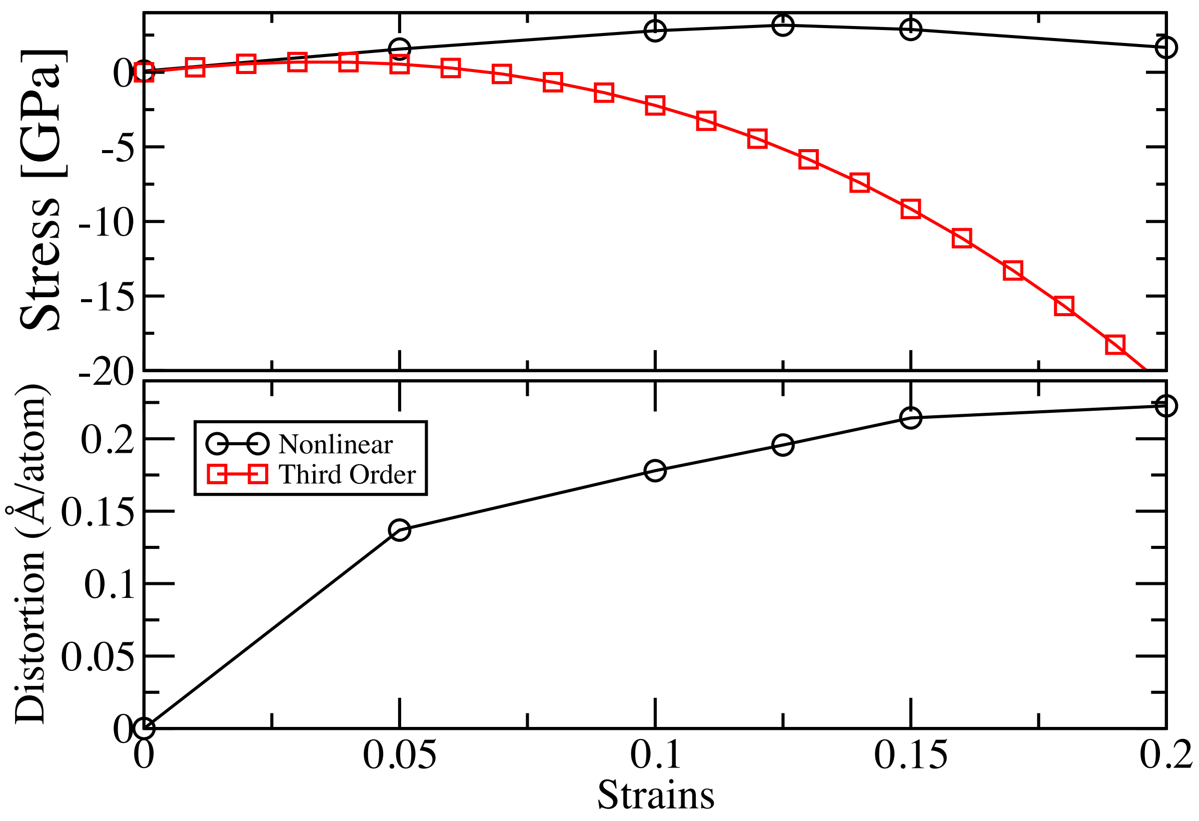
Stress [GPa]
Distortion (Å/atom)
Strains
Nonlinear
Third Order

# $Nb_3Ta_1$

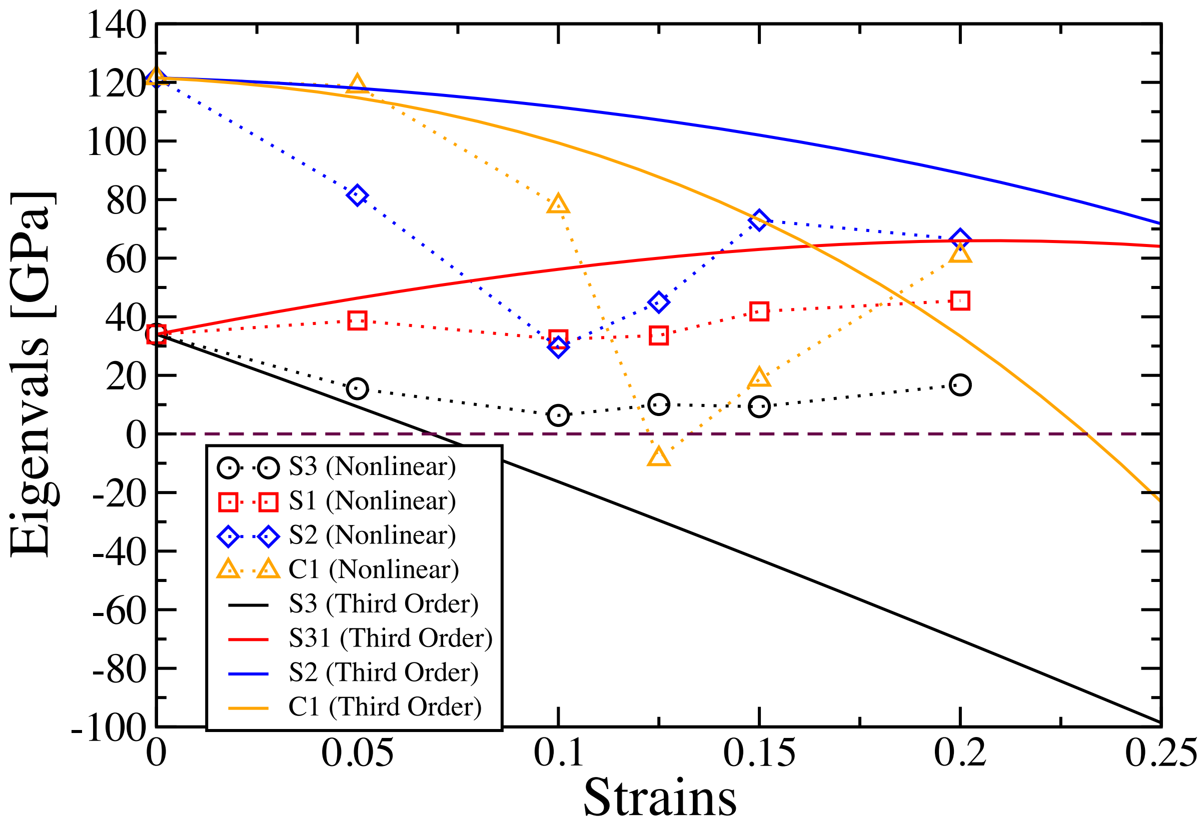

Eigenvals [GPa]
Strains
S3 (Nonlinear)
S1 (Nonlinear)
S2 (Nonlinear)
C1 (Nonlinear)
S3 (Third Order)
S31 (Third Order)
S2 (Third Order)
C1 (Third Order)


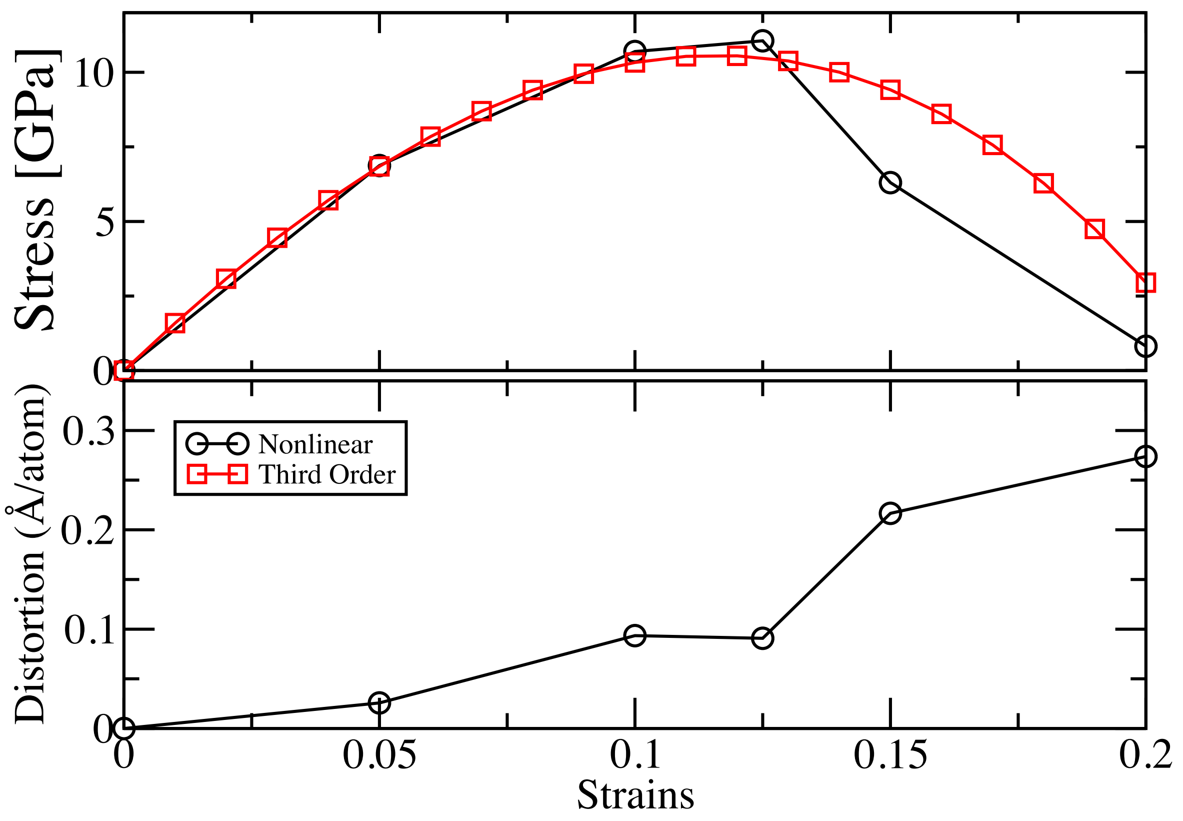

Stress [GPa]
Distortion (Å/atom)
Strains
Nonlinear
Third Order

# $Nb_3Ti_1$

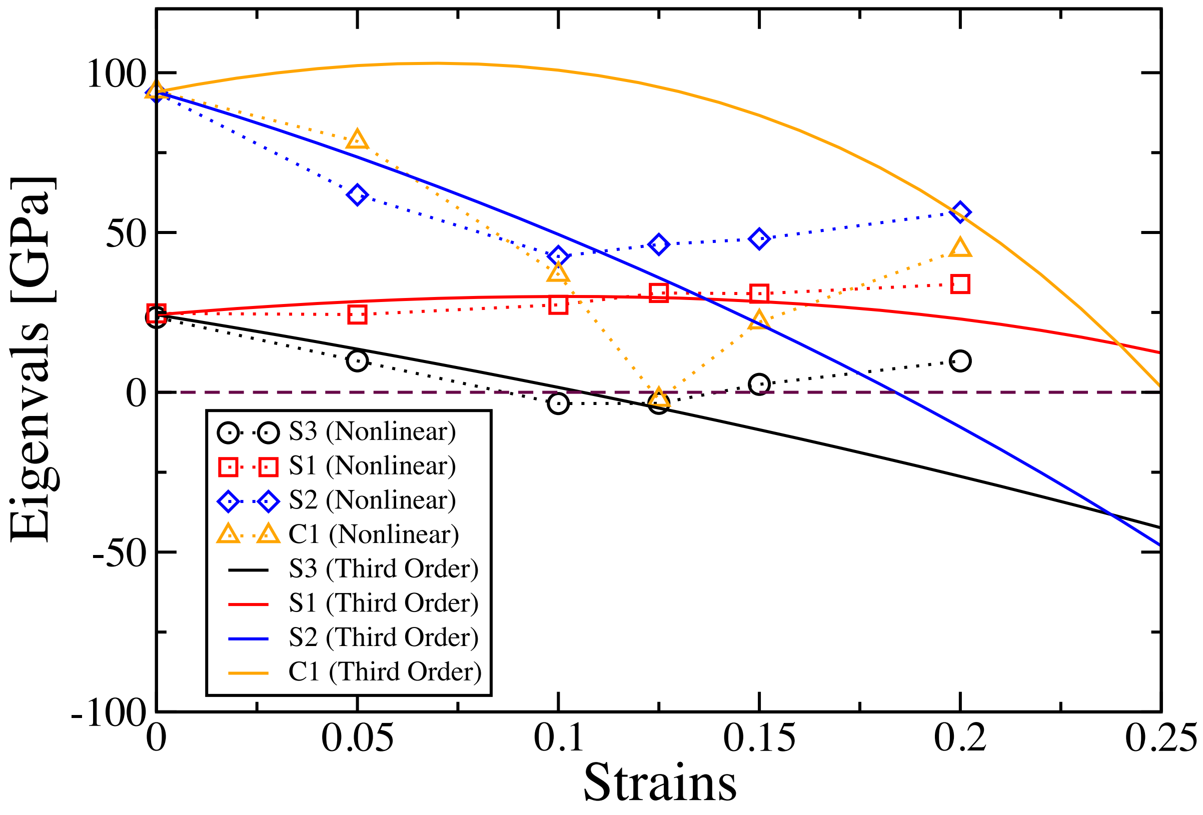

Eigenvals [GPa]
Strains
S3 (Nonlinear)
S1 (Nonlinear)
S2 (Nonlinear)
C1 (Nonlinear)
S3 (Third Order)
S1 (Third Order)
S2 (Third Order)
C1 (Third Order)
100
50
0
-50
-100
0
0.05
0.1
0.15
0.2
0.25


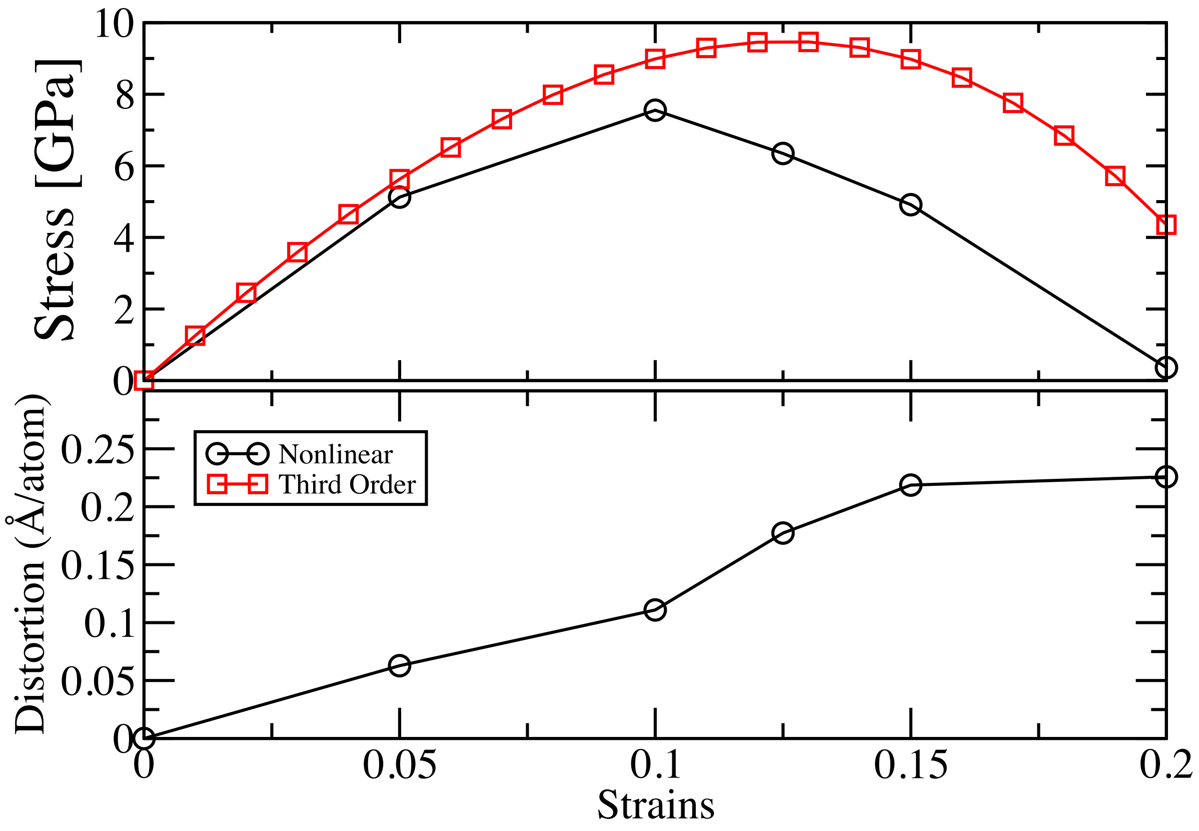

Stress [GPa]
Distortion (Å/atom)
Strains
Nonlinear
Third Order
10
8
6
4
2
0
0.25
0.2
0.15
0.1
0.05
0
0
0.05
0.1
0.15
0.2

# $Nb_3V_1$

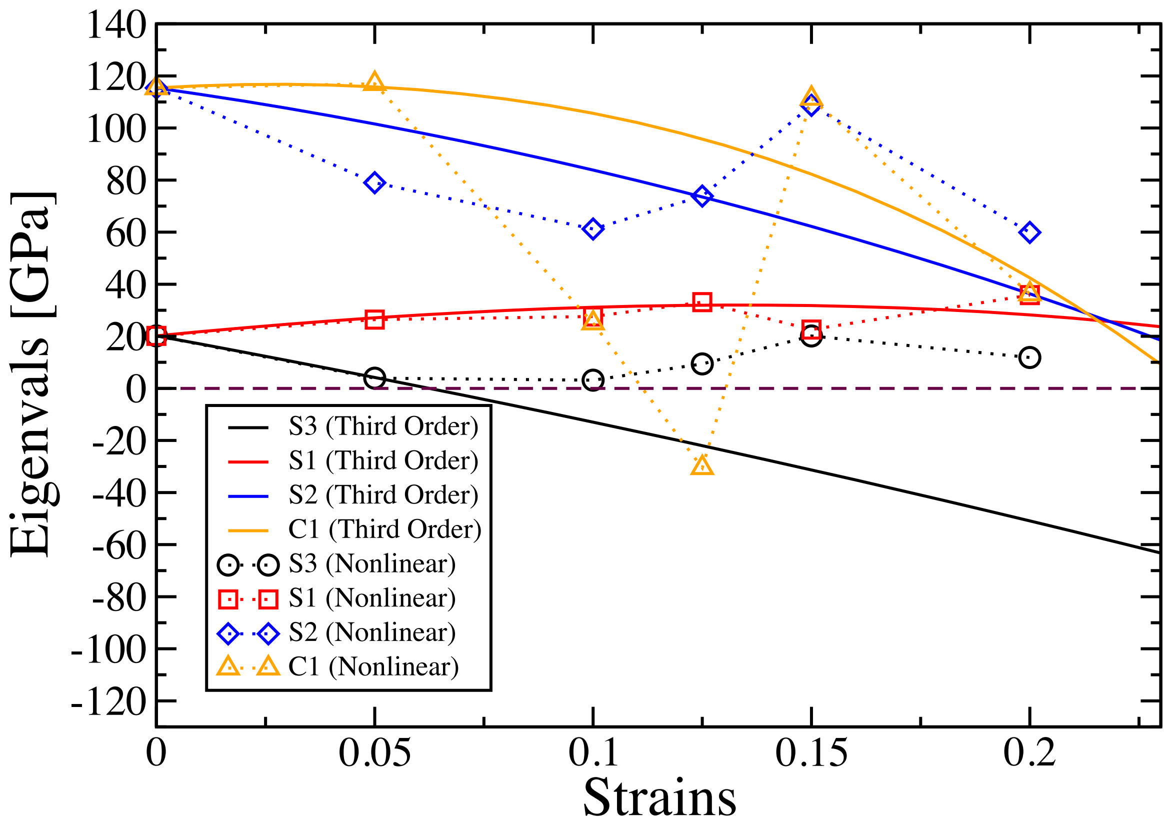

Eigenvals [GPa]
Strains
S3 (Third Order)
S1 (Third Order)
S2 (Third Order)
C1 (Third Order)
S3 (Nonlinear)
S1 (Nonlinear)
S2 (Nonlinear)
C1 (Nonlinear)


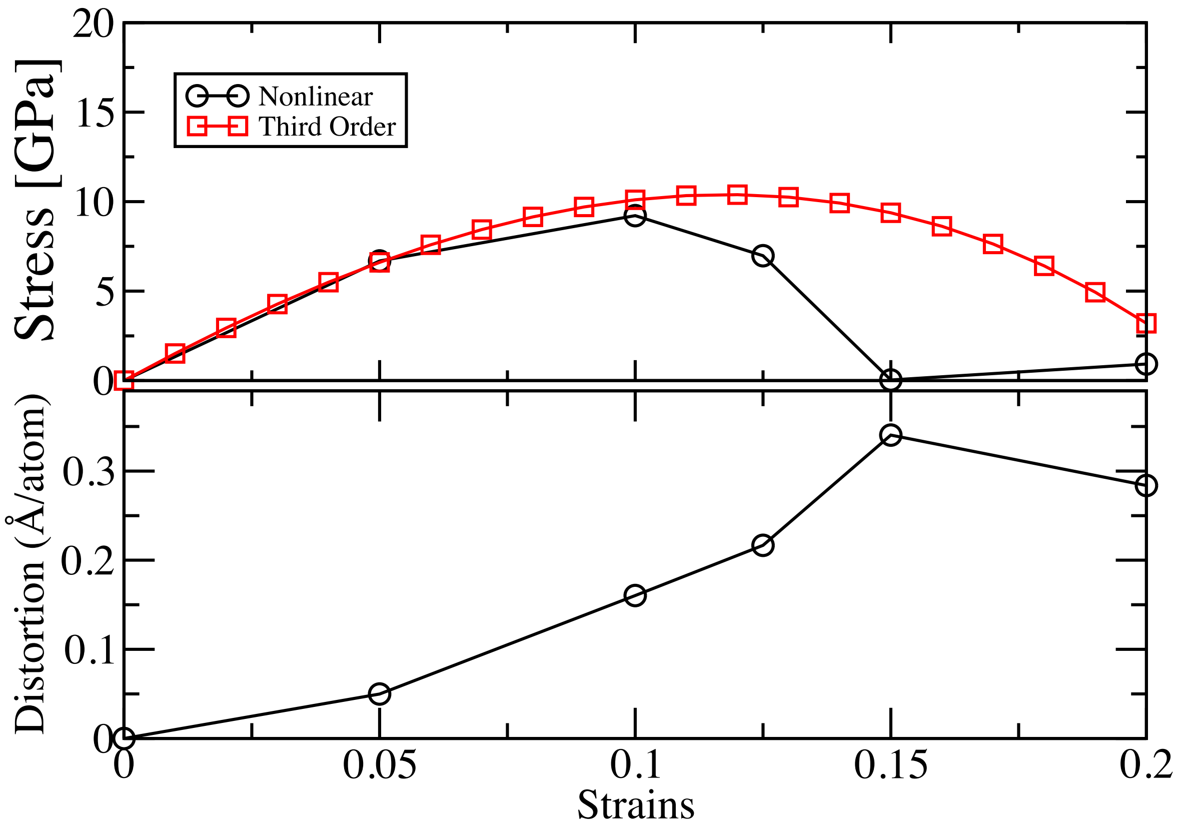

Stress [GPa]
Nonlinear
Third Order
Distortion (Å/atom)
Strains

# $Nb_3W_1$

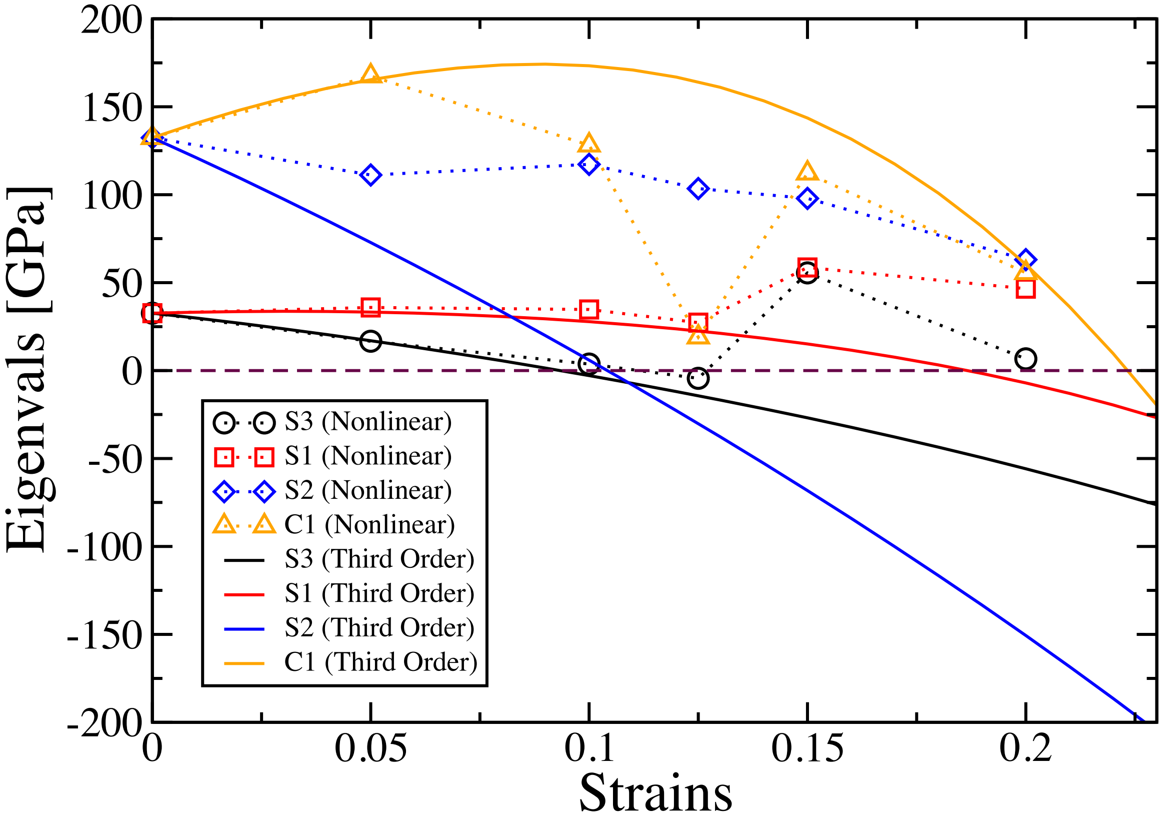

Eigenvals [GPa]
Strains
S3 (Nonlinear)
S1 (Nonlinear)
S2 (Nonlinear)
C1 (Nonlinear)
S3 (Third Order)
S1 (Third Order)
S2 (Third Order)
C1 (Third Order)
200
150
100
50
0
-50
-100
-150
-200
0
0.05
0.1
0.15
0.2


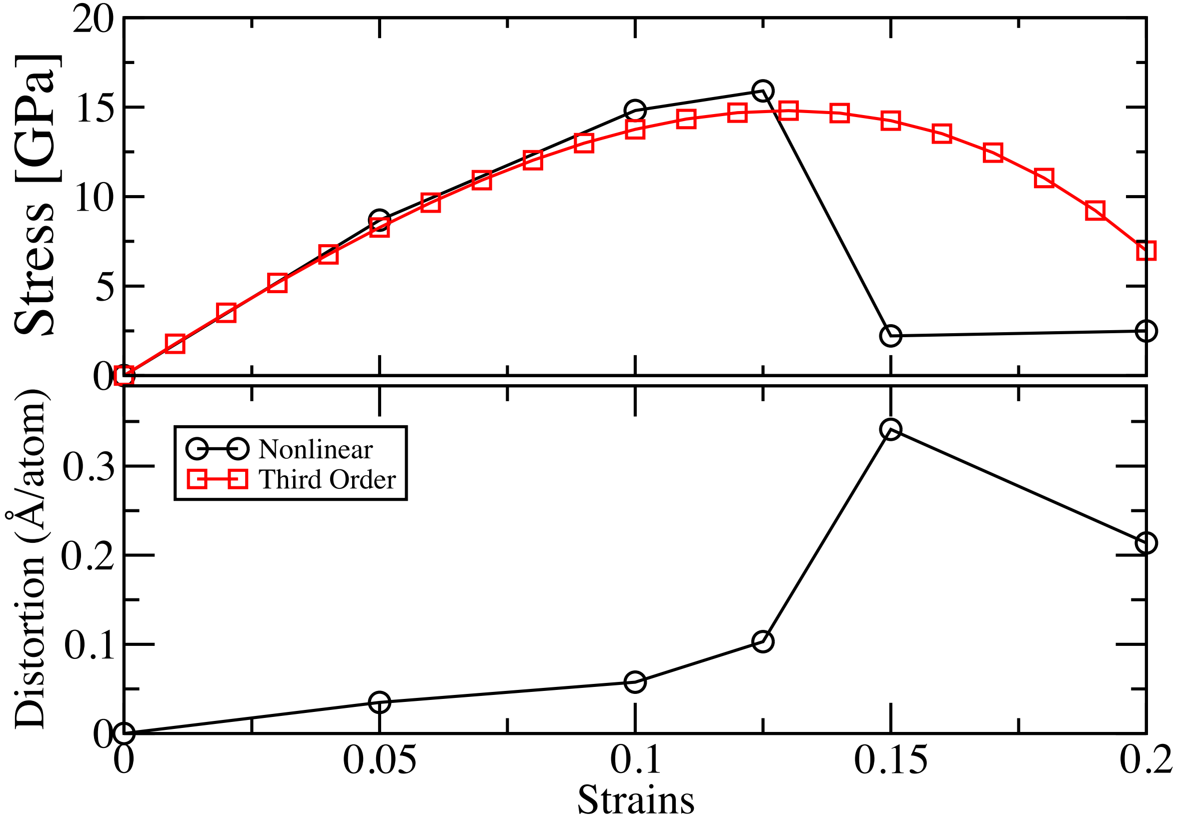

Stress [GPa]
Distortion (Å/atom)
Strains
Nonlinear
Third Order
20
15
10
5
0
0.3
0.2
0.1
0
0
0.05
0.1
0.15
0.2

# $Nb_3Zr_1$

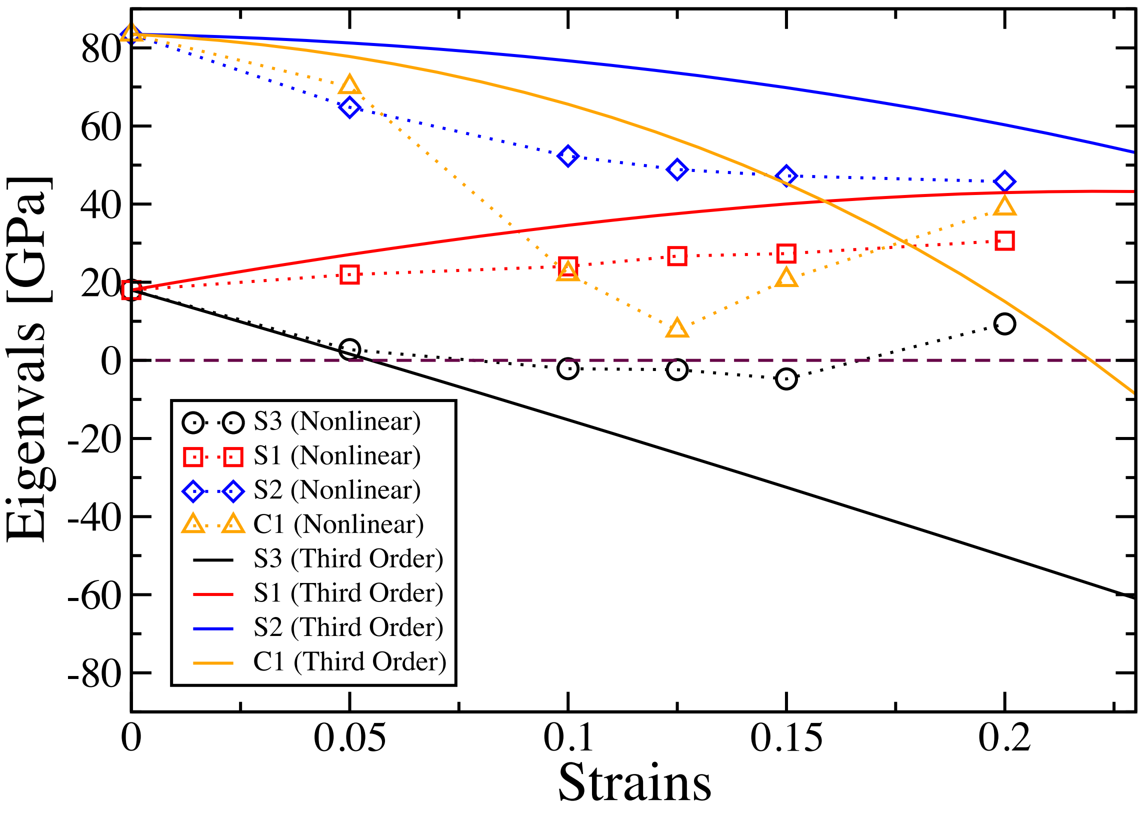
Eigenvals [GPa]
Strains
S3 (Nonlinear)
S1 (Nonlinear)
S2 (Nonlinear)
C1 (Nonlinear)
S3 (Third Order)
S1 (Third Order)
S2 (Third Order)
C1 (Third Order)

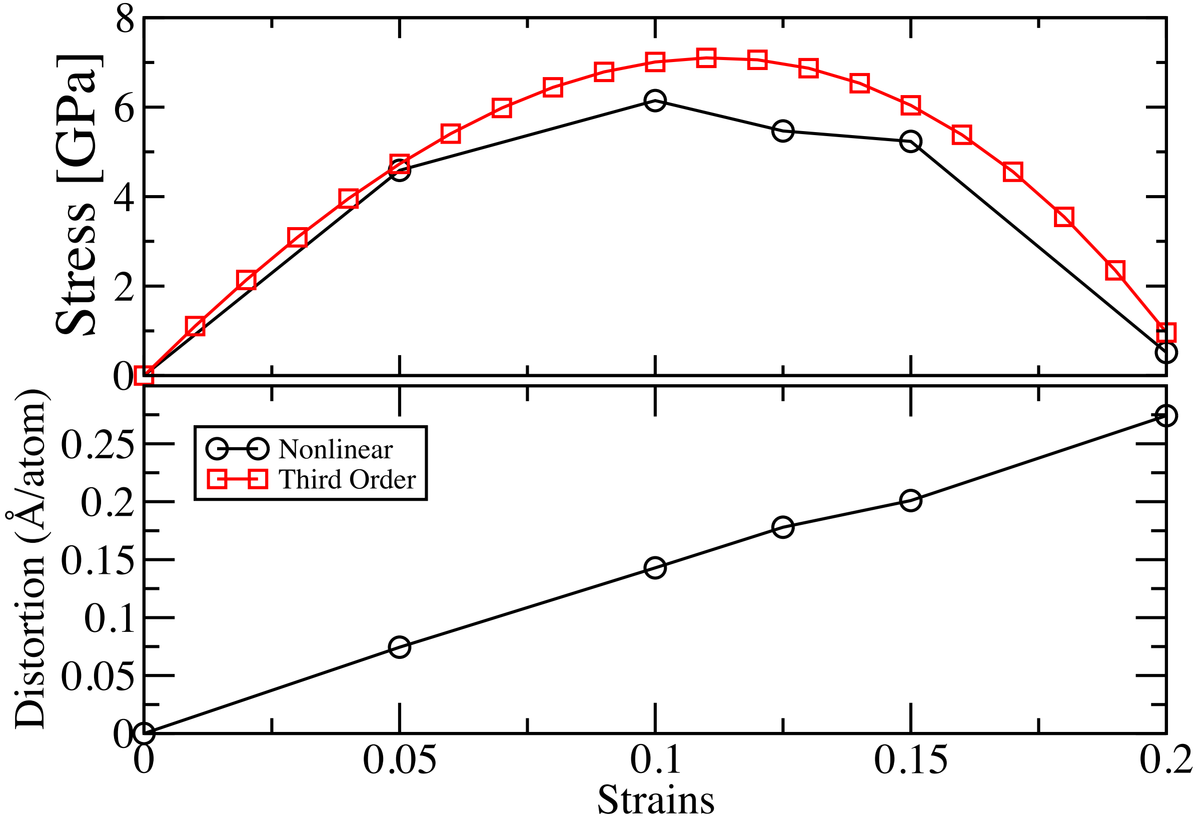
Stress [GPa]
Distortion (Å/atom)
Strains
Nonlinear
Third Order

# Refractory Metal Quaternaries

Wallace tensor eigenvalues, stress, lattice distortion

# CrMoNbV

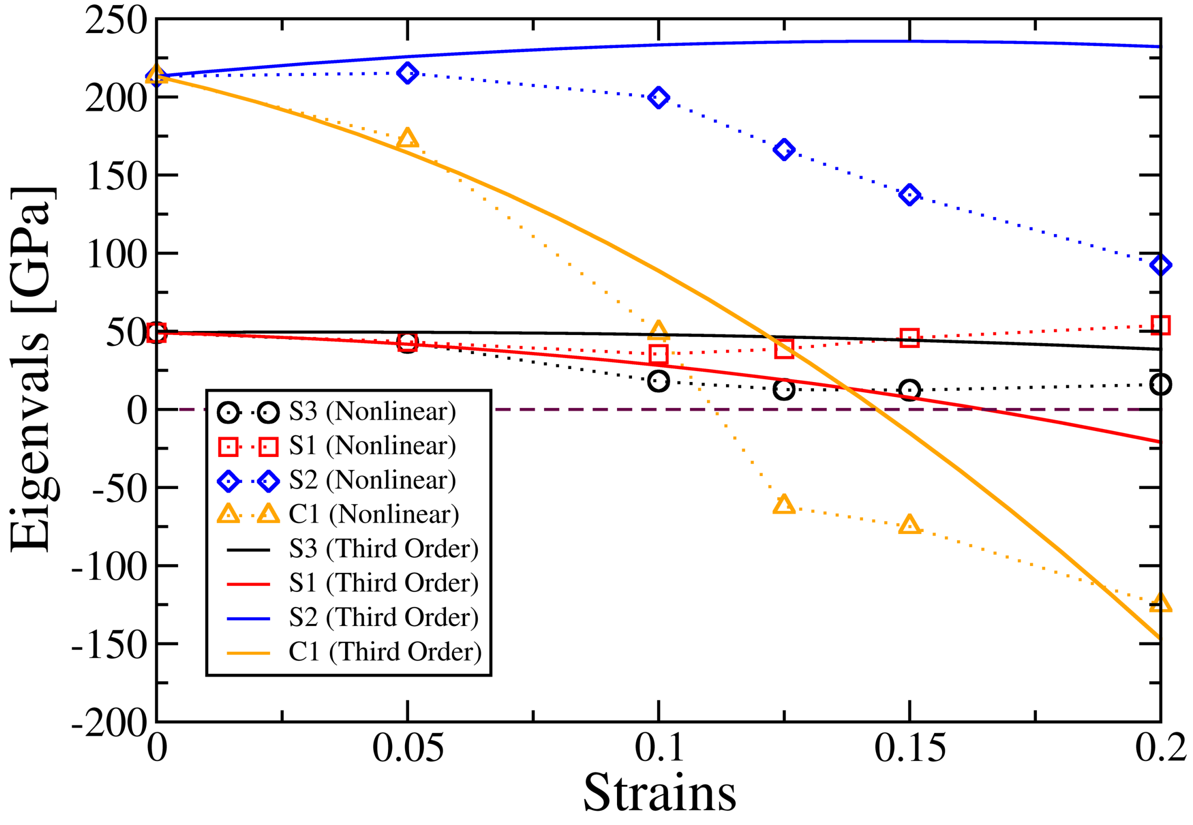

Eigenvals [GPa]
Strains
S3 (Nonlinear)
S1 (Nonlinear)
S2 (Nonlinear)
C1 (Nonlinear)
S3 (Third Order)
S1 (Third Order)
S2 (Third Order)
C1 (Third Order)


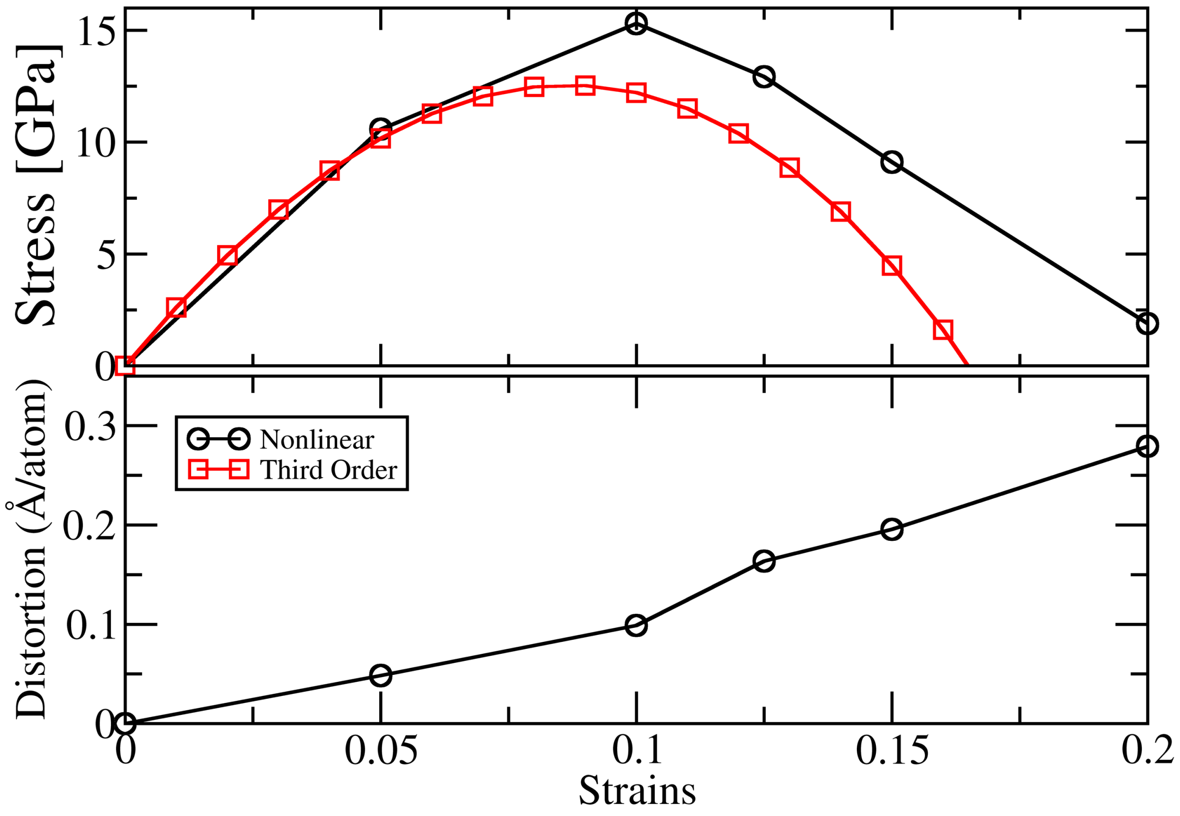

Stress [GPa]
Distortion (Å/atom)
Strains
Nonlinear
Third Order

# CrMoNbW

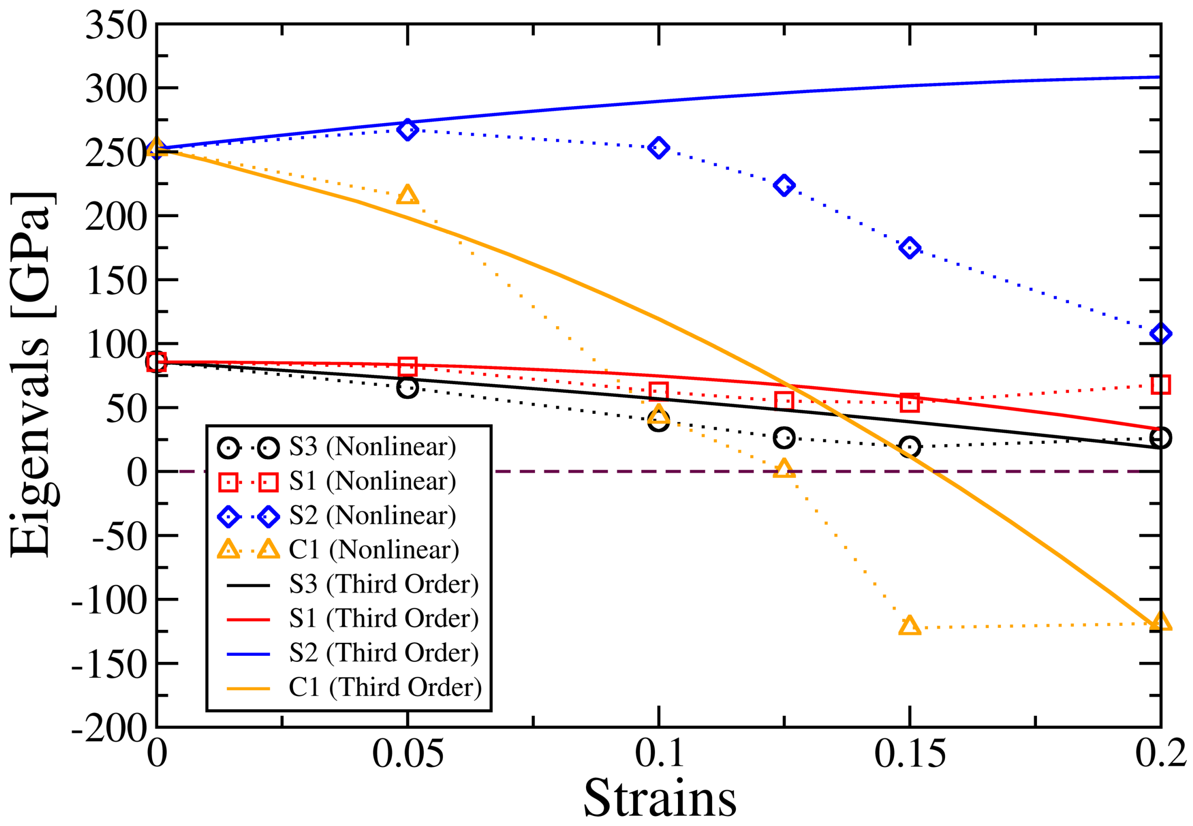
Eigenvals [GPa]
Strains
S3 (Nonlinear)
S1 (Nonlinear)
S2 (Nonlinear)
C1 (Nonlinear)
S3 (Third Order)
S1 (Third Order)
S2 (Third Order)
C1 (Third Order)

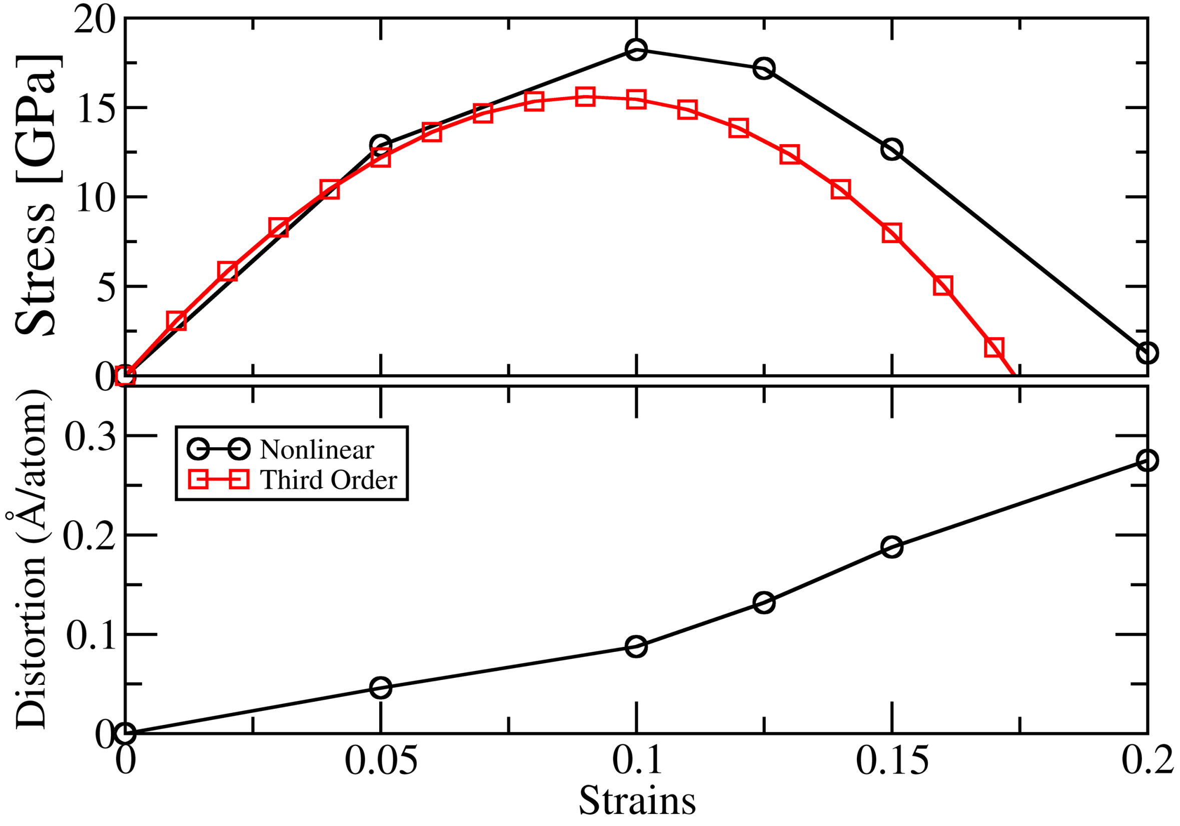
Stress [GPa]
Distortion (Å/atom)
Nonlinear
Third Order
Strains

# AlMoNbTi

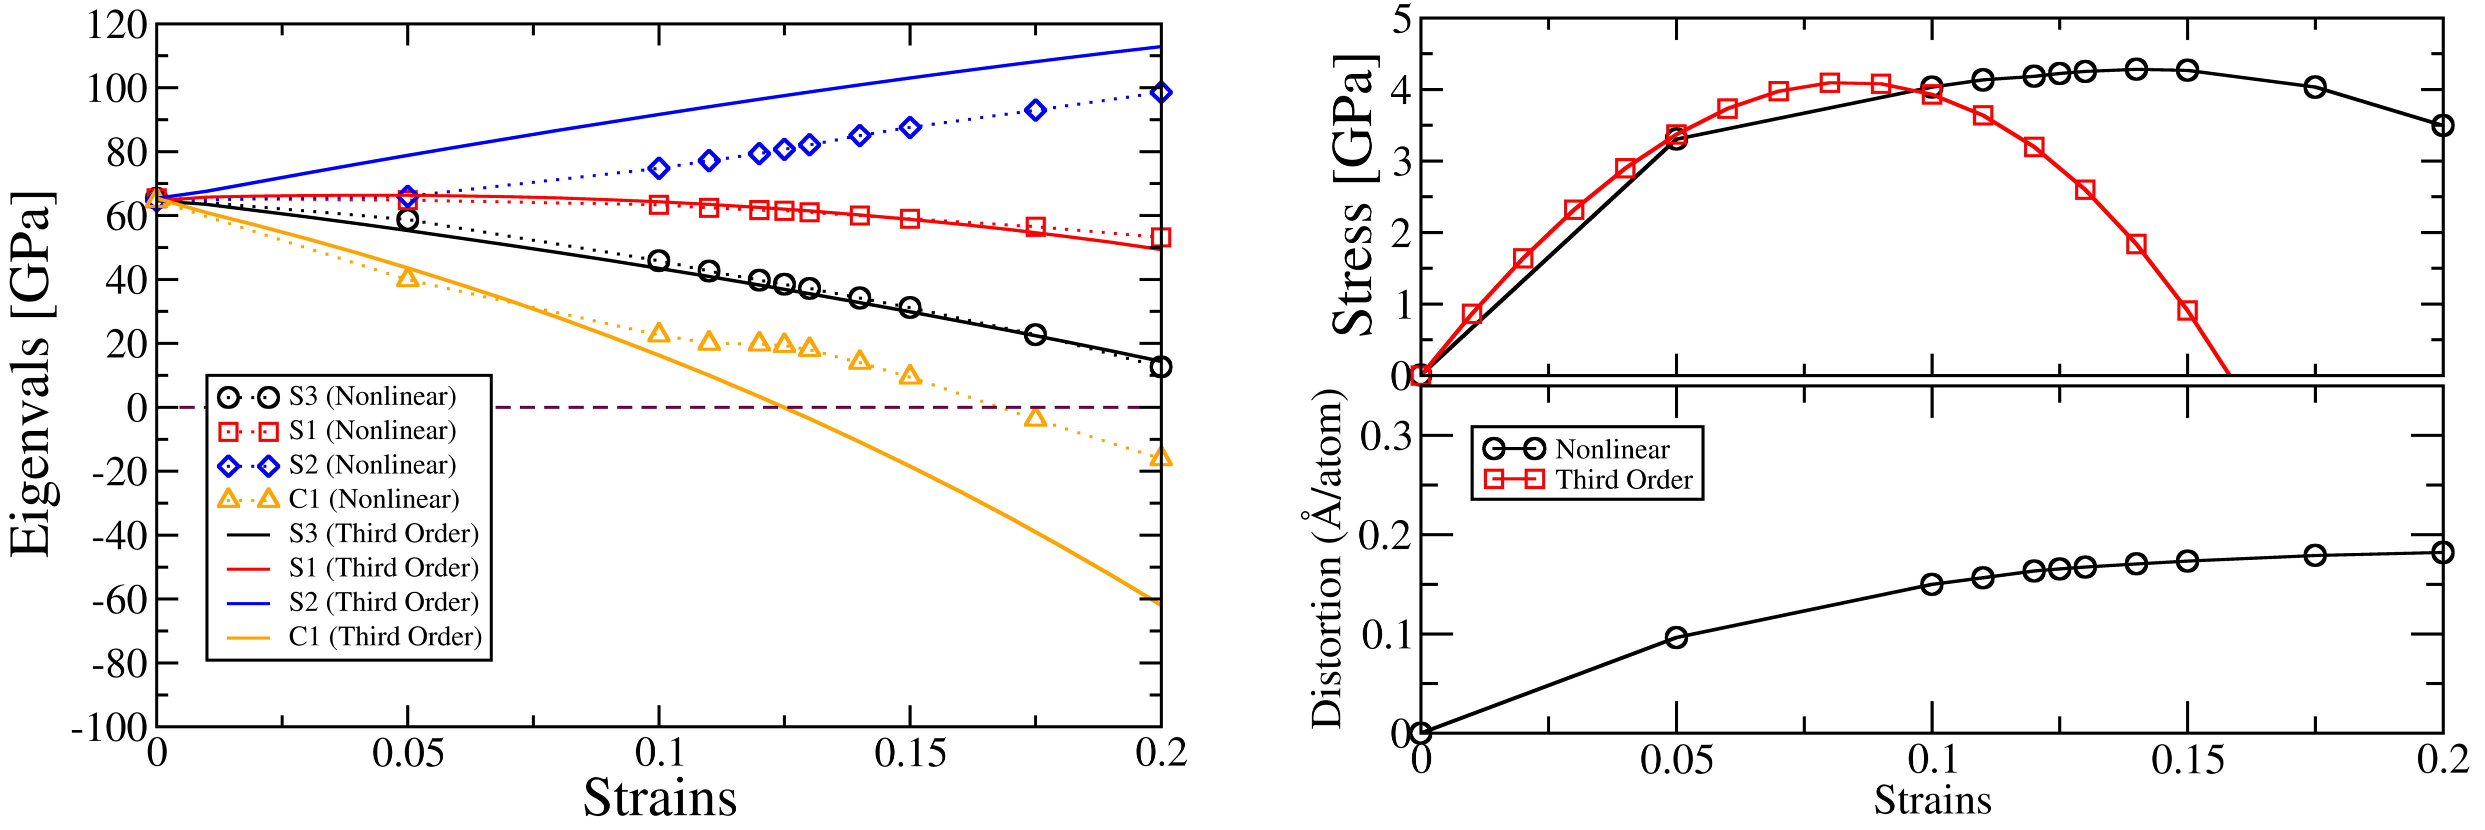

Eigenvals [GPa]
120
100
80
60
40
20
0
-20
-40
-60
-80
-100
0
0.05
0.1
0.15
0.2
Strains
S3 (Nonlinear)
S1 (Nonlinear)
S2 (Nonlinear)
C1 (Nonlinear)
S3 (Third Order)
S1 (Third Order)
S2 (Third Order)
C1 (Third Order)
Stress [GPa]
5
4
3
2
1
0
Distortion (Å/atom)
0.3
0.2
0.1
0
Nonlinear
Third Order
0
0.05
0.1
0.15
0.2
Strains

# CrMoNbTi

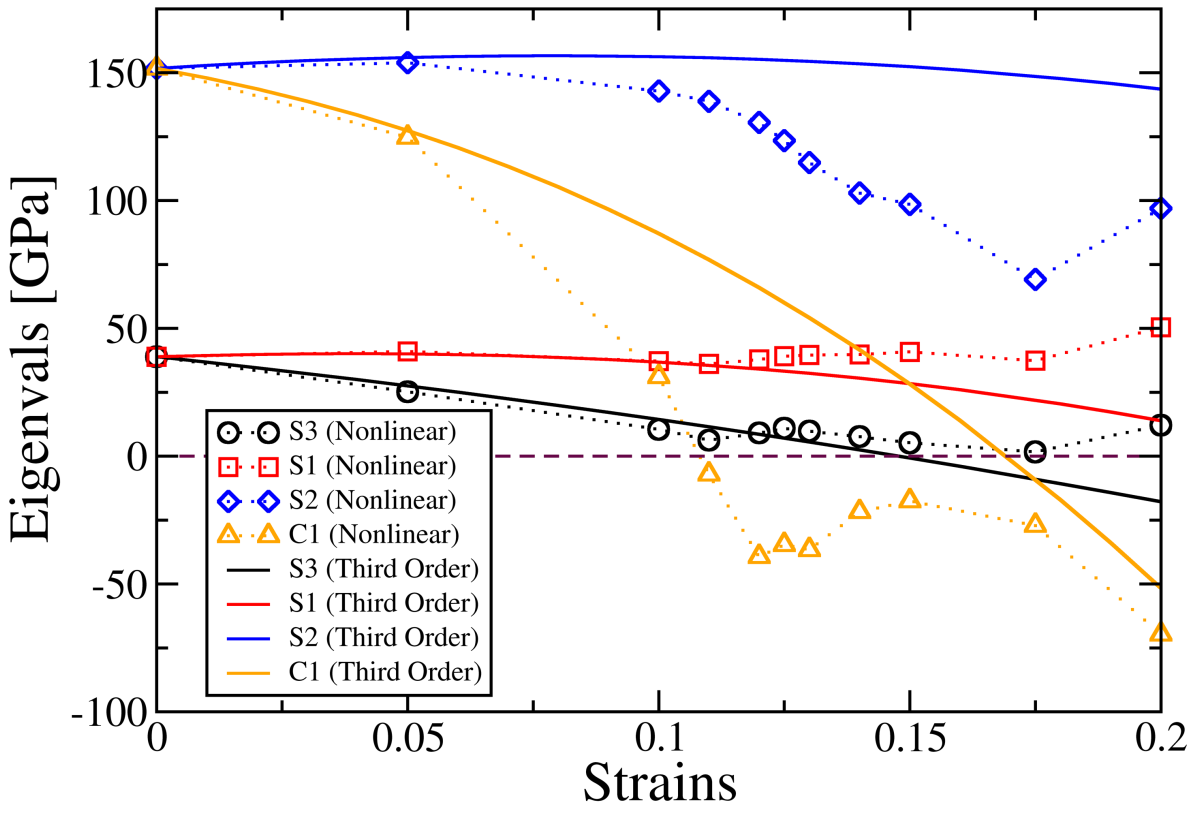

Eigenvals [GPa]
150
100
50
0
-50
-100
0
0.05
0.1
0.15
0.2
Strains
S3 (Nonlinear)
S1 (Nonlinear)
S2 (Nonlinear)
C1 (Nonlinear)
S3 (Third Order)
S1 (Third Order)
S2 (Third Order)
C1 (Third Order)


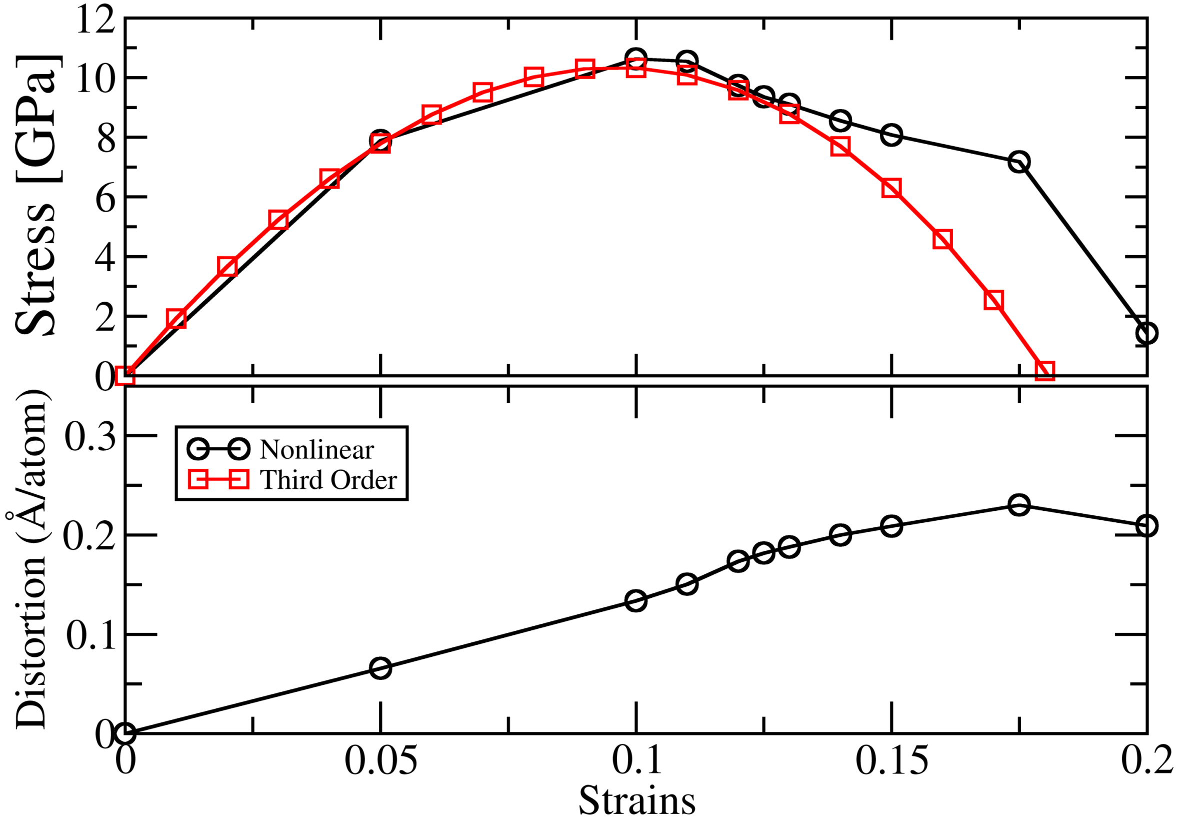

Stress [GPa]
12
10
8
6
4
2
0
Distortion (Å/atom)
0.3
0.2
0.1
0
0
0.05
0.1
0.15
0.2
Strains
Nonlinear
Third Order

# MoNbSiTi

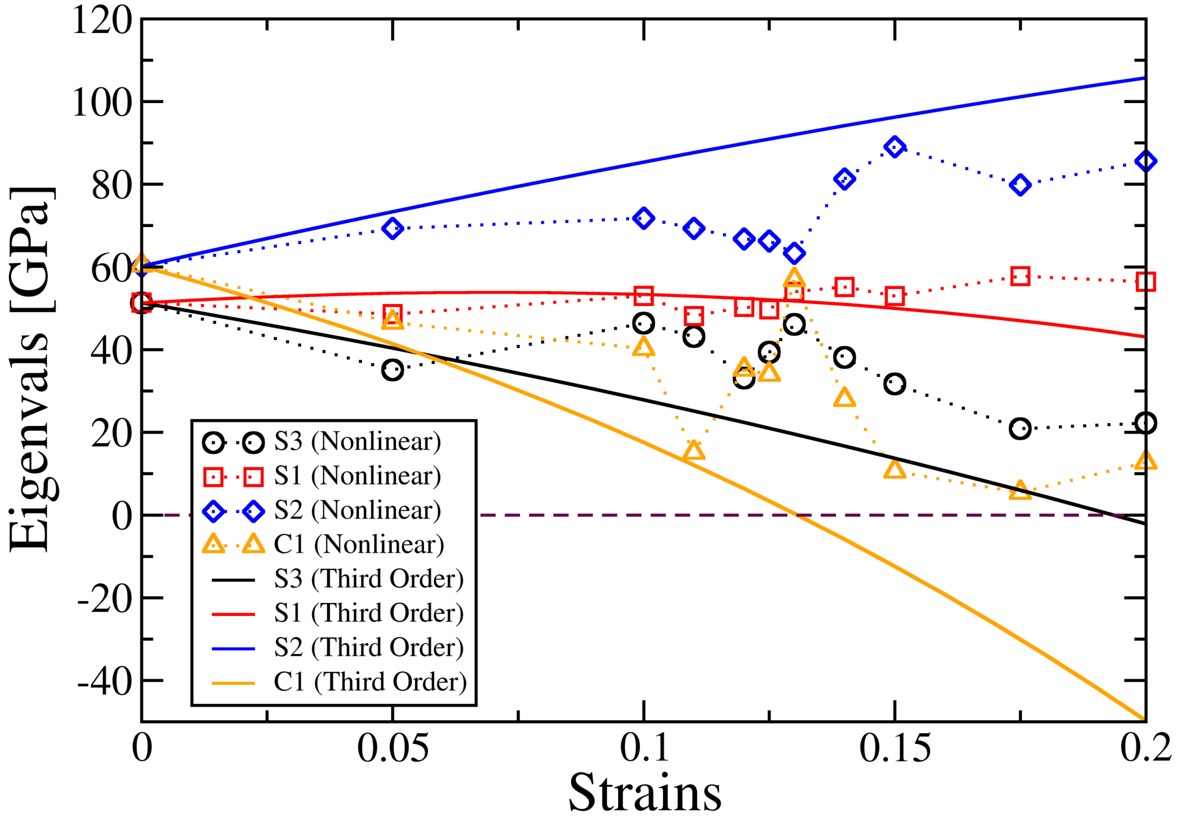

Eigenvals [GPa]
Strains
S3 (Nonlinear)
S1 (Nonlinear)
S2 (Nonlinear)
C1 (Nonlinear)
S3 (Third Order)
S1 (Third Order)
S2 (Third Order)
C1 (Third Order)


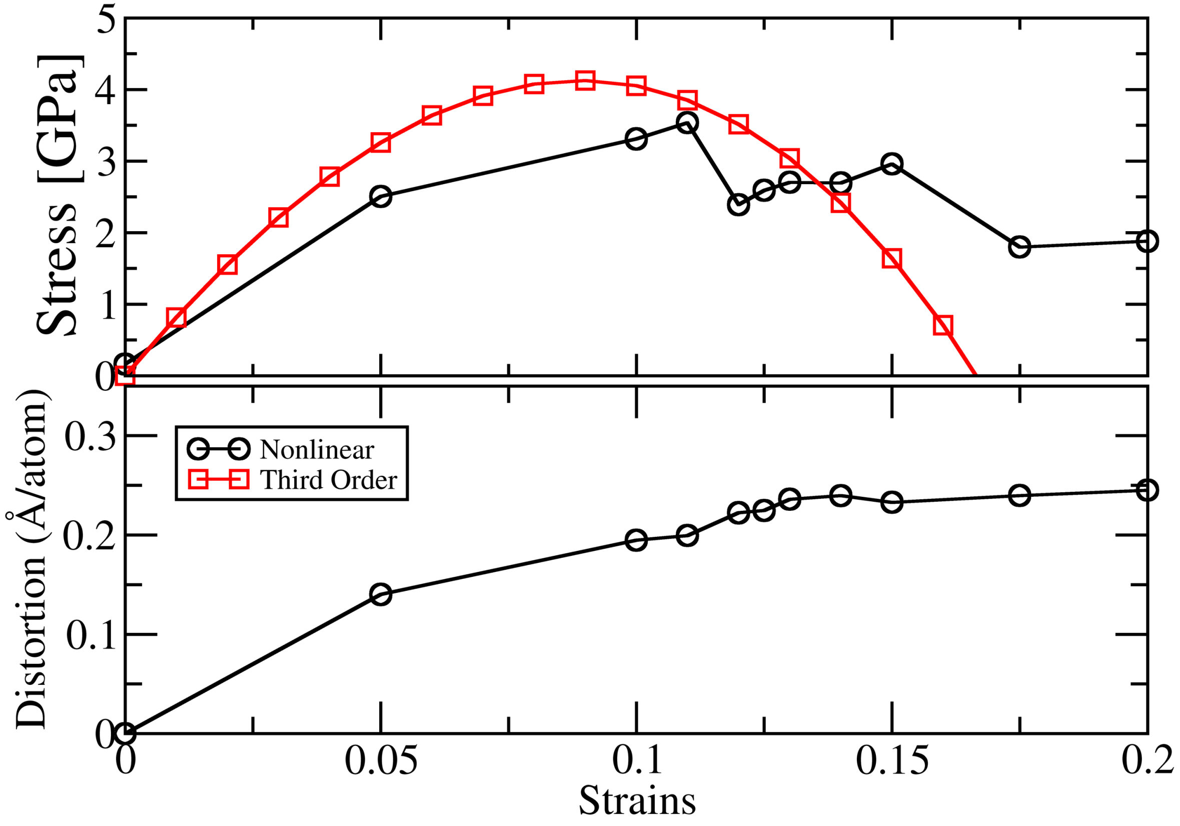

Stress [GPa]
Distortion (Å/atom)
Strains
Nonlinear
Third Order

# MoNbTaTi

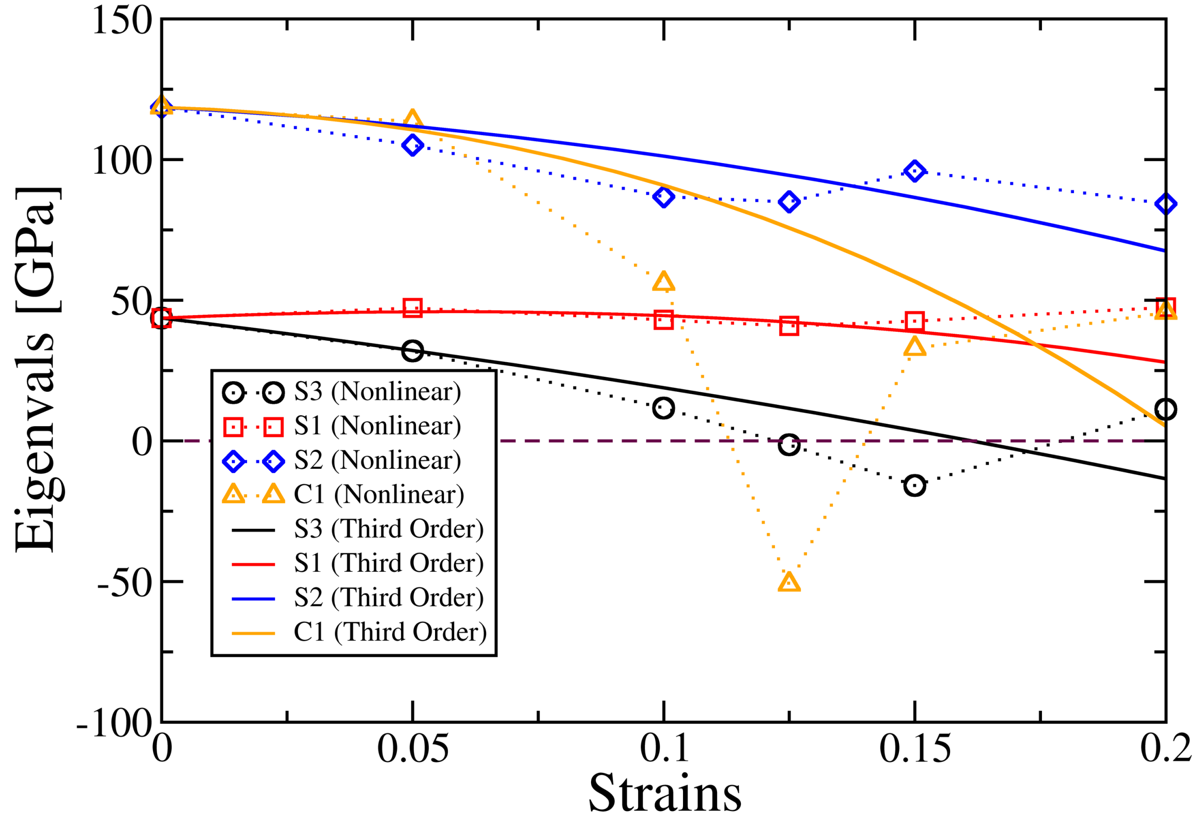

150
100
50
0
-50
-100
0
0.05
0.1
0.15
0.2
Eigenvals [GPa]
Strains
S3 (Nonlinear)
S1 (Nonlinear)
S2 (Nonlinear)
C1 (Nonlinear)
S3 (Third Order)
S1 (Third Order)
S2 (Third Order)
C1 (Third Order)


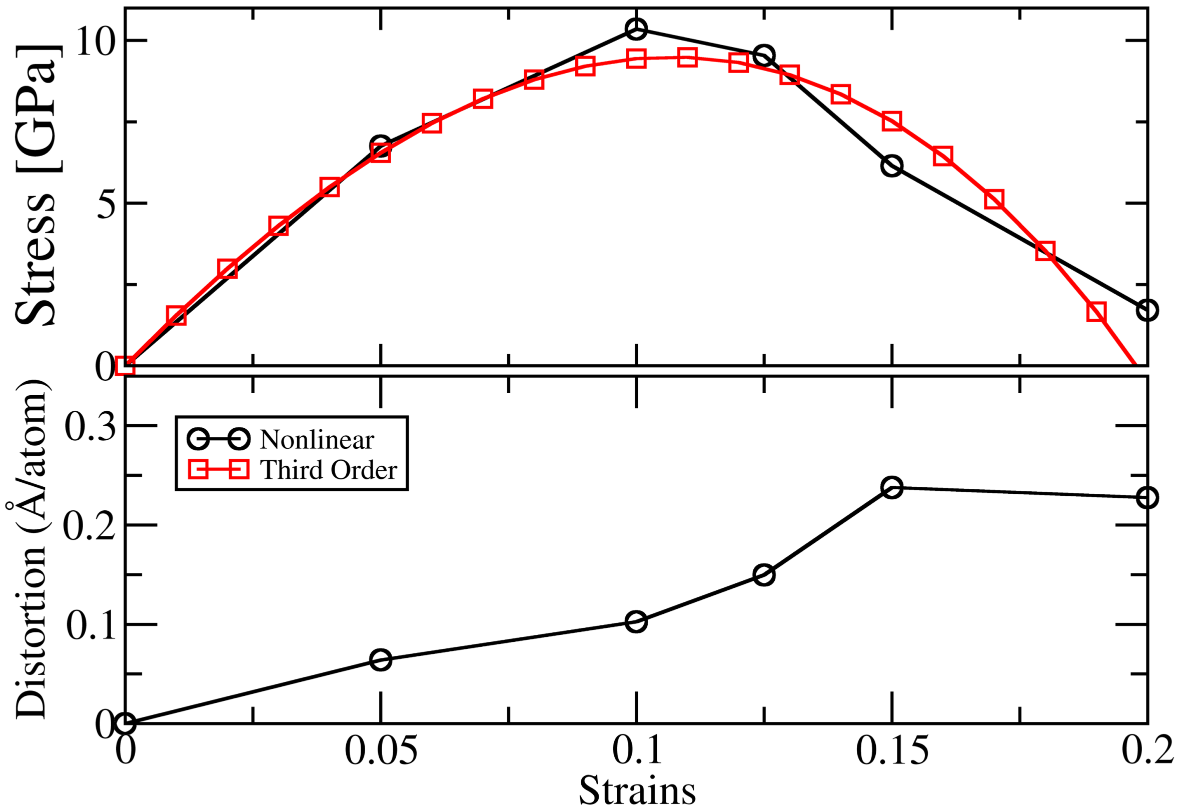

Stress [GPa]
10
5
0
Distortion (Å/atom)
0.3
0.2
0.1
0
0
0.05
0.1
0.15
0.2
Strains
Nonlinear
Third Order

# HfMoNbTi

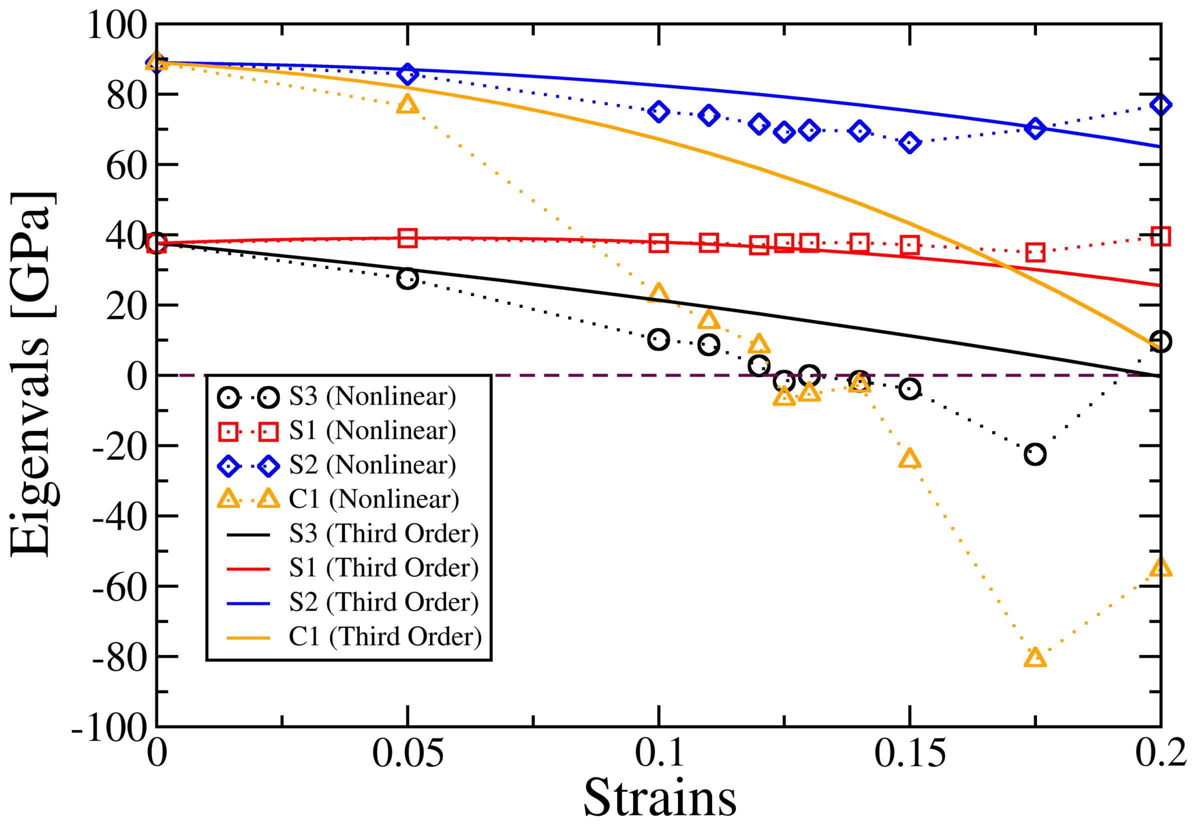

Eigenvals [GPa]
Strains
S3 (Nonlinear)
S1 (Nonlinear)
S2 (Nonlinear)
C1 (Nonlinear)
S3 (Third Order)
S1 (Third Order)
S2 (Third Order)
C1 (Third Order)


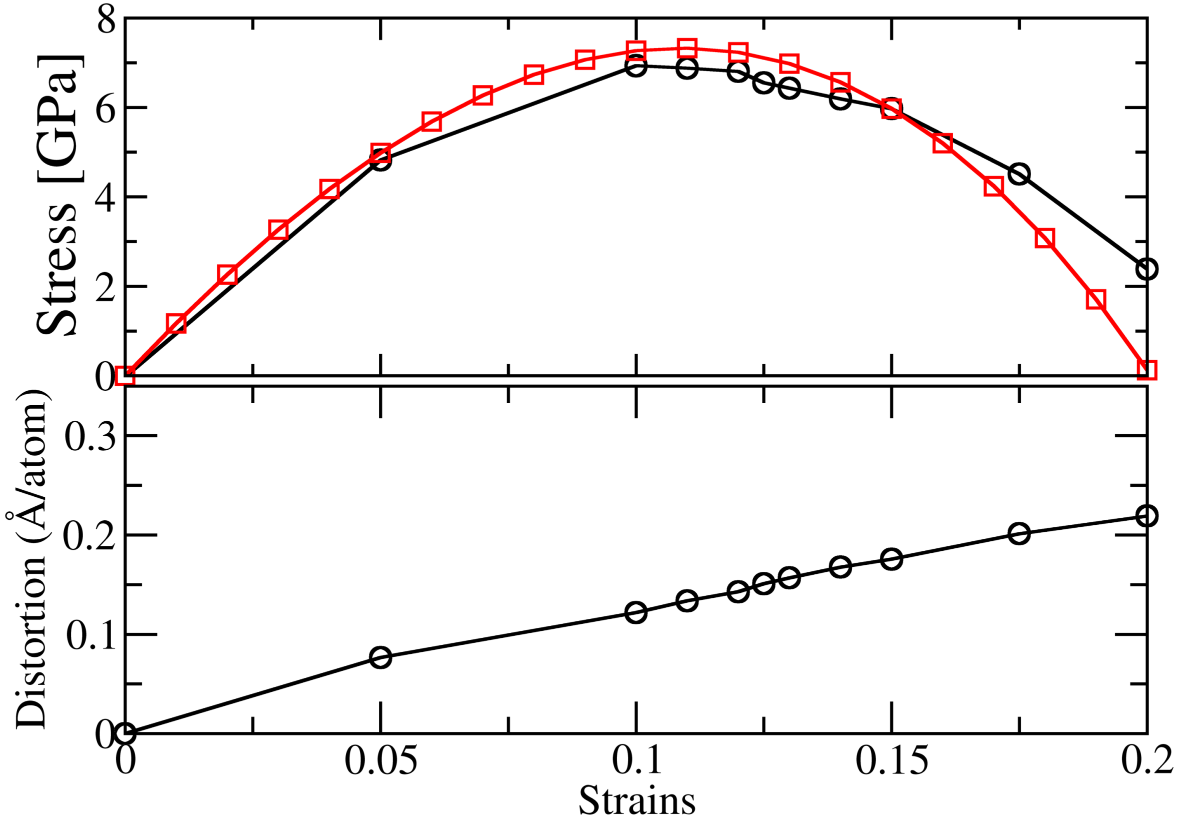

Stress [GPa]
Distortion (Å/atom)
Strains

# MoNbReTi

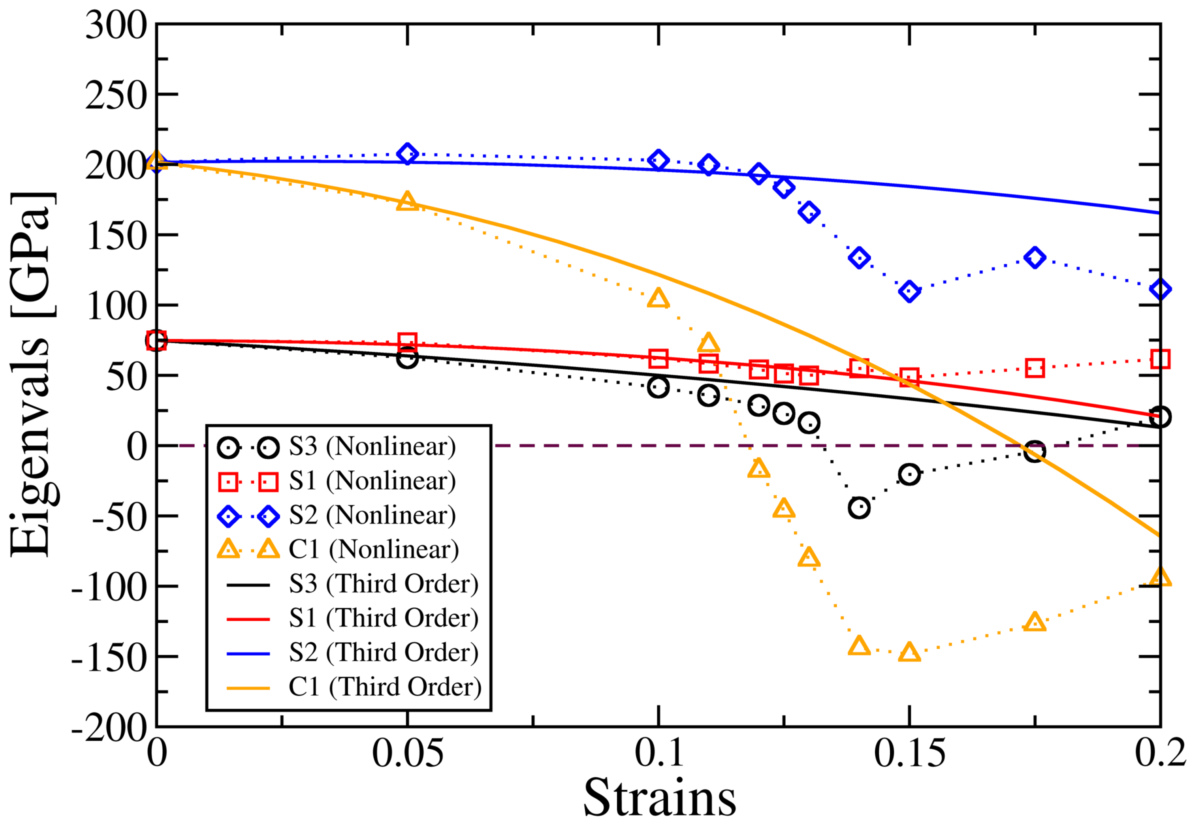

Eigenvals [GPa]
Strains
S3 (Nonlinear)
S1 (Nonlinear)
S2 (Nonlinear)
C1 (Nonlinear)
S3 (Third Order)
S1 (Third Order)
S2 (Third Order)
C1 (Third Order)


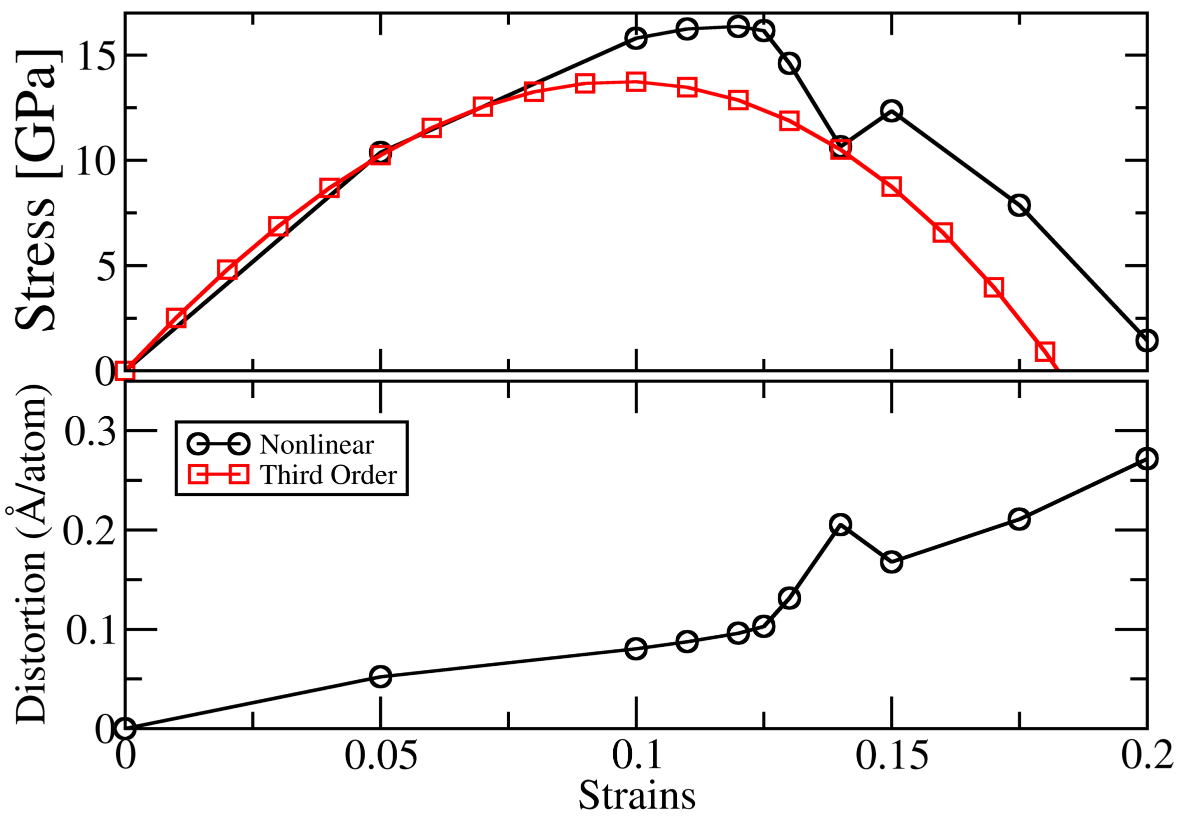

Stress [GPa]
Distortion (Å/atom)
Nonlinear
Third Order
Strains

# MoNbRuTi

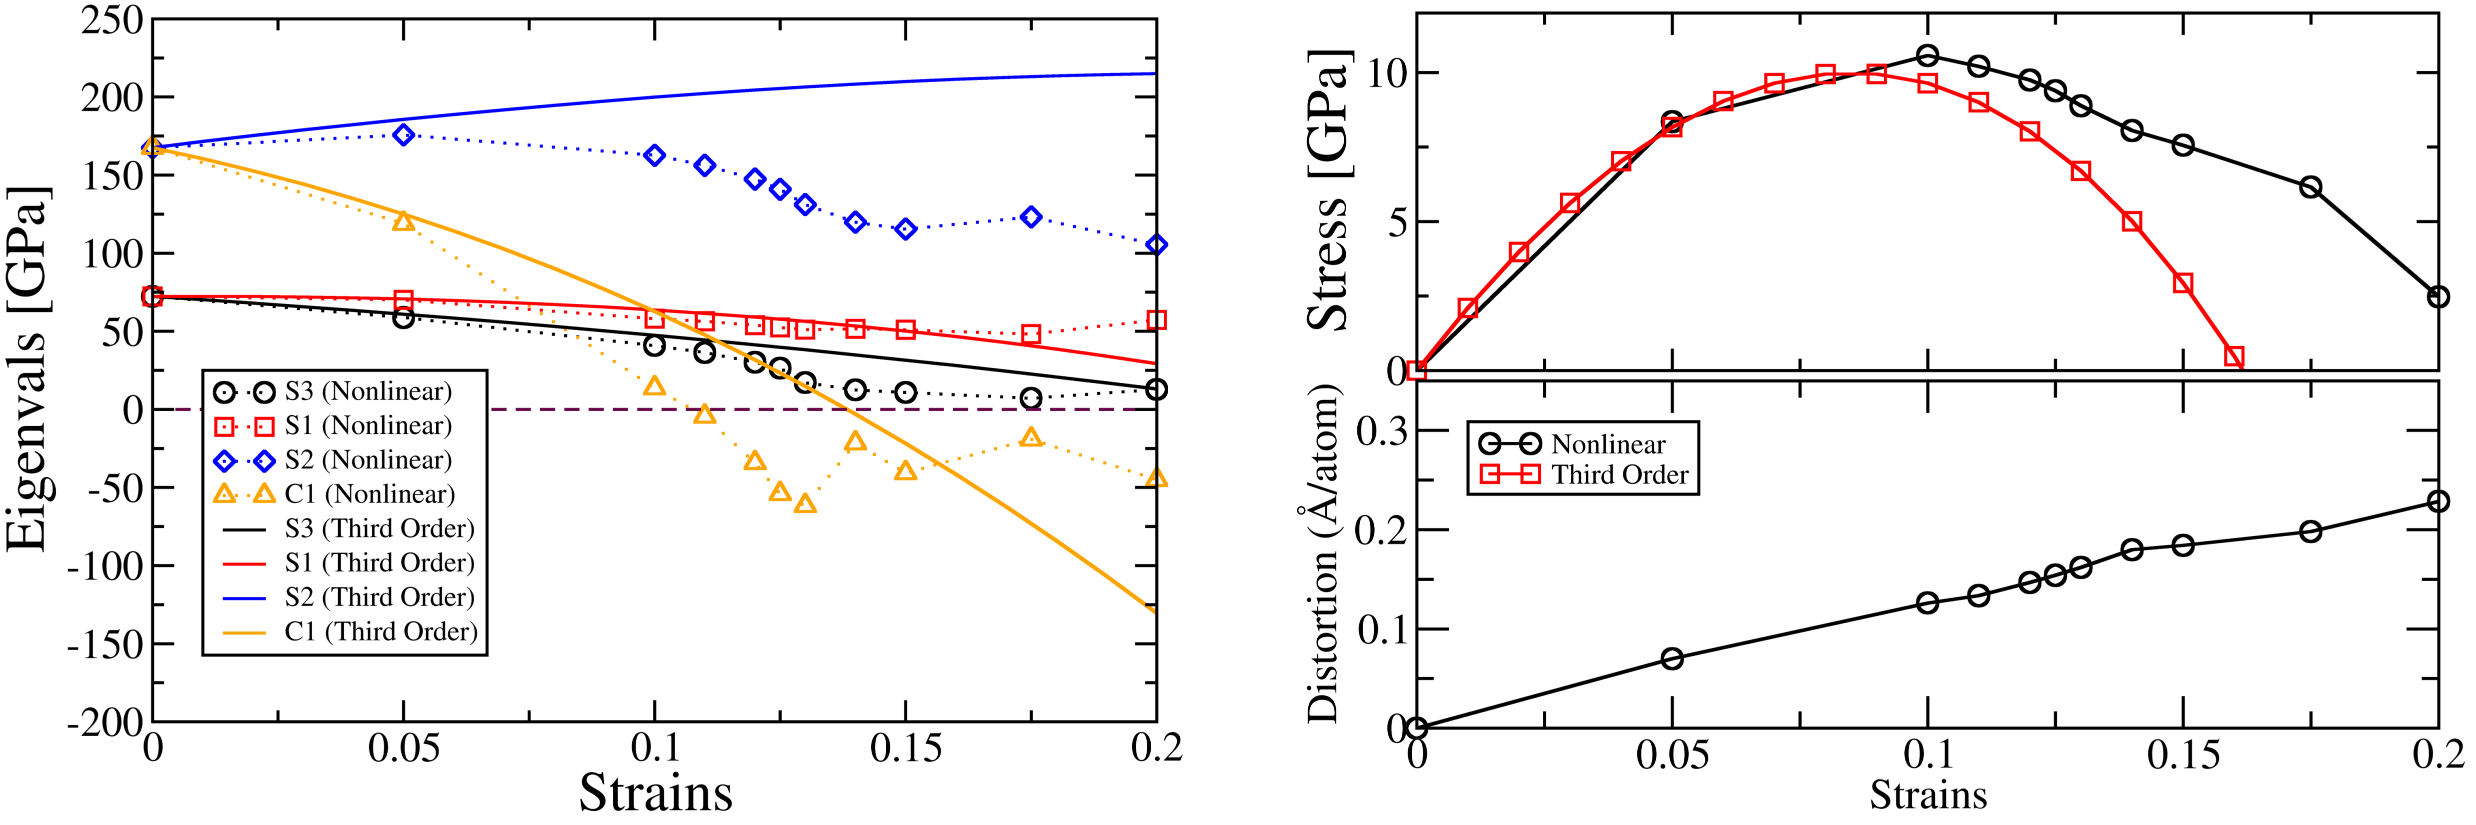

Eigenvals [GPa]
250
200
150
100
50
0
-50
-100
-150
-200
0
0.05
0.1
0.15
0.2
Strains
S3 (Nonlinear)
S1 (Nonlinear)
S2 (Nonlinear)
C1 (Nonlinear)
S3 (Third Order)
S1 (Third Order)
S2 (Third Order)
C1 (Third Order)
Stress [GPa]
10
5
0
Distortion (Å/atom)
0.3
0.2
0.1
0
Nonlinear
Third Order
0
0.05
0.1
0.15
0.2
Strains

# MoNbTiV

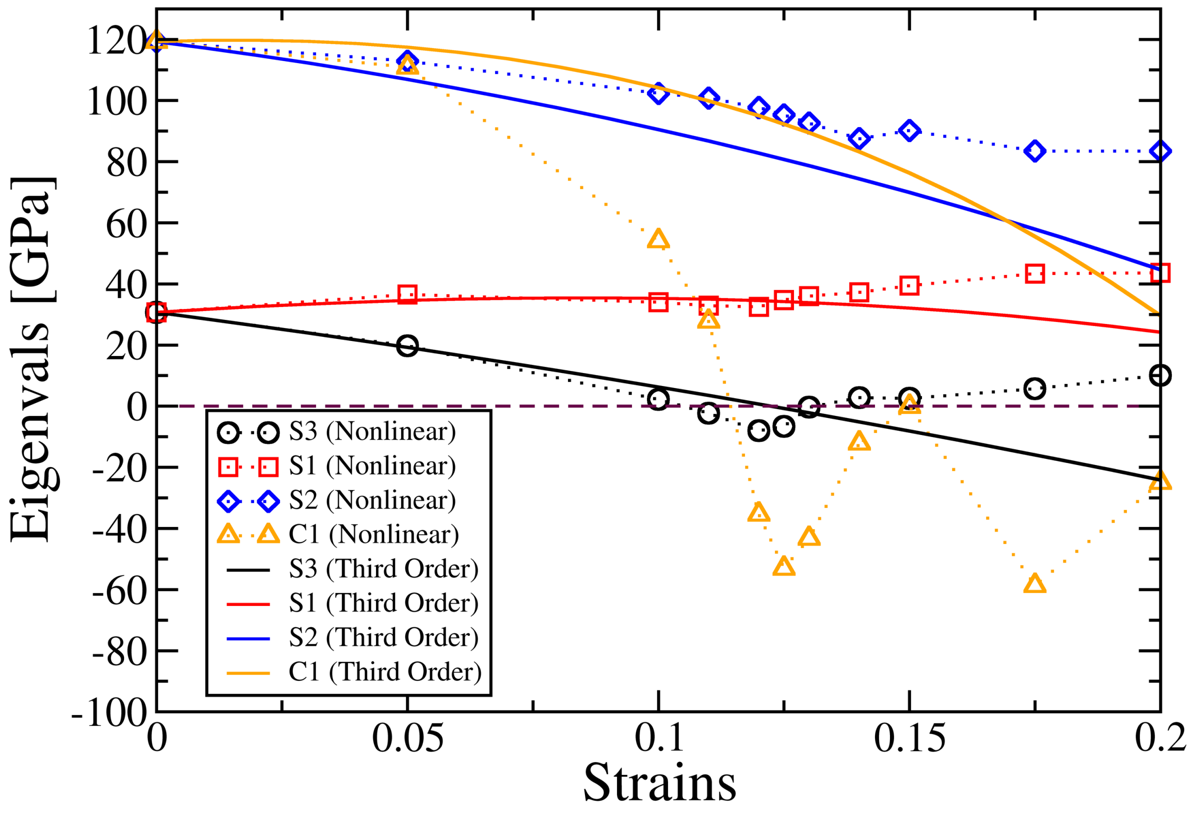

Eigenvals [GPa]
Strains
S3 (Nonlinear)
S1 (Nonlinear)
S2 (Nonlinear)
C1 (Nonlinear)
S3 (Third Order)
S1 (Third Order)
S2 (Third Order)
C1 (Third Order)


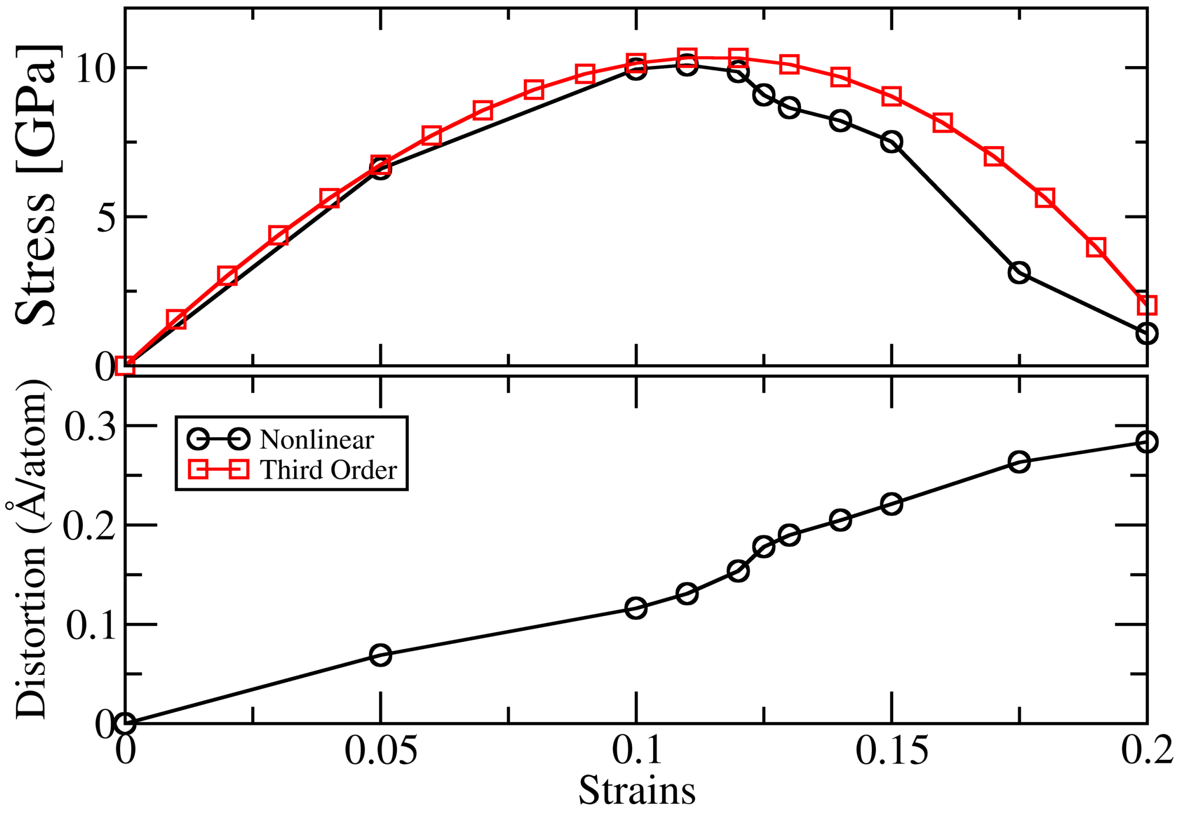

Stress [GPa]
Distortion (Å/atom)
Strains
Nonlinear
Third Order

# MoNbTiW

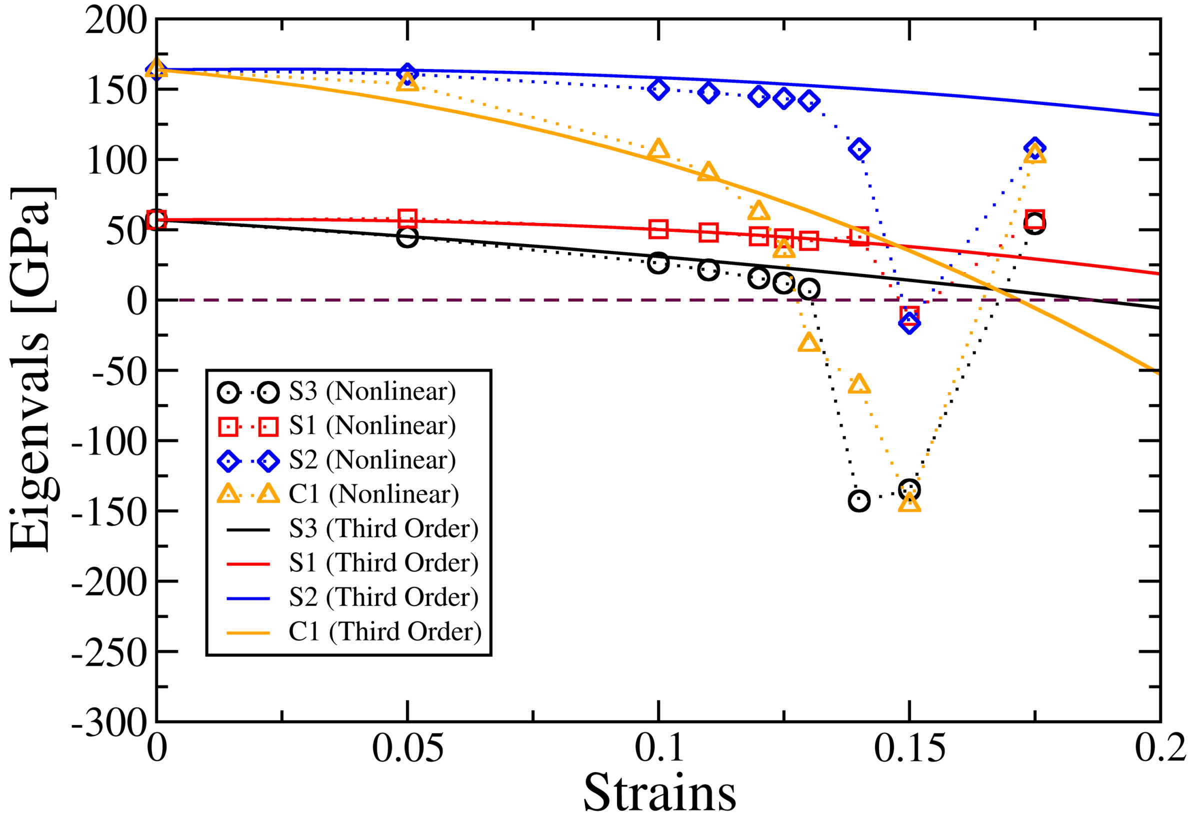
Eigenvals [GPa]
Strains
200
150
100
50
0
-50
-100
-150
-200
-250
-300
0
0.05
0.1
0.15
0.2
S3 (Nonlinear)
S1 (Nonlinear)
S2 (Nonlinear)
C1 (Nonlinear)
S3 (Third Order)
S1 (Third Order)
S2 (Third Order)
C1 (Third Order)

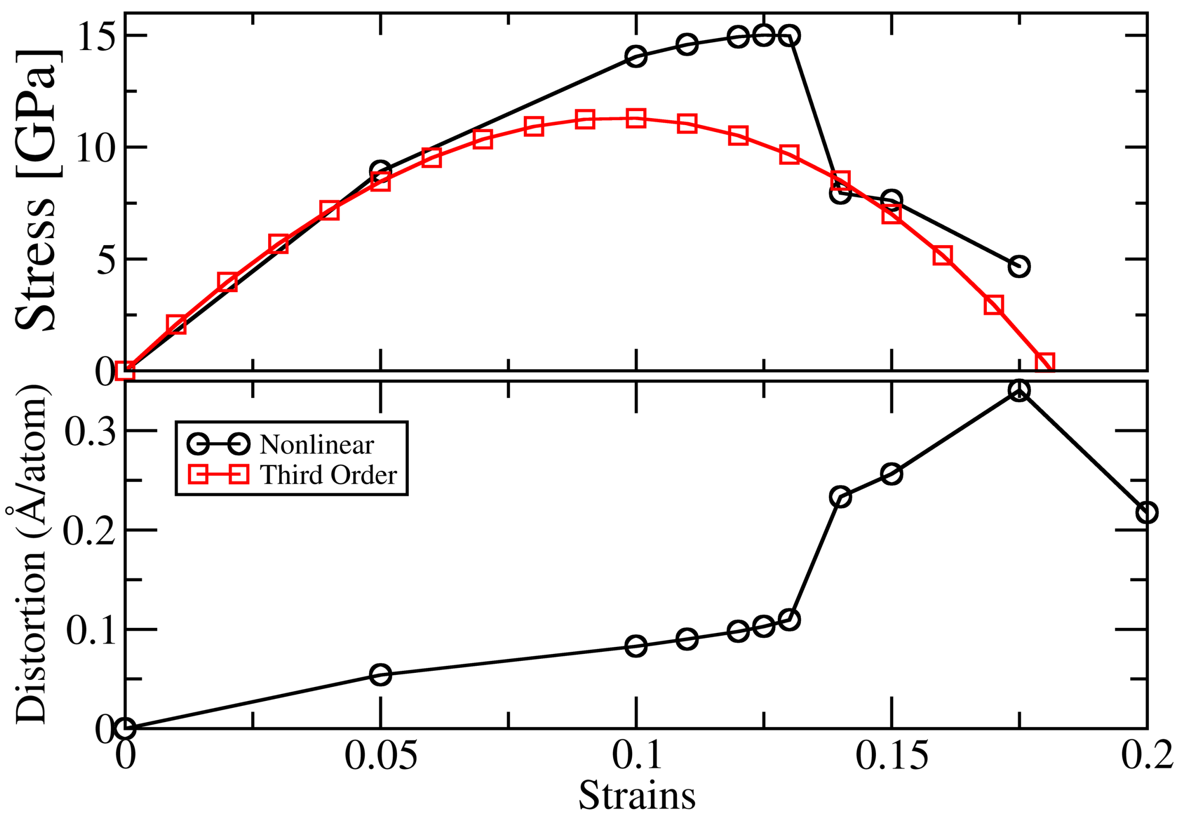
Stress [GPa]
15
10
5
0
Distortion (Å/atom)
0.3
0.2
0.1
0
Nonlinear
Third Order
0
0.05
0.1
0.15
0.2
Strains

# MoNbTiZr

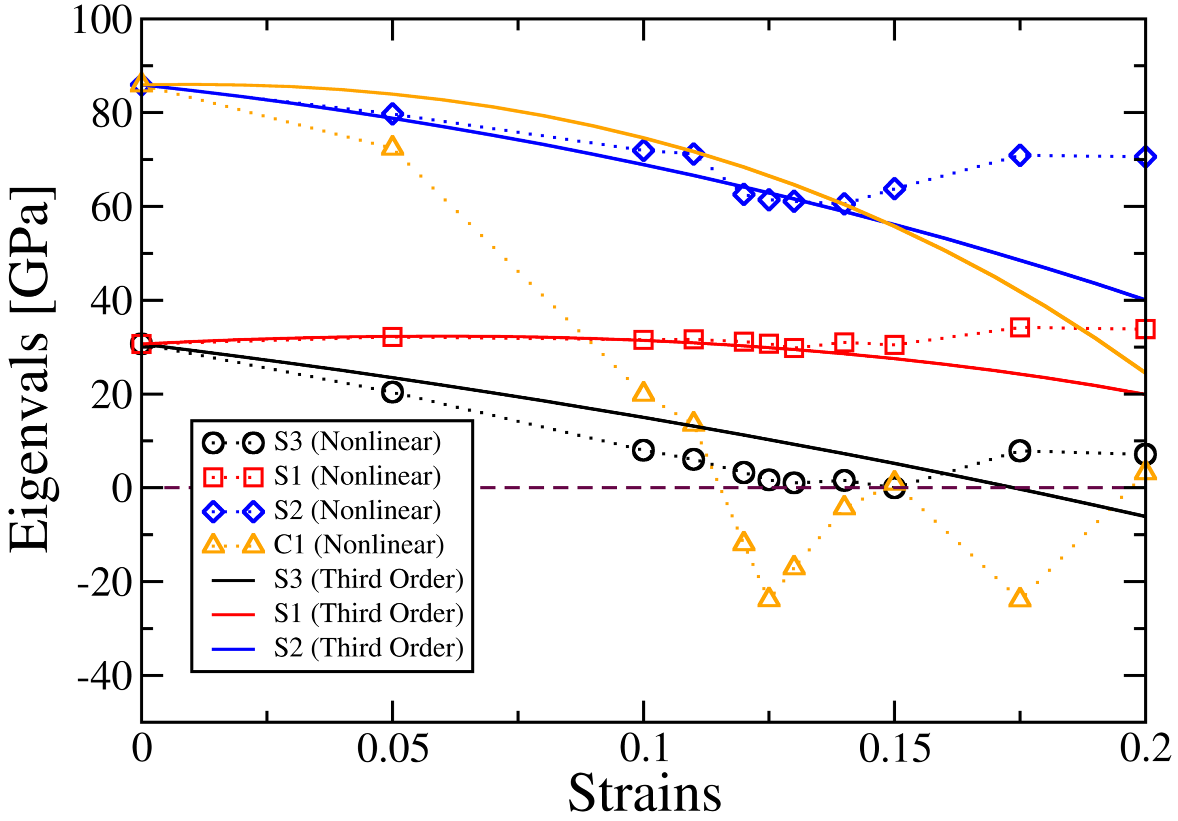

Eigenvals [GPa]
Strains
100
80
60
40
20
0
-20
-40
0
0.05
0.1
0.15
0.2
S3 (Nonlinear)
S1 (Nonlinear)
S2 (Nonlinear)
C1 (Nonlinear)
S3 (Third Order)
S1 (Third Order)
S2 (Third Order)


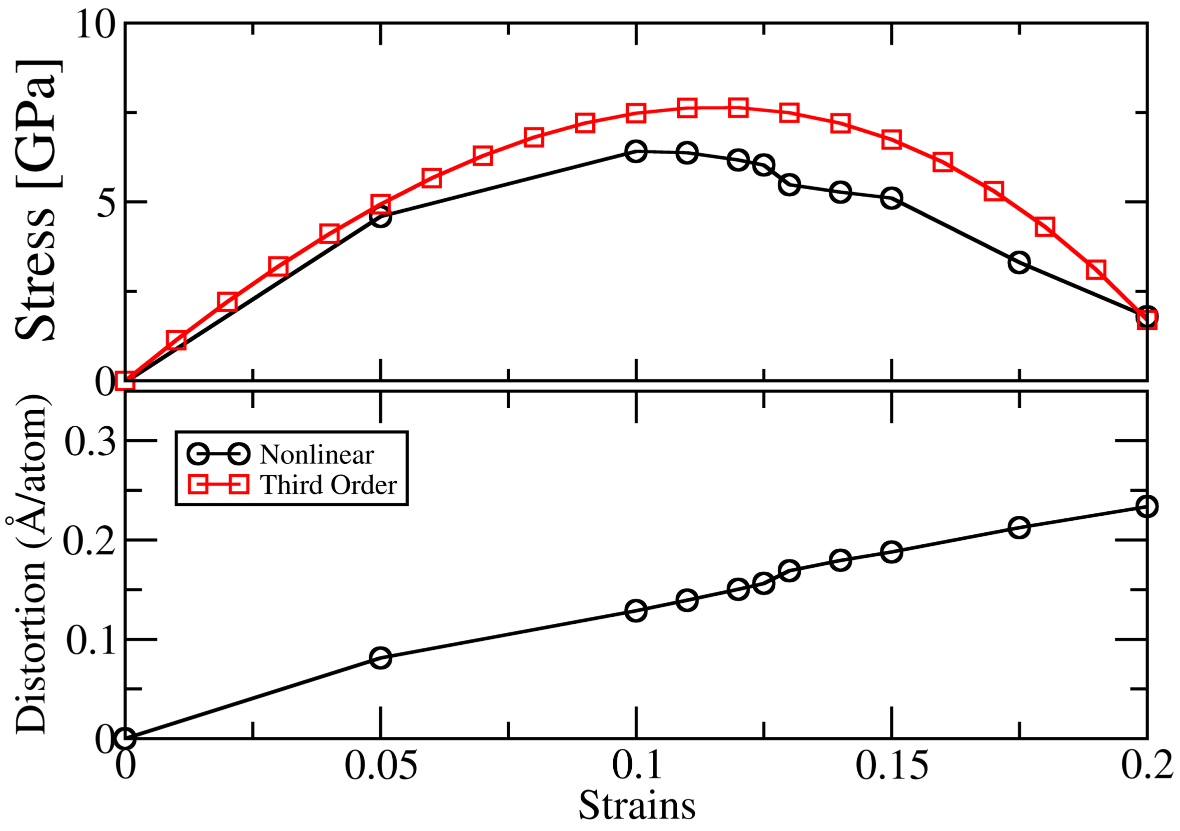

Stress [GPa]
10
5
0
Distortion (Å/atom)
0.3
0.2
0.1
0
Nonlinear
Third Order
0
0.05
0.1
0.15
0.2
Strains

# MoNbTaW

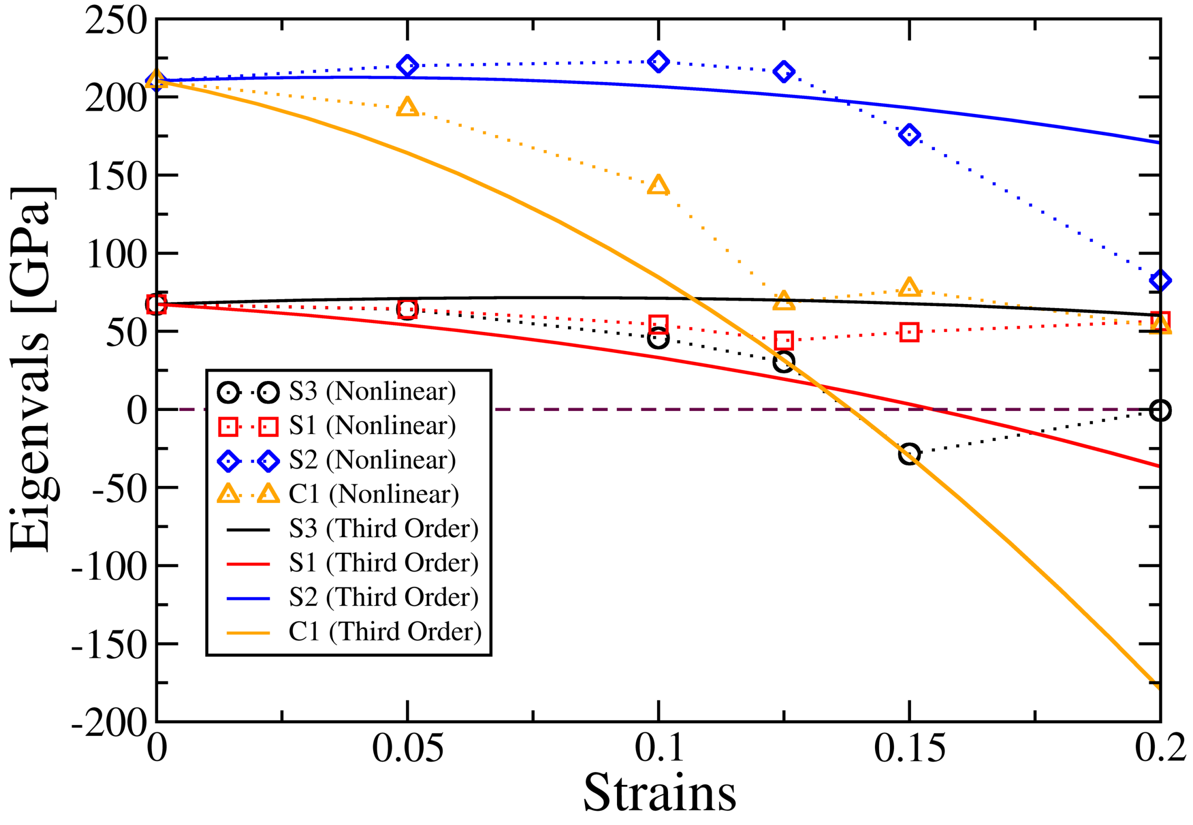

Eigenvals [GPa]
Strains
S3 (Nonlinear)
S1 (Nonlinear)
S2 (Nonlinear)
C1 (Nonlinear)
S3 (Third Order)
S1 (Third Order)
S2 (Third Order)
C1 (Third Order)
250
200
150
100
50
0
-50
-100
-150
-200
0
0.05
0.1
0.15
0.2


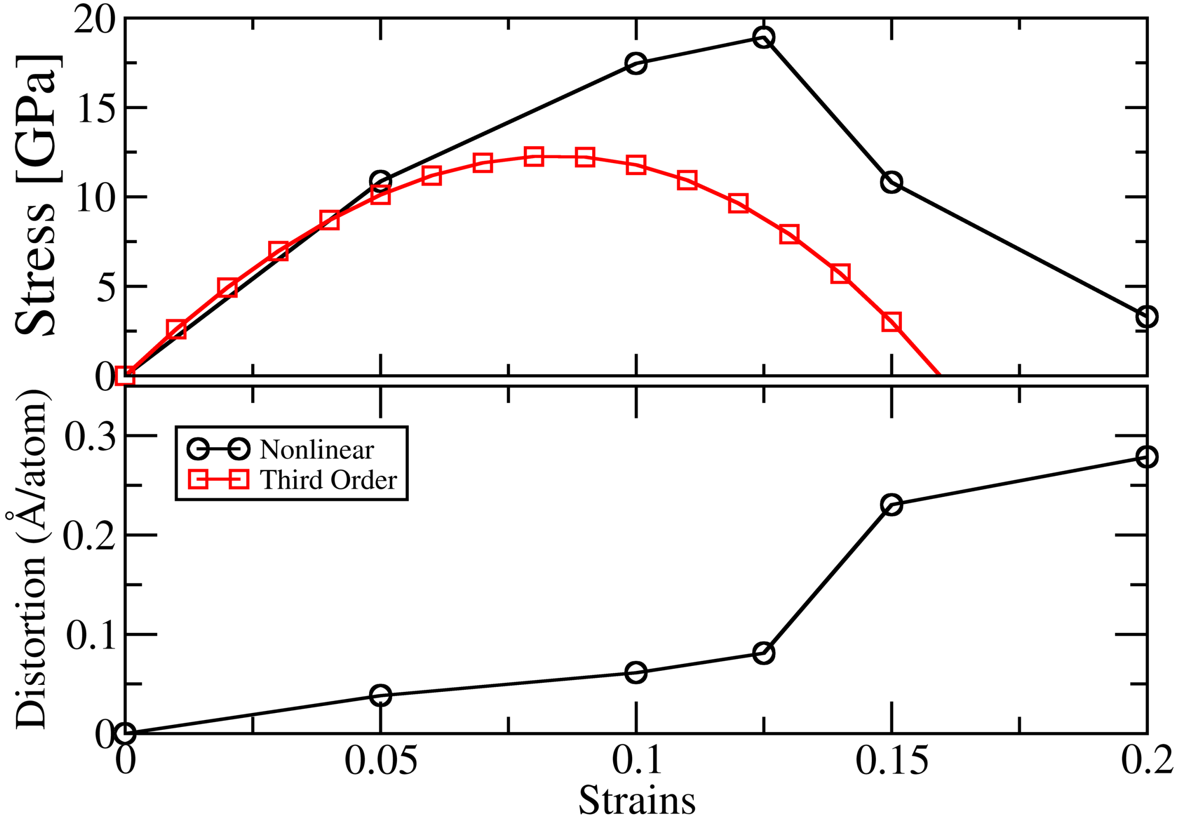

Stress [GPa]
Distortion (Å/atom)
Strains
Nonlinear
Third Order
20
15
10
5
0
0.3
0.2
0.1
0
0
0.05
0.1
0.15
0.2

# NbTaVW

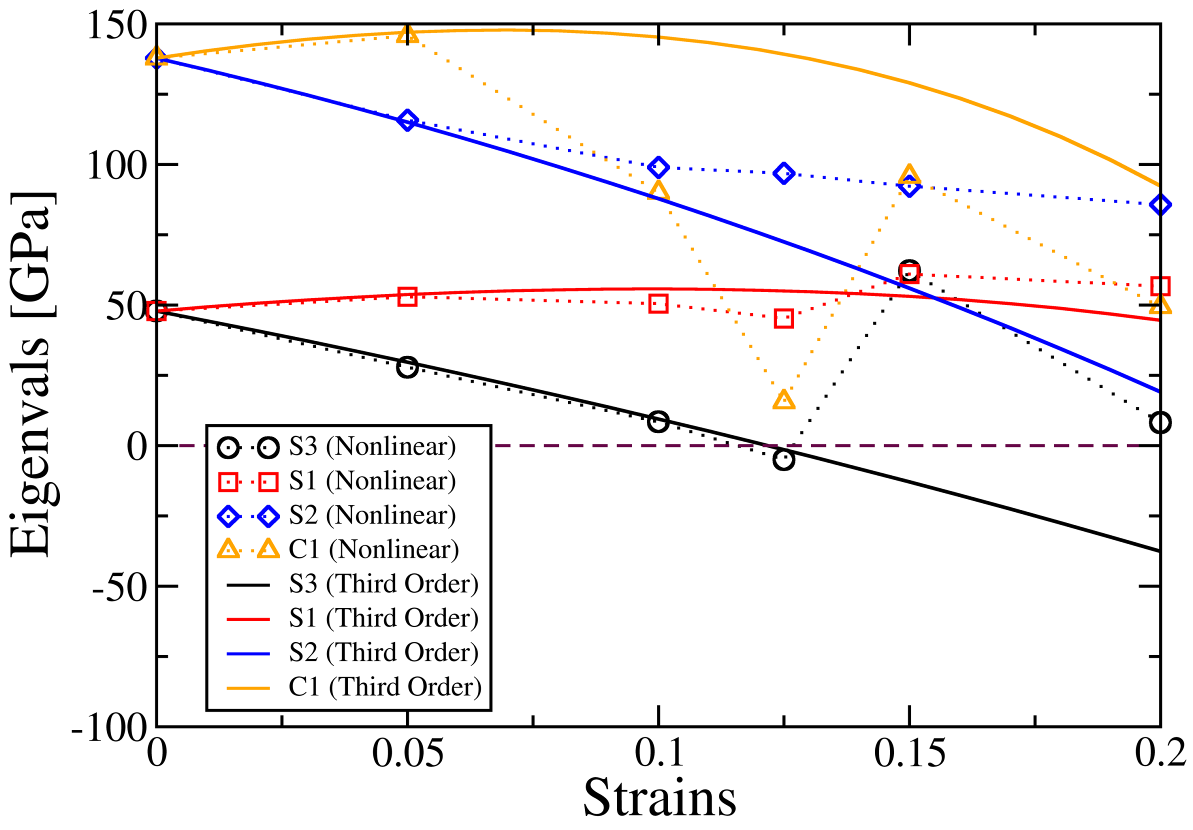

Eigenvals [GPa]
150
100
50
0
-50
-100
0
0.05
0.1
0.15
0.2
Strains
S3 (Nonlinear)
S1 (Nonlinear)
S2 (Nonlinear)
C1 (Nonlinear)
S3 (Third Order)
S1 (Third Order)
S2 (Third Order)
C1 (Third Order)


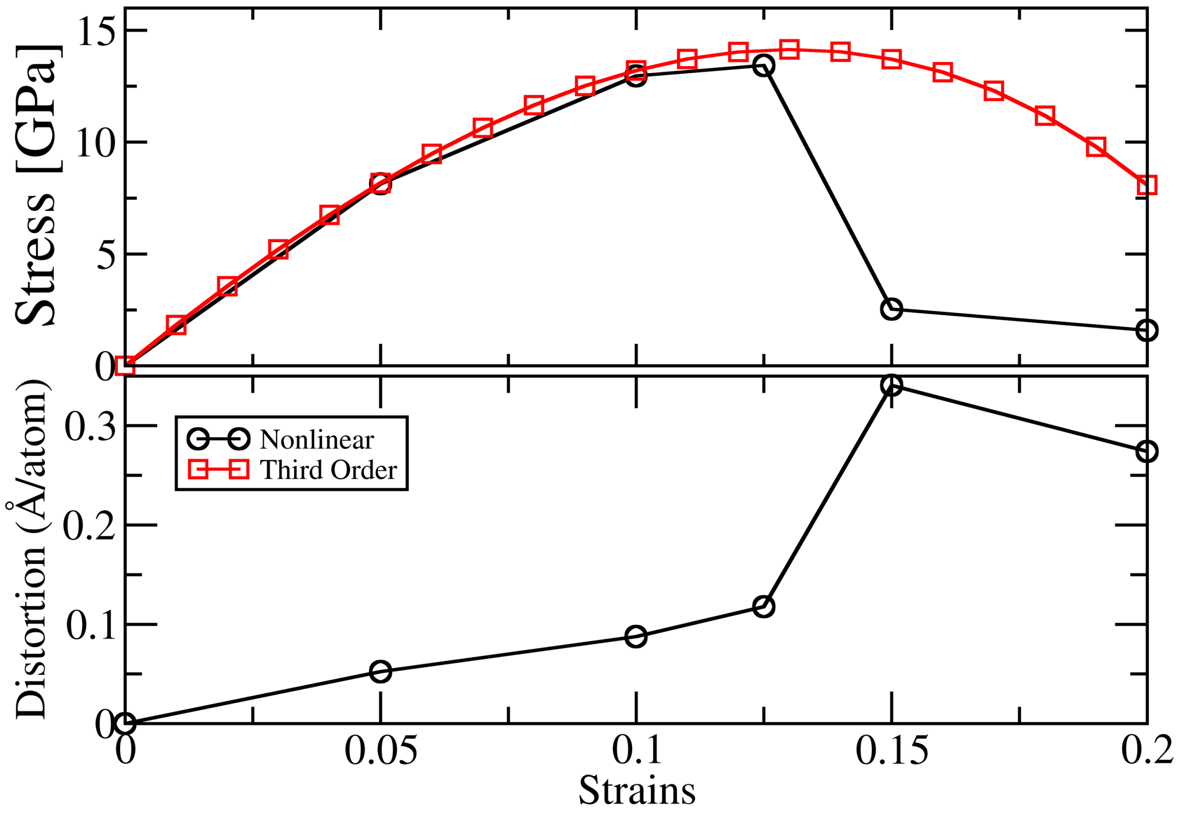

Stress [GPa]
15
10
5
0
Distortion (Å/atom)
0.3
0.2
0.1
0
Nonlinear
Third Order
0
0.05
0.1
0.15
0.2
Strains

# NbTaTiV

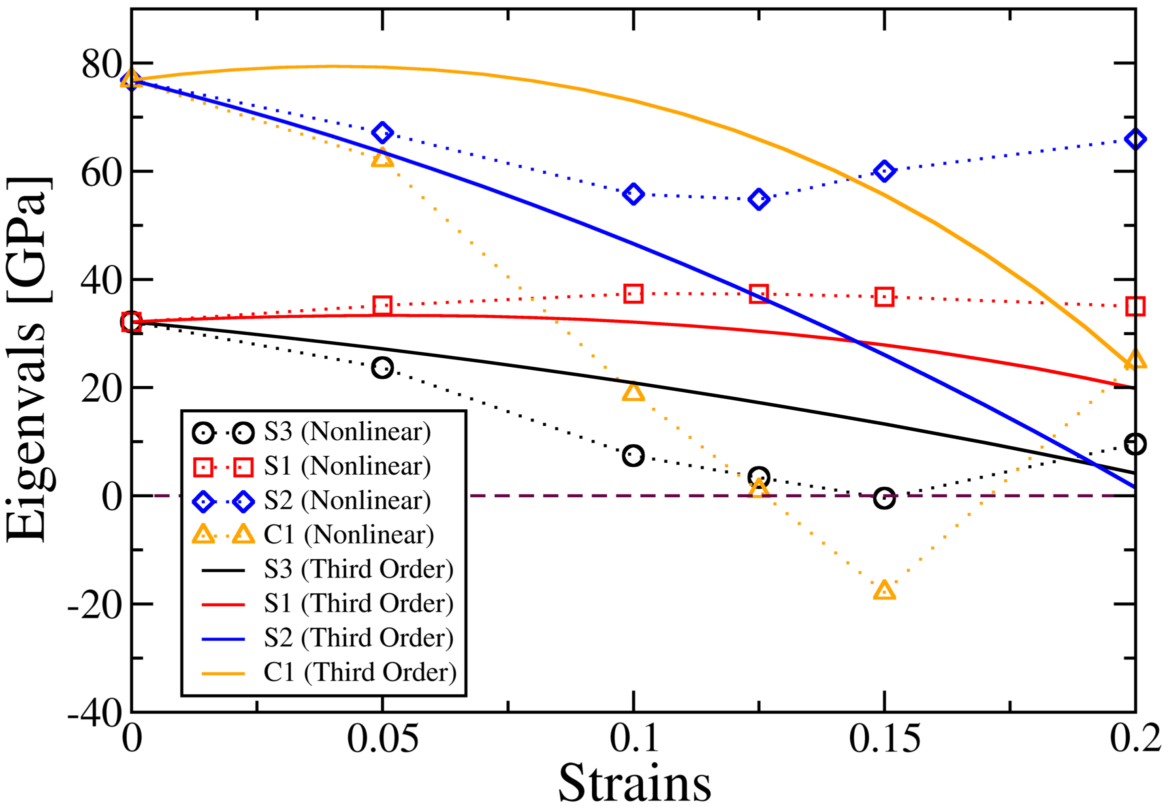

Eigenvals [GPa]
Strains
S3 (Nonlinear)
S1 (Nonlinear)
S2 (Nonlinear)
C1 (Nonlinear)
S3 (Third Order)
S1 (Third Order)
S2 (Third Order)
C1 (Third Order)


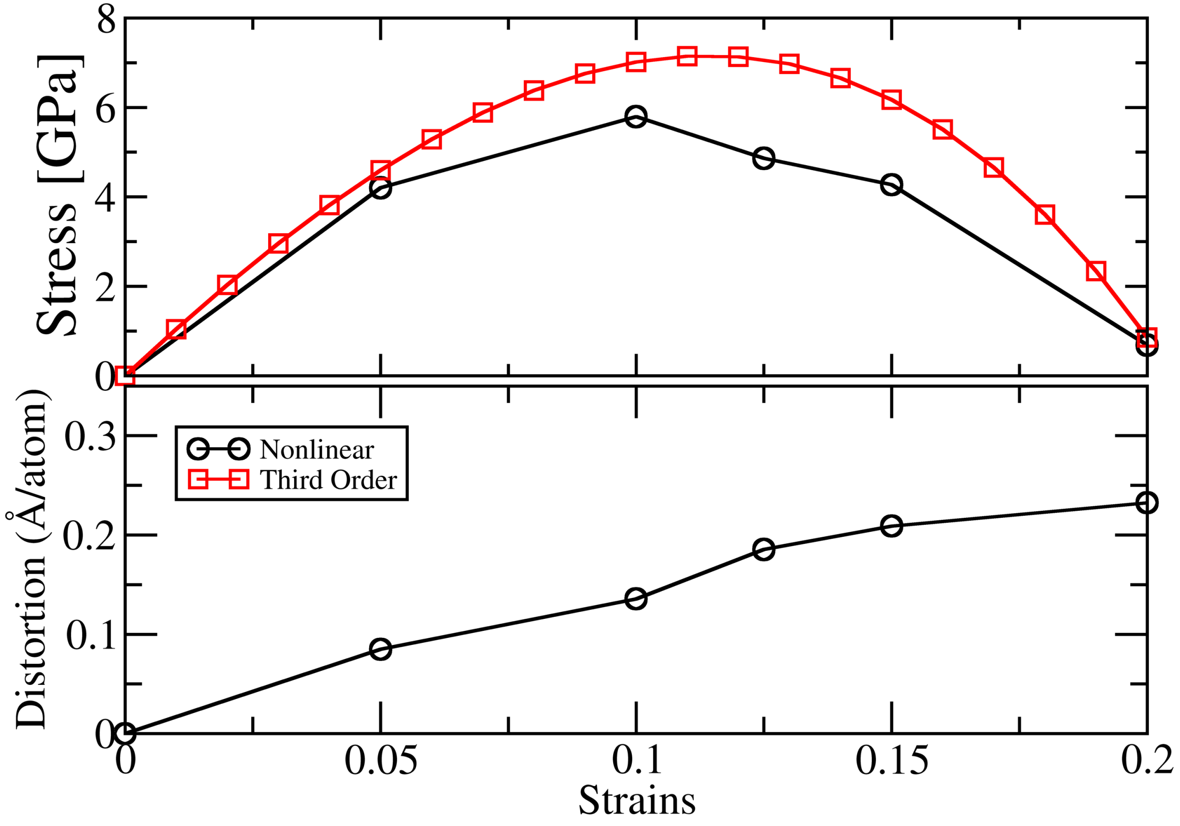

Stress [GPa]
Distortion (Å/atom)
Strains
Nonlinear
Third Order
